# Supplementary material for: Refined dual stable Grothendieck polynomials and generalized Bender-Knuth involutions
Source: arXiv:1509.03803 ancillary file (2015-10-14)
Supplement: Supplementary file 1 [file groth1alt.pdf]

# Refined dual stable Grothendieck polynomials and generalized Bender-Knuth involutions

Pavel Galashin, Darij Grinberg, and Gaku Liu

alternative version\*, October 13, 2015

The dual stable Grothendieck polynomials are a deformation of the Schur functions, originating in the study of the  $K$ -theory of the Grassmannian. We generalize these polynomials by introducing a countable family of additional parameters, and we prove that this generalization still defines symmetric functions. For this fact, we give two self-contained proofs, one of which constructs a family of involutions on the set of reverse plane partitions generalizing the Bender-Knuth involutions on semistandard tableaux, whereas the other classifies the structure of reverse plane partitions with entries 1 and 2.

## 1. Introduction

Thomas Lam and Pavlo Pylyavskyy, in [LamPyl07, §9.1], (and earlier Mark Shimozono and Mike Zabrocki in unpublished work of 2003) studied *dual stable Grothendieck polynomials*, a deformation (in a sense) of the Schur functions. Let us briefly recount their definition.<sup>1</sup>

Let  $\lambda/\mu$  be a skew partition. The Schur function  $s_{\lambda/\mu}$  is a multivariate generating function for the semistandard tableaux of shape  $\lambda/\mu$ . In the same vein,

---

\*This version of the paper is the closest to its original (written back in January 2015). It has the most details and contains an explicit statement and proof of the diamond lemma, as well as an application thereof which was omitted from the later versions of the paper.

<sup>1</sup>All definitions that will be made in this introduction are provisional. Every notion that will be used in the paper is going to be defined in more detail and precision in one of the sections below; thus, a reader not already familiar with Schur functions and partitions should start reading from Section 2 on.

the dual stable Grothendieck polynomial<sup>2</sup>  $g_{\lambda/\mu}$  is a generating function for the reverse plane partitions of shape  $\lambda/\mu$ ; these, unlike semistandard tableaux, are only required to have their entries increase *weakly* down columns (and along rows). More precisely,  $g_{\lambda/\mu}$  is a formal power series in countably many commuting indeterminates  $x_1, x_2, x_3, \dots$  (over an arbitrary commutative ring  $\mathbf{k}$ ) defined by

$$g_{\lambda/\mu} = \sum_{\substack{T \text{ is a reverse plane} \\ \text{partition of shape } \lambda/\mu}} \mathbf{x}^{\text{ircont}(T)},$$

where  $\mathbf{x}^{\text{ircont}(T)}$  is the monomial  $x_1^{a_1} x_2^{a_2} x_3^{a_3} \dots$  whose  $i$ -th exponent  $a_i$  is the number of columns of  $T$  containing the entry  $i$ . As proven in [LamPyl07, §9.1], this power series  $g_{\lambda/\mu}$  is a symmetric function (albeit, unlike  $s_{\lambda/\mu}$ , an inhomogeneous one in general). Lam and Pylyavskyy connect the  $g_{\lambda/\mu}$  to the (more familiar) *stable Grothendieck polynomials*  $G_{\lambda/\mu}$  (via a duality between the symmetric functions and their completion, which explains the name of the  $g_{\lambda/\mu}$ ; see [LamPyl07, §9.4]) and to the  $K$ -theory of Grassmannians ([LamPyl07, §9.5]).

We devise a common generalization of the dual stable Grothendieck polynomial  $g_{\lambda/\mu}$  and the classical skew Schur function  $s_{\lambda/\mu}$ . Namely, if  $t_1, t_2, t_3, \dots$  are countably many fixed elements of the base ring  $\mathbf{k}$  (e.g., polynomial indeterminates, or integers), then we set

$$\tilde{g}_{\lambda/\mu} = \sum_{\substack{T \text{ is a reverse plane} \\ \text{partition of shape } \lambda/\mu}} \mathbf{t}^{\text{ceq}(T)} \mathbf{x}^{\text{ircont}(T)},$$

where  $\mathbf{t}^{\text{ceq}(T)}$  is the product  $t_1^{b_1} t_2^{b_2} t_3^{b_3} \dots$  whose  $i$ -th exponent  $b_i$  is the number of cells in the  $i$ -th row of  $T$  whose entry equals the entry of their neighbor cell directly below them. This  $\tilde{g}_{\lambda/\mu}$  becomes  $g_{\lambda/\mu}$  when all the  $t_i$  are set to 1, and becomes  $s_{\lambda/\mu}$  when all the  $t_i$  are set to 0; but keeping the  $t_i$  arbitrary offers infinitely many degrees of freedom which are so far unexplored. Our main result, Theorem 3.3, states that  $\tilde{g}_{\lambda/\mu}$  is a symmetric function (in the  $x_1, x_2, x_3, \dots$ ).

We prove this result (thus obtaining a new proof of [LamPyl07, Theorem 9.1]) first using an elaborate generalization of the classical Bender-Knuth involutions to reverse plane partitions; these generalized involutions are constructed using a form of the *diamond lemma* (Lemma 4.1). Then, we prove it for a second time by analyzing the structure of reverse plane partitions whose entries lie in  $\{1, 2\}$ . The second proof reflects back on the first, in particular providing an alternative definition of the generalized Bender-Knuth involutions constructed in the first proof, and showing that these involutions are (in a sense) “the only reasonable choice”.

The present paper is organized as follows: In Section 2, we recall classical definitions and introduce notations pertaining to combinatorics and symmetric

---

<sup>2</sup>The word “polynomial” is a stretch:  $g_{\lambda/\mu}$  is a bounded-degree power series in infinitely many indeterminates (like  $s_{\lambda/\mu}$ ).

functions. In Section 3, we define the refined dual stable Grothendieck polynomials  $\tilde{g}_{\lambda/\mu}$ , state our main result (that they are symmetric functions), and do the first steps of its proof (by reducing it to a purely combinatorial statement about the existence of an involution with certain properties). In Section 4, we state and (for the sake of completeness) prove the version of the diamond lemma we need, and we digress to give an elementary application of it that serves to demonstrate its use. In Section 5, we prove our main result by constructing the required involution using the diamond lemma. In Section 6, we recapitulate the definition of the classical Bender-Knuth involution, and sketch the proof that our involution is a generalization of the latter. Finally, in Section 7 we study the structure of reverse plane partitions with entries belonging to  $\{1, 2\}$ , which (in particular) gives us an explicit formula for the  $\mathbf{t}$ -coefficients of  $\tilde{g}_{\lambda/\mu}(x_1, x_2, 0, 0, \dots; \mathbf{t})$ , and shines a new light on the involution constructed in Section 5 (also showing that it is the unique involution that shares certain natural properties with the classical Bender-Knuth involutions).

## 1.1. Acknowledgments

We owe our familiarity with dual stable Grothendieck polynomials to Richard Stanley. We thank Alexander Postnikov for providing context and motivation, and Thomas Lam and Pavlo Pylyavskyy for interesting conversations.

## 2. Notations and definitions

Let us begin by defining our notations (including some standard conventions from algebraic combinatorics).

### 2.1. Partitions and tableaux

We set  $\mathbb{N} = \{0, 1, 2, \dots\}$  and  $\mathbb{N}_+ = \{1, 2, 3, \dots\}$ . A *weak composition* will mean a sequence  $(\alpha_1, \alpha_2, \alpha_3, \dots) \in \mathbb{N}^{\mathbb{N}_+}$  of nonnegative integers such that all but finitely many  $i \in \mathbb{N}_+$  satisfy  $\alpha_i = 0$ . Given a weak composition  $\alpha = (\alpha_1, \alpha_2, \alpha_3, \dots)$ , we denote the sum  $\alpha_1 + \alpha_2 + \alpha_3 + \dots$  (which is finite and an element of  $\mathbb{N}$ ) by  $|\alpha|$  and call it the *size* of  $\alpha$ . Given a weak composition  $\alpha$  and a positive integer  $i$ , we let  $\alpha_i$  denote the  $i$ -th entry of  $\alpha$  (so that every weak composition  $\alpha$  automatically satisfies  $\alpha = (\alpha_1, \alpha_2, \alpha_3, \dots)$ ).

A *partition* means a weak composition  $(\alpha_1, \alpha_2, \alpha_3, \dots)$  satisfying  $\alpha_1 \geq \alpha_2 \geq \alpha_3 \geq \dots$ . We identify every partition  $(\alpha_1, \alpha_2, \alpha_3, \dots)$  with the (truncated) sequence  $(\alpha_1, \alpha_2, \dots, \alpha_m)$  whenever  $m$  is a nonnegative integer such that  $\alpha_{m+1} = \alpha_{m+2} = \alpha_{m+3} = \dots = 0$ . In particular, the partition  $(0, 0, 0, \dots)$  is thus identified with the empty sequence  $()$  (but also, for example, with  $(0, 0, 0)$ ). We denote the latter partition by  $\emptyset$ , and call it the *empty partition*.

We let  $\text{Par}$  denote the set of all partitions.

The *Young diagram*<sup>3</sup> of a partition  $\lambda$  is defined to be the subset  $\{(i, j) \in \mathbb{N}_+^2 \mid j \leq \lambda_i\}$  of  $\mathbb{N}_+^2$ . It is denoted by  $Y(\lambda)$ , and has size  $|Y(\lambda)| = \lambda_1 + \lambda_2 + \lambda_3 + \cdots = |\lambda|$ .

We draw every subset of  $\mathbb{N}_+^2$  (for example, the Young diagram of a partition) as a set of boxes in the plane, according to the following convention (known as the *English notation*, or also as the *matrix notation*): We imagine an infinite table, whose rows are labelled  $1, 2, 3, \dots$  (from left to right) and whose columns are labelled  $1, 2, 3, \dots$  as well (from top to bottom). We represent every element  $(i, j)$  of  $\mathbb{N}_+^2$  as a box in this table – namely, as the box at the intersection of row  $i$  with column  $j$ . In order to draw a subset  $Z$  of  $\mathbb{N}_+^2$ , we simply chart (the borders of) the boxes corresponding to all the  $(i, j) \in Z$ . For instance, the Young diagram of the partition  $(4, 2, 1)$  is the subset  $\{(1, 1), (1, 2), (1, 3), (1, 4), (2, 1), (2, 2), (3, 1)\}$  of  $\mathbb{N}_+^2$ , and we draw it as

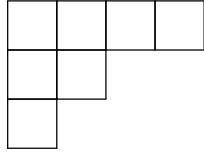

(since we draw them as boxes in the plane). (Our convention for drawing Young diagrams is identical with that in [Fulton97] and in [GriRei15].)

If  $\mu$  and  $\lambda$  are two partitions, then we say that  $\mu \subseteq \lambda$  if and only if every  $i \in \mathbb{N}_+$  satisfies  $\mu_i \leq \lambda_i$ . Equivalently,  $\mu \subseteq \lambda$  if and only if  $Y(\mu) \subseteq Y(\lambda)$ . This defines a partial order  $\subseteq$  on the set  $\text{Par}$  of all partitions. A *skew partition* shall denote a pair  $(\mu, \lambda)$  of two partitions  $\mu$  and  $\lambda$  satisfying  $\mu \subseteq \lambda$ ; this pair will also be denoted by  $\lambda/\mu$ . Given a skew partition  $\lambda/\mu$ , we define the (*skew*) *Young diagram*  $Y(\lambda/\mu)$  of this skew partition to be the subset  $Y(\lambda) \setminus Y(\mu)$  of  $\mathbb{N}_+^2$ . Again, this Young diagram is drawn as above; for instance, the Young diagram of  $(4, 3, 1) / (2, 1)$  is

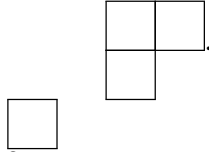

A subset  $Z$  of  $\mathbb{N}_+^2$  is said to be *convex* if it has the following property: If  $(i, j) \in Z$ ,  $(i', j') \in \mathbb{N}_+^2$  and  $(i'', j'') \in Z$  are such that  $i \leq i' \leq i''$  and  $j \leq j' \leq j''$ , then

$$(i', j') \in Z. \quad (1)$$

It is clear that the Young diagram  $Y(\lambda/\mu)$  is convex whenever  $\lambda/\mu$  is a skew partition. It is easy to show that, conversely, every finite convex subset of  $\mathbb{N}_+^2$  has the form  $Y(\lambda/\mu)$  for some skew partition  $\lambda/\mu$ .

If  $Z$  is a subset of  $\mathbb{N}_+^2$  (for instance, a Young diagram), then a *filling* of  $Z$  means a map  $T : Z \rightarrow \mathbb{N}_+$ . Such a filling can be visually represented by drawing the elements of  $Z$  as boxes (following the convention above) and, for every  $c \in Z$ ,

inserting the value  $T(c)$  into the box corresponding to  $c$ . For instance,

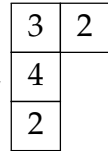

<sup>3</sup>also known as the *Ferrers diagram*

one possible filling of  $Y((2, 1, 1))$ ; formally speaking, it is the map  $Y((2, 1, 1)) \rightarrow \mathbb{N}_+$  which sends  $(1, 1)$ ,  $(1, 2)$ ,  $(2, 1)$  and  $(3, 1)$  to 3, 2, 4 and 2, respectively. When  $T$  is a filling of  $Z$  and when  $c$  is a cell in  $Z$ , we refer to the integer  $T(c) \in \mathbb{N}_+$  as the *entry* of  $T$  in the cell  $c$ . For varying  $c$ , these integers are called the *entries* of  $T$ .

Given a finite convex subset  $Z$  of  $\mathbb{N}_+^2$ , we define a *reverse plane partition of shape  $Z$*  to be a filling  $T : Z \rightarrow \mathbb{N}_+^2$  of  $Z$  satisfying the following two requirements:

- The entries of  $T$  are *weakly increasing along rows* (speaking in terms of the picture). In more precise terms: If  $(i, j)$  and  $(i, j')$  are two elements of  $Z$  such that  $j < j'$ , then  $T(i, j) \leq T(i, j')$ .
- The entries of  $T$  are *weakly increasing down columns*. In more precise terms: If  $(i, j)$  and  $(i', j)$  are two elements of  $Z$  such that  $i < i'$ , then  $T(i, j) \leq T(i', j)$ .

Generally, a *reverse plane partition* is defined to be a map which is a reverse plane partition of shape  $Z$  for some finite convex subset  $Z$  of  $\mathbb{N}_+^2$ . Notice that  $Z$  is uniquely determined by the map (in fact, it is the domain of the map).

We shall abbreviate the term “reverse plane partition” as “*rpp*”. For instance,

|   |   |   |
|---|---|---|
|   | 3 | 3 |
| 2 | 3 |   |
| 3 | 4 |   |

 is an rpp of shape  $Y((3, 2, 2) / (1))$ .

A well-known class of rpps are the *semistandard tableaux* (also known as column-strict tableaux). To define this class, it is enough to change “weakly increasing down columns” into “strictly increasing down columns” (and, correspondingly, change “ $T(i, j) \leq T(i', j)$ ” into “ $T(i, j) < T(i', j)$ ”) in the above definition of an

rpp. For instance,
 

|   |   |   |
|---|---|---|
|   | 3 | 3 |
| 2 | 3 |   |
| 3 | 4 |   |

 is not a semistandard tableau due to having two 3’s

in its second column, but
 

|   |   |   |
|---|---|---|
|   | 3 | 3 |
| 2 | 4 |   |
| 3 | 7 |   |

 is a semistandard tableau. Semistandard

tableaux have been studied for decades; an exposition of their properties and applications can be found in Fulton’s [Fulton97].

**Remark 2.1.** Let  $\lambda/\mu$  be a skew partition. What we call a semistandard tableau of shape  $Y(\lambda/\mu)$  is usually called a *semistandard tableau of shape  $\lambda/\mu$* . (However, unlike the “semistandard tableaux” defined by some other authors, our semistandard tableaux of shape  $Y(\lambda/\mu)$  do not “store” the skew partition  $\lambda/\mu$  as part of their data.)

## 2.2. Symmetric functions

We now come to the algebraic part of our definitions.

We let  $\mathbf{k}$  be an arbitrary commutative ring with unity.<sup>4</sup> We consider the ring  $\mathbf{k}[[x_1, x_2, x_3, \dots]]$  of formal power series in countably many indeterminates  $x_1, x_2, x_3, \dots$ . Given a weak composition  $\alpha$ , we let  $\mathbf{x}^\alpha$  be the monomial  $x_1^{\alpha_1} x_2^{\alpha_2} x_3^{\alpha_3} \dots$ .

A formal power series  $f \in \mathbf{k}[[x_1, x_2, x_3, \dots]]$  is said to be *bounded-degree* if there exists an  $N \in \mathbb{N}$  such that every monomial  $\mathbf{x}^\alpha$  which occurs (with nonzero coefficient) in  $f$  satisfies  $|\alpha| \leq N$ . (Notice that  $|\alpha|$  is the degree of  $\mathbf{x}^\alpha$ .) The set of all bounded-degree power series in  $\mathbf{k}[[x_1, x_2, x_3, \dots]]$  is a  $\mathbf{k}$ -subalgebra of  $\mathbf{k}[[x_1, x_2, x_3, \dots]]$ , and will be denoted by  $\mathbf{k}[[x_1, x_2, x_3, \dots]]_{\text{bdd}}$ .

We let  $\mathfrak{S}_{(\infty)}$  denote the group of all permutations  $\pi$  of the set  $\mathbb{N}_+$  such that all but finitely many  $i \in \mathbb{N}_+$  satisfy  $\pi(i) = i$ . This is a subgroup of the group  $\mathfrak{S}_\infty$  of *all* permutations of  $\mathbb{N}_+$ . The group  $\mathfrak{S}_{(\infty)}$  is generated by the subset  $\{s_1, s_2, s_3, \dots\}$ , where each  $s_i$  is the transposition  $(i, i+1)$ .<sup>5</sup> The group  $\mathfrak{S}_\infty$  (and thus, also its subgroup  $\mathfrak{S}_{(\infty)}$ ) acts on the set of all weak compositions by the rule

$$\begin{aligned} \pi \cdot (\alpha_1, \alpha_2, \alpha_3, \dots) &= (\alpha_{\pi^{-1}(1)}, \alpha_{\pi^{-1}(2)}, \alpha_{\pi^{-1}(3)}, \dots) \\ &\text{for every } \pi \in \mathfrak{S}_\infty \text{ and} \\ &\text{every weak composition } (\alpha_1, \alpha_2, \alpha_3, \dots). \end{aligned}$$

A formal power series  $f \in \mathbf{k}[[x_1, x_2, x_3, \dots]]$  is said to be *symmetric* if it has the following property: Whenever  $\alpha$  and  $\beta$  are two weak compositions in the same  $\mathfrak{S}_{(\infty)}$ -orbit, the coefficients of  $f$  before  $\mathbf{x}^\alpha$  and before  $\mathbf{x}^\beta$  are equal.<sup>6</sup>

The *symmetric functions* over  $\mathbf{k}$  are defined to be the symmetric bounded-degree power series  $f \in \mathbf{k}[[x_1, x_2, x_3, \dots]]$ . They form a  $\mathbf{k}$ -subalgebra of  $\mathbf{k}[[x_1, x_2, x_3, \dots]]$ . This  $\mathbf{k}$ -subalgebra is called the *ring of symmetric functions over  $\mathbf{k}$* ; it will be denoted by  $\Lambda$  or (when  $\mathbf{k}$  is not clear from the context) by  $\Lambda_{\mathbf{k}}$ . (The reader shall be warned that [LamPyl07] denotes this  $\mathbf{k}$ -algebra by  $\text{Sym}$ , while using the notation  $\Lambda$  for the set which we call  $\text{Par}$ .) Symmetric functions are a classical field of research, and are closely related to Young diagrams and tableaux; see [Stan99, Chapter 7], [Macdon95] and [GriRei15, Chapter 2] for expositions.

Another equivalent way to define the notion of symmetric functions is the following: The group  $\mathfrak{S}_\infty$  acts  $\mathbf{k}$ -linearly and continuously on the  $\mathbf{k}$ -module  $\mathbf{k}[[x_1, x_2, x_3, \dots]]$  by the rule

$$\pi \mathbf{x}^\alpha = \mathbf{x}^{\pi \cdot \alpha} \quad \text{for every } \pi \in \mathfrak{S}_\infty \text{ and every weak composition } \alpha.$$

<sup>4</sup>Many authors, such as those of [LamPyl07], set  $\mathbf{k} = \mathbb{Z}$ .

<sup>5</sup>To prove this result, it is enough to notice that the finite symmetric groups  $\mathfrak{S}_n$  for all  $n \in \mathbb{N}$  can be canonically embedded into  $\mathfrak{S}_{(\infty)}$ , and  $\mathfrak{S}_{(\infty)}$  becomes their direct limit.

<sup>6</sup>Notice that this definition does not change if  $\mathfrak{S}_{(\infty)}$  is replaced by  $\mathfrak{S}_\infty$ . But it is customary (and useful to our purposes) to define it using  $\mathfrak{S}_{(\infty)}$ .

The subgroup  $\mathfrak{S}_{(\infty)}$  of  $\mathfrak{S}_{\infty}$  thus also acts on  $\mathbf{k}[[x_1, x_2, x_3, \dots]]$  by restriction. Both  $\mathfrak{S}_{\infty}$  and  $\mathfrak{S}_{(\infty)}$  preserve the  $\mathbf{k}$ -submodule  $\mathbf{k}[[x_1, x_2, x_3, \dots]]_{\text{bdd}}$ , and thus act on  $\mathbf{k}[[x_1, x_2, x_3, \dots]]_{\text{bdd}}$  as well. Now,

$$\Lambda = (\mathbf{k}[[x_1, x_2, x_3, \dots]]_{\text{bdd}})^{\mathfrak{S}_{\infty}} = (\mathbf{k}[[x_1, x_2, x_3, \dots]]_{\text{bdd}})^{\mathfrak{S}_{(\infty)}}.$$

### 2.3. Schur functions

Given a subset  $Z$  of  $\mathbb{N}_+^2$  and a filling  $T$  of  $Z$ , we define a weak composition  $\text{cont}(T)$  by setting

$$(\text{cont}(T))_i = |T^{-1}(i)| = (\text{the number of entries of } T \text{ equal to } i) \\ \text{for every } i \in \mathbb{N}_+.$$

We call  $\text{cont}(T)$  the *content* of  $T$ . Notice that  $\mathbf{x}^{\text{cont}(T)} = \prod_{c \in Z} x_{T(c)}$ .

Given a skew partition  $\lambda/\mu$ , we define the *Schur function*  $s_{\lambda/\mu}$  to be the formal power series  $\sum_{\substack{T \text{ is a semistandard} \\ \text{tableau of shape } Y(\lambda/\mu)}} \mathbf{x}^{\text{cont}(T)}$ . A nontrivial property of these Schur functions is that they are symmetric:

**Proposition 2.2.** We have  $s_{\lambda/\mu} \in \Lambda$  for every skew partition  $\lambda/\mu$ .

This result appears, e.g., in [Stan99, Theorem 7.10.2] and [GriRei15, Proposition 2.11]; it is commonly proven bijectively using the so-called *Bender-Knuth involutions*. We shall recall the definitions of these involutions in Section 6.

One might attempt to replace “semistandard tableau” by “rpp” in the definition of a Schur function. However, the resulting power series are (in general) no longer symmetric (for instance,  $\sum_{\substack{T \text{ is an rpp} \\ \text{of shape } Y((2,1))}} \mathbf{x}^{\text{cont}(T)} \notin \Lambda$ ). Nevertheless, Lam

and Pylyavskyy [LamPyl07, §9] have noticed that it is possible to define symmetric functions from rpps, albeit it requires replacing the content  $\text{cont}(T)$  by a subtler construction. Let us now discuss their definition.

### 2.4. Dual stable Grothendieck polynomials

If  $Z$  is a convex subset of  $\mathbb{N}_+^2$ , if  $T$  is a filling of  $Z$ , and if  $k \in \mathbb{N}_+$ , then:

- The *k-th column* of  $T$  will mean the sequence of all entries of  $T$  in cells of the form  $(i, k)$  with  $i \in \mathbb{N}_+$  (in the order of increasing  $i$ ).
- The *k-th row* of  $T$  will mean the sequence of all entries of  $T$  in cells of the form  $(k, i)$  with  $i \in \mathbb{N}_+$  (in the order of increasing  $i$ ).

Notice that (due to  $Z$  being convex) there are no “gaps” in these rows and columns: If  $Z$  is a convex subset of  $\mathbb{N}_+^2$ , and if  $k \in \mathbb{N}_+$ , then the positive integers  $i$  satisfying  $(i, k) \in Z$  form a (possibly empty) interval, and so do the positive integers  $i$  satisfying  $(k, i) \in Z$ .

If  $Z$  is a convex subset of  $\mathbb{N}_+^2$ , and if  $T$  is a filling of  $Z$ , then we define a weak composition  $\text{ircont}(T)$  by setting

$$(\text{ircont}(T))_i = (\text{the number of } k \in \mathbb{N}_+ \text{ such that the } k\text{-th column of } T \text{ contains } i) \\ \text{for every } i \in \mathbb{N}_+.$$

(In more colloquial terms,  $(\text{ircont}(T))_i$  is the number of columns of  $T$  which contain  $i$ .) We refer to  $\text{ircont}(T)$  as the *irredundant content* of  $T$ . For instance, if

$$T = \begin{array}{|c|c|} \hline & 3 \\ \hline 2 & 3 \\ \hline 3 & 4 \\ \hline \end{array}, \text{ then } \text{ircont}(T) = (0, 1, 3, 1, 0, 0, 0, \dots) \text{ (since 1 is contained in 0}$$

columns of  $T$ , while 2 is contained in 1 column, 3 in 3 columns, etc.).

Notice that

$$\text{ircont}(T) = \text{cont}(T) \quad \text{if } T \text{ is a semistandard tableau.} \quad (2)$$

Indeed, (2) follows by noticing that in every given column of a semistandard tableau, every positive integer occurs at most once.

For the rest of this section, we fix a skew partition  $\lambda/\mu$ . Now, the *dual stable Grothendieck polynomial*  $g_{\lambda/\mu}$  is defined to be the formal power series

$$\sum_{\substack{T \text{ is an rpp} \\ \text{of shape } Y(\lambda/\mu)}} \mathbf{x}^{\text{ircont}(T)}.$$

It is easy to see that  $g_{\lambda/\mu}$  is a well-defined formal power series (i.e., the infinite sum  $\sum_{\substack{T \text{ is an rpp} \\ \text{of shape } Y(\lambda/\mu)}} \mathbf{x}^{\text{ircont}(T)}$  converges in the usual topology on the ring

$\mathbf{k}[[x_1, x_2, x_3, \dots]]$ ).<sup>7</sup> Unlike the Schur function  $s_{\lambda/\mu}$ , it is (in general) not homogeneous, because whenever a column of an rpp  $T$  contains an entry several times, the corresponding monomial  $\mathbf{x}^{\text{ircont}(T)}$  “counts” this entry only once. It is fairly clear that the highest-degree homogeneous component of  $g_{\lambda/\mu}$  is  $s_{\lambda/\mu}$  (the component of degree  $|\lambda| - |\mu|$ ). Therefore,  $g_{\lambda/\mu}$  can be regarded as an inhomogeneous deformation of the Schur function  $s_{\lambda/\mu}$ .

Lam and Pylyavskyy, in [LamPy107, §9.1], have shown the following fact:

<sup>7</sup>Be warned that  $g_{\lambda/\mu}$  is (despite its name) not a polynomial (barring trivial cases).



■ **Proposition 2.3.** We have  $g_{\lambda/\mu} \in \Lambda$  for every skew partition  $\lambda/\mu$ .

They prove this proposition using generalized plactic algebras [FomGre06, Lemma 3.1] (and also give a second, combinatorial proof for the case  $\mu = \emptyset$  by explicitly expanding  $g_{\lambda/\emptyset}$  as a sum of Schur functions).

In the next section, we shall introduce a refinement of these  $g_{\lambda/\mu}$ , and later we will reprove Proposition 2.3 in a self-contained and elementary way.

### 3. Refined dual stable Grothendieck polynomials

#### 3.1. Definition

We fix arbitrary elements  $t_1, t_2, t_3, \dots$  of  $\mathbf{k}$ . (For instance,  $\mathbf{k}$  can be a polynomial ring in infinitely many variables over another ring  $\mathbf{m}$ , and  $t_1, t_2, t_3, \dots$  can then be these variables.) For every weak composition  $\alpha$ , we set  $\mathbf{t}^\alpha = t_1^{\alpha_1} t_2^{\alpha_2} t_3^{\alpha_3} \cdots \in \mathbf{k}$ .

If  $Z$  is a subset of  $\mathbb{N}_+^2$ , and if  $T$  is a filling of  $Z$ , then a *redundant cell* of  $T$  will mean a cell  $(i, j)$  of  $Z$  such that  $(i+1, j)$  is also a cell of  $Z$  and satisfies  $T(i, j) = T(i+1, j)$ . Notice that a semistandard tableau is the same thing as an rpp which has no redundant cells<sup>8</sup>.

If  $Z$  is a subset of  $\mathbb{N}_+^2$ , and if  $T$  is a filling of  $Z$ , then we define a weak composition  $\text{ceq}(T)$  by

$$(\text{ceq}(T))_i = (\text{the number of } j \in \mathbb{N}_+ \text{ such that } (i, j) \text{ is a redundant cell of } T) \quad (3)$$

for every  $i \in \mathbb{N}_+$ .

(Visually speaking,  $(\text{ceq}(T))_i$  is the number of columns of  $T$  whose entry in the  $i$ -th row equals their entry in the  $(i+1)$ -th row.) We call  $\text{ceq}(T)$  the *column-equalities counter* of  $T$ . Notice that

$$|\text{ceq}(T)| = (\text{the number of all redundant cells of } T) \quad (4)$$

for every rpp  $T$ . For instance, if  $T = \begin{array}{|c|c|} \hline & 3 & 3 \\ \hline 2 & 3 & \\ \hline 3 & 4 & \\ \hline \end{array}$ , then  $\text{ceq}(T) = (1, 0, 0, 0, \dots)$

(since the 1-st and 2-nd rows of  $T$  have equal entries in one column, while for every  $i > 1$ , the  $i$ -th and  $(i+1)$ -th rows of  $T$  do not have equal entries in any column).

<sup>8</sup>*Proof.* Recall that the difference between a semistandard tableau and an rpp is that the entries of a semistandard tableau have to be strictly increasing down columns, whereas the entries of an rpp have to be merely weakly increasing down columns. Thus, a semistandard tableau is the same thing as an rpp whose every column has no adjacent equal entries. In other words, a semistandard tableau is the same thing as an rpp which has no redundant cells (because having two adjacent equal entries in a column is tantamount to having a redundant cell).

Let now  $\lambda/\mu$  be a skew partition. We set

$$\tilde{g}_{\lambda/\mu} = \sum_{\substack{T \text{ is an rpp} \\ \text{of shape } Y(\lambda/\mu)}} \mathbf{t}^{\text{ceq}(T)} \mathbf{x}^{\text{ircont}(T)}.$$

This  $\tilde{g}_{\lambda/\mu}$  is a well-defined formal power series in  $\mathbf{k}[[x_1, x_2, x_3, \dots]]$ <sup>9</sup>, and moreover belongs to  $\mathbf{k}[[x_1, x_2, x_3, \dots]]_{\text{bdd}}$  (since  $|\text{ircont}(T)| \leq |Y(\lambda/\mu)| = |\lambda| - |\mu|$  for every rpp  $T$  of shape  $Y(\lambda/\mu)$ ).

Let us give some examples of  $\tilde{g}_{\lambda/\mu}$ .

**Example 3.1. (a)** Let  $n \in \mathbb{N}$ , let  $\lambda = (n)$  and let  $\mu = \emptyset$ . Then, the rpps  $T$  of shape  $Y(\lambda/\mu)$  have the form  $\begin{bmatrix} a_1 & a_2 & \cdots & a_n \end{bmatrix}$  with  $a_1 \leq a_2 \leq \cdots \leq a_n$ . Each such rpp  $T$  satisfies  $\text{ceq}(T) = \emptyset$  and  $\mathbf{x}^{\text{ircont}(T)} = x_{a_1} x_{a_2} \cdots x_{a_n}$ . Thus, the definition of  $\tilde{g}_{\lambda/\mu}$  yields

$$\begin{aligned} \tilde{g}_{\lambda/\mu} &= \sum_{\substack{T \text{ is an rpp} \\ \text{of shape } Y(\lambda/\mu)}} \mathbf{t}^{\text{ceq}(T)} \mathbf{x}^{\text{ircont}(T)} = \sum_{a_1 \leq a_2 \leq \cdots \leq a_n} \underbrace{\mathbf{t}^{\emptyset}}_{=1} x_{a_1} x_{a_2} \cdots x_{a_n} \\ &= \sum_{a_1 \leq a_2 \leq \cdots \leq a_n} x_{a_1} x_{a_2} \cdots x_{a_n}. \end{aligned}$$

This is the so-called  $n$ -th complete homogeneous symmetric function  $h_n$ .

**(b)** Let now  $n \in \mathbb{N}$ , let  $\lambda = \underbrace{(1, 1, \dots, 1)}_{n \text{ times}}$  and let  $\mu = \emptyset$ . Then, the rpps

$T$  of shape  $Y(\lambda/\mu)$  have the form  $\begin{bmatrix} a_1 \\ a_2 \\ \vdots \\ a_n \end{bmatrix}$  with  $a_1 \leq a_2 \leq \cdots \leq a_n$ . Each such

rpp  $T$  satisfies  $\mathbf{t}^{\text{ceq}(T)} = \prod_{\substack{i \in \{1, 2, \dots, n\}; \\ a_i = a_{i+1}}} t_i$  and  $\mathbf{x}^{\text{ircont}(T)} = \prod_{\substack{i \in \{1, 2, \dots, n\}; \\ a_i < a_{i+1}}} x_i$ , where we

set  $a_{n+1} = \infty$  in order to simplify our notations. Thus, the definition of  $\tilde{g}_{\lambda/\mu}$

<sup>9</sup>*Proof.* We need to show that the infinite sum  $\sum_{\substack{T \text{ is an rpp} \\ \text{of shape } Y(\lambda/\mu)}} \mathbf{t}^{\text{ceq}(T)} \mathbf{x}^{\text{ircont}(T)}$  converges with re-

spect to the standard topology on  $\mathbf{k}[[x_1, x_2, x_3, \dots]]$ . In other words, we need to show that every monomial  $\mathbf{x}^\alpha$  occurs only finitely often in this sum. But this is fairly clear: Given a monomial  $\mathbf{x}^\alpha$ , there exist only finitely many  $i \in \mathbb{N}_+$  satisfying  $\alpha_i > 0$ . These finitely many  $i$  are the only entries that can occur in an rpp  $T$  of shape  $Y(\lambda/\mu)$  which satisfies  $\text{ircont}(T) = \alpha$ . Hence, there are only finitely many such rpps. This means that there are only finitely many terms in the sum  $\sum_{\substack{T \text{ is an rpp} \\ \text{of shape } Y(\lambda/\mu)}} \mathbf{t}^{\text{ceq}(T)} \mathbf{x}^{\text{ircont}(T)}$  in which the monomial  $\mathbf{x}^\alpha$  occurs, qed.

yields

$$\begin{aligned}\tilde{g}_{\lambda/\mu} &= \sum_{\substack{T \text{ is an rpp} \\ \text{of shape } Y(\lambda/\mu)}} \mathbf{t}^{\text{ceq}(T)} \mathbf{x}^{\text{ircont}(T)} = \sum_{a_1 \leq a_2 \leq \dots \leq a_n} \left( \prod_{\substack{i \in \{1,2,\dots,n\}; \\ a_i = a_{i+1}}} t_i \right) \left( \prod_{\substack{i \in \{1,2,\dots,n\}; \\ a_i < a_{i+1}}} x_i \right) \\ &= \sum_{k=0}^n e_k(t_1, t_2, \dots, t_{n-1}) e_{n-k}(x_1, x_2, x_3, \dots),\end{aligned}$$

where  $e_i(\xi_1, \xi_2, \xi_3, \dots)$  denotes the  $i$ -th elementary symmetric function in the indeterminates  $\xi_1, \xi_2, \xi_3, \dots$ . It is possible to rewrite this as

$$\tilde{g}_{\lambda/\mu} = e_n(t_1, t_2, \dots, t_{n-1}, x_1, x_2, x_3, \dots).$$

(c) Let now  $n = 3$ , let  $\lambda = (2, 1)$  and let  $\mu = \emptyset$ . Then, the rpps  $T$  of shape  $Y(\lambda/\mu)$  have the form 

|     |     |
|-----|-----|
| $a$ | $b$ |
| $c$ |     |

 with  $a \leq b$  and  $a \leq c$ . Each such rpp  $T$  satisfies

$$\mathbf{t}^{\text{ceq}(T)} = \begin{cases} 1, & \text{if } a < c; \\ t_1, & \text{if } a = c \end{cases} \text{ and } \mathbf{x}^{\text{ircont}(T)} = \begin{cases} x_a x_b x_c, & \text{if } a < c; \\ x_a x_b, & \text{if } a = c \end{cases}. \text{ Thus,}$$

$$\begin{aligned}\tilde{g}_{\lambda/\mu} &= \sum_{\substack{T \text{ is an rpp} \\ \text{of shape } Y(\lambda/\mu)}} \mathbf{t}^{\text{ceq}(T)} \mathbf{x}^{\text{ircont}(T)} = \sum_{a \leq b; a \leq c} \begin{cases} 1, & \text{if } a < c; \\ t_1, & \text{if } a = c \end{cases} \begin{cases} x_a x_b x_c, & \text{if } a < c; \\ x_a x_b, & \text{if } a = c \end{cases} \\ &= \sum_{a \leq b; a < c} x_a x_b x_c + t_1 \sum_{a \leq b} x_a x_b.\end{aligned}$$

The power series  $\tilde{g}_{\lambda/\mu}$  generalize the power series  $g_{\lambda/\mu}$  and  $s_{\lambda/\mu}$  studied before:

**Proposition 3.2.** Let  $\lambda/\mu$  be a skew partition.

(a) If  $(t_1, t_2, t_3, \dots) = (1, 1, 1, \dots)$ , then  $\tilde{g}_{\lambda/\mu} = g_{\lambda/\mu}$ .

(b) If  $(t_1, t_2, t_3, \dots) = (0, 0, 0, \dots)$ , then  $\tilde{g}_{\lambda/\mu} = s_{\lambda/\mu}$ .

*Proof of Proposition 3.2.* (a) Let  $(t_1, t_2, t_3, \dots) = (1, 1, 1, \dots)$ . Then,  $\mathbf{t}^\alpha = 1$  for every weak composition  $\alpha$ . Thus,  $\mathbf{t}^{\text{ceq}(T)} = 1$  for every rpp  $T$ . Now, the definition of  $\tilde{g}_{\lambda/\mu}$  yields  $\tilde{g}_{\lambda/\mu} = \sum_{\substack{T \text{ is an rpp} \\ \text{of shape } Y(\lambda/\mu)}} \underbrace{\mathbf{t}^{\text{ceq}(T)}}_{=1} \mathbf{x}^{\text{ircont}(T)} = \sum_{\substack{T \text{ is an rpp} \\ \text{of shape } Y(\lambda/\mu)}} \mathbf{x}^{\text{ircont}(T)} = g_{\lambda/\mu}$ .

This proves Proposition 3.2 (a).

(b) Let  $(t_1, t_2, t_3, \dots) = (0, 0, 0, \dots)$ . Then, if  $T$  is an rpp which has at least one redundant cell, then  $\mathbf{t}^{\text{ceq}(T)} = 0$  (because  $\text{ceq}(T)$  has at least one nonzero entry in this case). Therefore, the sum  $\sum_{\substack{T \text{ is an rpp} \\ \text{of shape } Y(\lambda/\mu)}} \mathbf{t}^{\text{ceq}(T)} \mathbf{x}^{\text{ircont}(T)}$  does not change if

we discard all addends for which  $T$  has at least one redundant cell. Thus,

$$\begin{aligned} \sum_{\substack{T \text{ is an rpp} \\ \text{of shape } Y(\lambda/\mu)}} \mathbf{t}^{\text{ceq}(T)} \mathbf{x}^{\text{ircont}(T)} &= \sum_{\substack{T \text{ is an rpp} \\ \text{of shape } Y(\lambda/\mu); \\ T \text{ has no redundant cells}}} \mathbf{t}^{\text{ceq}(T)} \mathbf{x}^{\text{ircont}(T)} \\ &= \sum_{\substack{T \text{ is a semistandard} \\ \text{tableau of shape } Y(\lambda/\mu)}} \mathbf{t}^{\text{ceq}(T)} \mathbf{x}^{\text{ircont}(T)} \end{aligned}$$

(since a semistandard tableau of shape  $Y(\lambda/\mu)$  is the same thing as an rpp of shape  $Y(\lambda/\mu)$  which has no redundant cells). Now, the definition of  $\tilde{g}_{\lambda/\mu}$  yields

$$\begin{aligned} \tilde{g}_{\lambda/\mu} &= \sum_{\substack{T \text{ is an rpp} \\ \text{of shape } Y(\lambda/\mu)}} \mathbf{t}^{\text{ceq}(T)} \mathbf{x}^{\text{ircont}(T)} = \sum_{\substack{T \text{ is a semistandard} \\ \text{tableau of shape } Y(\lambda/\mu)}} \underbrace{\mathbf{t}^{\text{ceq}(T)}}_{=1 \text{ (since } \text{ceq}(T)=\emptyset)} \underbrace{\mathbf{x}^{\text{ircont}(T)}}_{=\mathbf{x}^{\text{cont}(T)} \text{ (by (2))}} \\ &= \sum_{\substack{T \text{ is a semistandard} \\ \text{tableau of shape } Y(\lambda/\mu)}} \mathbf{x}^{\text{cont}(T)} = s_{\lambda/\mu}. \end{aligned}$$

□

### 3.2. The symmetry statement

Our main result is now the following:

**Theorem 3.3.** Let  $\lambda/\mu$  be a skew partition. Then,  $\tilde{g}_{\lambda/\mu} \in \Lambda$ .

It is clear that Proposition 2.2 and Proposition 2.3 are particular cases of Theorem 3.3 (due to Proposition 3.2).

We shall prove Theorem 3.3 bijectively. The core of our proof will be the following fact:

**Theorem 3.4.** Let  $\lambda/\mu$  be a skew partition. Let  $i \in \mathbb{N}_+$ . Let  $\text{RPP}(\lambda/\mu)$  denote the set of all rpps of shape  $Y(\lambda/\mu)$ . Then, there exists an involution  $\mathbf{B}_i : \text{RPP}(\lambda/\mu) \rightarrow \text{RPP}(\lambda/\mu)$  which has the following property: For every  $T \in \text{RPP}(\lambda/\mu)$ , we have

$$\text{ceq}(\mathbf{B}_i(T)) = \text{ceq}(T) \quad (5)$$

and

$$\text{ircont}(\mathbf{B}_i(T)) = s_i \cdot \text{ircont}(T). \quad (6)$$

<sup>10</sup> (Here,  $s_i \cdot \text{ircont}(T)$  means the result of the transposition  $s_i = (i, i+1) \in \mathfrak{S}_{(\infty)}$  acting on the weak composition  $\text{ircont}(T)$ .)

This involution  $\mathbf{B}_i$  is a generalization of the  $i$ -th Bender-Knuth involution defined for semistandard tableaux (see, e.g., [GriRei15, proof of Proposition 2.11]),

<sup>10</sup>We notice that the equality (6) says the following:

but its definition is more complicated than that of the latter.<sup>11</sup> Defining it and proving its properties will take a significant part of this paper.

Let us first see how Theorem 3.4 implies Theorem 3.3:

*Proof of Theorem 3.3 using Theorem 3.4.* We know that  $\tilde{g}_{\lambda/\mu} \in \mathbf{k}[[x_1, x_2, x_3, \dots]]_{\text{bdd}}$ . Hence, in order to prove that  $\tilde{g}_{\lambda/\mu} \in \Lambda$ , it is enough to prove that  $\tilde{g}_{\lambda/\mu}$  is invariant under the action of  $\mathfrak{S}_{(\infty)}$  (since  $\Lambda = (\mathbf{k}[[x_1, x_2, x_3, \dots]]_{\text{bdd}})^{\mathfrak{S}_{(\infty)}}$ ). To show this, it is enough to prove that  $\tilde{g}_{\lambda/\mu}$  is invariant under the action of  $s_i \in \mathfrak{S}_{(\infty)}$  for every  $i \in \mathbb{N}_+$  (because the group  $\mathfrak{S}_{(\infty)}$  is generated by the subset  $\{s_1, s_2, s_3, \dots\}$ ). In other words, it is enough to prove that  $s_i \cdot \tilde{g}_{\lambda/\mu} = \tilde{g}_{\lambda/\mu}$  for every  $i \in \mathbb{N}_+$ . So let us prove this.

Fix  $i \in \mathbb{N}_+$ . Theorem 3.4 gives us an involution  $\mathbf{B}_i : \text{RPP}(\lambda/\mu) \rightarrow \text{RPP}(\lambda/\mu)$  satisfying the property described in Theorem 3.4. Now, the definition of  $\tilde{g}_{\lambda/\mu}$  yields  $\tilde{g}_{\lambda/\mu} = \sum_{T \in \text{RPP}(\lambda/\mu)} \mathbf{t}^{\text{ceq}(T)} \mathbf{x}^{\text{ircont}(T)}$ , so that

$$s_i \cdot \tilde{g}_{\lambda/\mu} = \sum_{T \in \text{RPP}(\lambda/\mu)} \mathbf{t}^{\text{ceq}(T)} \underbrace{(s_i \cdot \mathbf{x}^{\text{ircont}(T)})}_{=\mathbf{x}^{s_i \cdot \text{ircont}(T)}} = \sum_{T \in \text{RPP}(\lambda/\mu)} \mathbf{t}^{\text{ceq}(T)} \mathbf{x}^{s_i \cdot \text{ircont}(T)}.$$

Compared with

$$\begin{aligned} \tilde{g}_{\lambda/\mu} &= \sum_{T \in \text{RPP}(\lambda/\mu)} \mathbf{t}^{\text{ceq}(T)} \mathbf{x}^{\text{ircont}(T)} = \sum_{T \in \text{RPP}(\lambda/\mu)} \underbrace{\mathbf{t}^{\text{ceq}(\mathbf{B}_i(T))}}_{=\mathbf{t}^{\text{ceq}(T)} \text{ (by (5))}} \underbrace{\mathbf{x}^{\text{ircont}(\mathbf{B}_i(T))}}_{=\mathbf{x}^{s_i \cdot \text{ircont}(T)} \text{ (by (6))}} \\ &\quad \left( \begin{array}{l} \text{here, we have substituted } \mathbf{B}_i(T) \text{ for } T \text{ in the sum} \\ \text{(since } \mathbf{B}_i : \text{RPP}(\lambda/\mu) \rightarrow \text{RPP}(\lambda/\mu) \text{ is a bijection)} \end{array} \right) \\ &= \sum_{T \in \text{RPP}(\lambda/\mu)} \mathbf{t}^{\text{ceq}(T)} \mathbf{x}^{s_i \cdot \text{ircont}(T)}, \end{aligned}$$

this yields  $s_i \cdot \tilde{g}_{\lambda/\mu} = \tilde{g}_{\lambda/\mu}$ , and this completes our proof. □

### 3.3. Reduction to 12-rpps

We shall make one further simplification before we step to the actual proof of Theorem 3.4.

- 
- The number of columns of  $\mathbf{B}_i(T)$  containing the entry  $i$  equals the number of columns of  $T$  containing the entry  $i+1$ .
  - The number of columns of  $\mathbf{B}_i(T)$  containing the entry  $i+1$  equals the number of columns of  $T$  containing the entry  $i$ .
  - For every  $h \in \mathbb{N}_+ \setminus \{i, i+1\}$ , the number of columns of  $\mathbf{B}_i(T)$  containing the entry  $h$  equals the number of columns of  $T$  containing the entry  $h$ .

<sup>11</sup>We will compare our involution  $\mathbf{B}_i$  with the  $i$ -th Bender-Knuth involution in Section 6.

We define a *12-rpp* to be an rpp whose entries all belong to the set  $\{1, 2\}$ . For

instance,

|   |   |   |   |   |
|---|---|---|---|---|
|   |   | 1 | 1 | 2 |
|   |   | 1 | 2 | 2 |
|   | 1 | 2 | 2 |   |
| 1 | 1 | 2 |   |   |

is a 12-rpp of shape  $(5, 5, 4, 3) / (2, 2, 1)$ .

Clearly, every column of a 12-rpp is a sequence of 1's followed by a sequence of 2's (where each of these sequences can be empty). The same holds for every row of a 12-rpp.

We now claim:

**Lemma 3.5.** Let  $Z$  be a finite convex subset of  $\mathbb{N}_+^2$ . Let  $\mathbf{R}$  denote the set of all 12-rpps of shape  $Z$ . Then, there exists an involution  $\mathbf{B} : \mathbf{R} \rightarrow \mathbf{R}$  (defined canonically in terms of  $Z$ ) which has the following property: For every  $S \in \mathbf{R}$ , the equalities

$$\text{ceq}(\mathbf{B}(S)) = \text{ceq}(S) \quad (7)$$

and

$$\text{ircont}(\mathbf{B}(S)) = s_1 \cdot \text{ircont}(S) \quad (8)$$

hold.

Before we prove this lemma, we will show how Theorem 3.4 can be derived from this lemma. But first of all, let us rewrite the lemma as follows:

**Lemma 3.6.** Let  $Z$  be a finite convex subset of  $\mathbb{N}_+^2$ . Let  $i \in \mathbb{N}_+$ . Let  $\mathbf{R}_Z$  denote the set of all rpps of shape  $Z$  whose entries all belong to the set  $\{i, i+1\}$ . Then, there exists an involution  $\mathbf{B}_Z : \mathbf{R}_Z \rightarrow \mathbf{R}_Z$  (defined canonically in terms of  $Z$ ) which has the following property: For every  $P \in \mathbf{R}_Z$ , the equalities

$$\text{ceq}(\mathbf{B}_Z(P)) = \text{ceq}(P) \quad (9)$$

and

$$\text{ircont}(\mathbf{B}_Z(P)) = s_i \cdot \text{ircont}(P) \quad (10)$$

hold.

*Proof of Lemma 3.6 using Lemma 3.5.* The only difference between Lemma 3.5 and Lemma 3.6 is that the entries 1 and 2 in Lemma 3.5 have been relabelled as  $i$  and  $i+1$  in Lemma 3.6. Thus, the two lemmas are equivalent, so that the latter follows from the former.

(More formally: Define  $\mathbf{R}$  as in Lemma 3.5. Then, we can define a bijection  $\Phi : \mathbf{R} \rightarrow \mathbf{R}_Z$  as follows: For every  $T \in \mathbf{R}$ , let  $\Phi(T)$  be the filling of  $Z$  which is obtained from  $T$  by replacing all 1's and 2's by  $i$ 's and  $(i+1)$ 's, respectively. Now, an involution  $\mathbf{B}_Z$  satisfying the claim of Lemma 3.6 can be constructed from an involution  $\mathbf{B}$  satisfying the claim of Lemma 3.5 by the formula  $\mathbf{B}_Z = \Phi \circ \mathbf{B} \circ \Phi^{-1}$ .)  $\square$

*Proof of Theorem 3.4 using Lemma 3.6.* Let us define a map  $\mathbf{B}_i : \text{RPP}(\lambda/\mu) \rightarrow \text{RPP}(\lambda/\mu)$ .

Indeed, let  $T \in \text{RPP}(\lambda/\mu)$ . Then,  $T^{-1}(\{i, i+1\})$  is a finite convex subset of  $Y(\lambda/\mu)$ . We denote this subset by  $Z$ . Let  $\mathbf{R}_Z$  denote the set of all rpps of shape  $Z$  whose entries all belong to the set  $\{i, i+1\}$ . Lemma 3.6 yields that there exists an involution  $\mathbf{B}_Z : \mathbf{R}_Z \rightarrow \mathbf{R}_Z$  (defined canonically in terms of  $Z$ ) which has the following property: For every  $P \in \mathbf{R}_Z$ , the equalities (9) and (10) hold. Consider this involution  $\mathbf{B}_Z$ . Clearly,  $T|_Z \in \mathbf{R}_Z$ . Hence, the involution  $\mathbf{B}_Z : \mathbf{R}_Z \rightarrow \mathbf{R}_Z$  gives rise to a  $\mathbf{B}_Z(T|_Z) \in \mathbf{R}_Z$ . Now, we define a new filling  $T'$  of  $Y(\lambda/\mu)$  as follows:

$$T'(c) = \begin{cases} (\mathbf{B}_Z(T|_Z))(c), & \text{if } c \in Z; \\ T(c), & \text{if } c \notin Z \end{cases} \quad \text{for every cell } c \text{ of } Y(\lambda/\mu).$$

In other words,  $T'$  is obtained from  $T$  by:

- replacing all entries of the restriction  $T|_Z$  (that is, all entries in cells  $c \in Z$ ) by the respective entries of  $\mathbf{B}_Z(T|_Z)$ , and
- leaving all other entries as they are.

Notice that  $T'|_Z = \mathbf{B}_Z(T|_Z)$  and  $T'|_{Y(\lambda/\mu) \setminus Z} = T|_{Y(\lambda/\mu) \setminus Z}$ . These two equalities determine  $T'$ . It is easy to see that  $T'$  is an rpp of shape  $Y(\lambda/\mu)$ . That is,  $T' \in \text{RPP}(\lambda/\mu)$ . We now define  $\mathbf{B}_i(T) = T'$ . Thus, a map  $\mathbf{B}_i : \text{RPP}(\lambda/\mu) \rightarrow \text{RPP}(\lambda/\mu)$  is defined.

The reader can easily verify that this map  $\mathbf{B}_i$  is an involution, and that every  $T \in \text{RPP}(\lambda/\mu)$  satisfies (5) and (6). (Essentially, these properties follow from the analogous properties of the map  $\mathbf{B}_Z$ , once one realizes that every  $T \in \text{RPP}(\lambda/\mu)$  satisfies

$$\begin{aligned} (\mathbf{B}_i(T))^{-1}(\{i, i+1\}) &= T^{-1}(\{i, i+1\}), \\ \text{ceq}(T) &= \text{ceq}(T|_Z) + \text{ceq}(T|_{Y(\lambda/\mu) \setminus Z}) \end{aligned}$$

and

$$\text{ircont}(T) = \text{ircont}(T|_Z) + \underbrace{\text{ircont}(T|_{Y(\lambda/\mu) \setminus Z})}_{\text{This composition is invariant under } s_i \text{ (because its } i\text{-th and } (i+1)\text{-th entries are zero)}}.$$

)

**Example 3.7.** Let us give an example of how  $\mathbf{B}_i$  acts on an rpp. Assume for this example that  $\lambda = (9, 8, 8, 7)$  and  $\mu = (4, 3, 2, 1)$ , and let  $T$  be the filling

|   |   |   |   |   |   |   |   |
|---|---|---|---|---|---|---|---|
|   |   |   | 1 | 3 | 3 | 4 | 5 |
|   |   | 1 | 1 | 3 | 4 | 6 |   |
|   | 1 | 2 | 3 | 4 | 5 | 6 |   |
| 1 | 1 | 2 | 3 | 4 | 8 |   |   |

(there is an invisible empty 1-st column here). Set  $i = 3$ . Then,  $Z = T^{-1}(\{i, i+1\})$  is the set

$$\{(1, 6), (1, 7), (1, 8), (2, 6), (2, 7), (3, 5), (3, 6), (4, 5), (4, 6)\}.$$

The rpp  $T|_Z$  is

|   |   |   |   |
|---|---|---|---|
|   | 3 | 3 | 4 |
|   | 3 | 4 |   |
| 3 | 4 |   |   |
| 3 | 4 |   |   |

(with the first four columns being empty and invisible). We have not defined  $\mathbf{B}_Z$  yet, but let us assume that  $\mathbf{B}_Z$  maps this rpp  $T|_Z$  to

$$\mathbf{B}_Z(T|_Z) = \begin{array}{cccc} & & 3 & 3 & 3 \\ & & 3 & 4 & \\ & 4 & 4 & & \\ & 4 & 4 & & \end{array}.$$

(This is, in fact, what the map  $\mathbf{B}_Z$  defined below does to  $T|_Z$ .) Then,  $\mathbf{B}_i(T)$  is obtained from  $T$  by replacing the entries of  $T|_Z$  by the respective entries of  $\mathbf{B}_Z(T|_Z)$ , while leaving all other entries as they are. Thus,

$$\mathbf{B}_i(T) = \begin{array}{cccccc} & & & 1 & 3 & 3 & 3 & 5 \\ & & & 1 & 1 & 3 & 4 & 6 \\ & & 1 & 2 & 4 & 4 & 5 & 6 \\ 1 & 1 & 2 & 4 & 4 & 8 & & \end{array}.$$

□



## 4. A diamond lemma

### 4.1. The lemma

By now we have derived Theorem 3.4 from Lemma 3.6, and Lemma 3.6 from Lemma 3.5. In order to complete the puzzle, we need to prove Lemma 3.5. To do so, let us first state a simple lemma.

**Lemma 4.1.** Let  $\mathbf{S}$  be a finite set. Let  $\ell : \mathbf{S} \rightarrow \mathbb{N}$  be a map. Let  $\Rightarrow$  be a binary relation on the set  $\mathbf{S}$ . (We shall write this relation in infix form; i.e., we will write “ $a \Rightarrow b$ ” to mean “ $(a, b)$  belongs to the relation  $\Rightarrow$ ”.)

Define a new binary relation  $\Rightarrow^*$  on  $\mathbf{S}$  (also written in infix form) as follows: For two elements  $a \in \mathbf{S}$  and  $b \in \mathbf{S}$ , we set  $a \Rightarrow^* b$  if and only if there exists a sequence  $(a_0, a_1, \dots, a_n)$  of elements of  $\mathbf{S}$  such that  $a_0 = a$  and  $a_n = b$  and such that every  $i \in \{0, 1, \dots, n-1\}$  satisfies  $a_i \Rightarrow a_{i+1}$ .<sup>12</sup> (In other words, we define  $\Rightarrow^*$  as the reflexive-and-transitive closure of the relation  $\Rightarrow$ .)

Assume that the following two hypotheses are true:

- The *local confluence hypothesis*: If  $a, b$  and  $c$  are three elements of  $\mathbf{S}$  satisfying  $a \Rightarrow b$  and  $a \Rightarrow c$ , then there exists a  $d \in \mathbf{S}$  such that  $b \Rightarrow^* d$  and  $c \Rightarrow^* d$ .
- The *length-decrease hypothesis*: If  $a \in \mathbf{S}$  and  $b \in \mathbf{S}$  are two elements satisfying  $a \Rightarrow b$ , then  $\ell(a) > \ell(b)$ .

We say that an element  $a \in \mathbf{S}$  is *final* if there exists no  $b \in \mathbf{S}$  satisfying  $a \Rightarrow b$ . Then, for every  $a \in \mathbf{S}$ , there exists a unique final element  $b \in \mathbf{S}$  such that  $a \Rightarrow^* b$ .

Lemma 4.1 is an easy particular case of what is called *Newman’s lemma* (see, e.g., [BezCoq03], or [BaaNip98, Lemma 2.7.2 + Fact 2.1.7]).<sup>13</sup> (Some authors refer to Newman’s lemma as the *diamond lemma*, but the latter name is shared with at least one different fact.)

For the sake of completeness, we shall give the simple proof of Lemma 4.1.

*Proof of Lemma 4.1.* The relation  $\Rightarrow^*$  is the reflexive-and-transitive closure of the relation  $\Rightarrow$ . This yields the following properties (all of which are easy to check):

<sup>12</sup>Notice that  $n$  is allowed to be 0 here.

<sup>13</sup>In the general version, the finiteness of  $\mathbf{S}$  and the length-decrease hypothesis are replaced by a requirement that there exist no infinite sequences  $(a_0, a_1, a_2, \dots) \in \mathbf{S}^\infty$  such that every  $i \in \mathbb{N}$  satisfies  $a_i \Rightarrow a_{i+1}$ . The proof of this generalization is harder than that of Lemma 4.1, and not constructive. While there is a constructive reformulation of this generalization (presented in [BezCoq03, Lemma 3.3]), we do not have a use for it in this paper.

- The relation  $\Rightarrow^*$  is reflexive and transitive and extends the relation  $\Rightarrow$ .
- If  $a \in \mathbf{S}$  and  $b \in \mathbf{S}$  are elements satisfying  $a \Rightarrow^* b$  and  $a \neq b$ , then

$$\text{there exists a } c \in \mathbf{S} \text{ such that } a \Rightarrow c \text{ and } c \Rightarrow^* b. \quad (11)$$

- We have

$$\ell(a) \geq \ell(b) \quad \text{for any } a \in \mathbf{S} \text{ and } b \in \mathbf{S} \text{ satisfying } a \Rightarrow^* b \quad (12)$$

(because of the length-decrease hypothesis).

Now, we need to show that, for every  $a \in \mathbf{S}$ ,

$$\text{there exists a unique final element } b \in \mathbf{S} \text{ such that } a \Rightarrow^* b. \quad (13)$$

*Proof of (13):* We shall prove (13) by strong induction over  $\ell(a)$ .

*Induction step:* Let  $N \in \mathbb{N}$ . Assume (as the induction hypothesis) that (13) is proven for every  $a \in \mathbf{S}$  satisfying  $\ell(a) < N$ . We need to prove that (13) holds for every  $a \in \mathbf{S}$  satisfying  $\ell(a) = N$ .

Let  $a \in \mathbf{S}$  be such that  $\ell(a) = N$ . We need to show that (13) holds for this  $a$ .

If there exists no  $c \in \mathbf{S}$  satisfying  $a \Rightarrow c$ , then (13) holds<sup>14</sup>. Hence, for the rest of this proof, we WLOG assume that there exists some  $c \in \mathbf{S}$  satisfying  $a \Rightarrow c$ . Let us denote this  $c$  by  $c_1$ . Thus,  $c_1 \in \mathbf{S}$  and  $a \Rightarrow c_1$ . Applying the length-decrease hypothesis to  $b = c_1$ , we thus obtain  $\ell(a) > \ell(c_1)$ , so that  $\ell(c_1) < \ell(a) = N$ . Thus, we can apply (13) to  $c_1$  instead of  $a$  (according to the induction hypothesis). As a result, we conclude that there exists a unique final element  $b \in \mathbf{S}$  such that  $c_1 \Rightarrow^* b$ . Let us denote this  $b$  by  $b_1$ . Thus,  $b_1$  is a final element of  $\mathbf{S}$  such that  $c_1 \Rightarrow^* b_1$ .

Since  $a \Rightarrow c_1$ , we have  $a \Rightarrow^* c_1$  (since the relation  $\Rightarrow^*$  extends the relation  $\Rightarrow$ ). Combining this with  $c_1 \Rightarrow^* b_1$ , we obtain  $a \Rightarrow^* b_1$  (since the relation  $\Rightarrow^*$  is transitive). Thus, there exists a final element  $b \in \mathbf{S}$  such that  $a \Rightarrow^* b$  (namely,  $b = b_1$ ). We shall now prove that such a  $b$  is unique.

Indeed, let  $b_2$  be any final element  $b \in \mathbf{S}$  such that  $a \Rightarrow^* b$ . Thus,  $b_2$  is a final element of  $\mathbf{S}$  such that  $a \Rightarrow^* b_2$ . We will prove that  $b_2 = b_1$ .

It is easy to see that  $a \neq b_2$  (because  $a \Rightarrow c_1$  shows that  $a$  is not final, but  $b_2$  is final). Hence, (11) (applied to  $b = b_2$ ) yields that there exists a  $c \in \mathbf{S}$  such that

---

<sup>14</sup>*Proof.* Assume that there exists no  $c \in \mathbf{S}$  satisfying  $a \Rightarrow c$ . Then,  $a$  itself is final. Hence, there exists a final element  $b \in \mathbf{S}$  such that  $a \Rightarrow^* b$  (namely,  $b = a$ ). This  $b$  is unique, because (11) shows that every  $b \in \mathbf{S}$  satisfying  $a \Rightarrow^* b$  and  $a \neq b$  would have to satisfy  $a \Rightarrow c$  for some  $c \in \mathbf{S}$  (which would contradict the fact that  $a$  is final). This proves (13).

$a \Rightarrow c$  and  $c \xRightarrow{*} b_2$ . Let us denote this  $c$  by  $c_2$ . Then,  $c_2$  is an element of  $\mathbf{S}$  such that  $a \Rightarrow c_2$  and  $c_2 \xRightarrow{*} b_2$ .

The local confluence hypothesis (applied to  $c_1$  and  $c_2$  instead of  $b$  and  $c$ ) shows that there exists a  $d \in \mathbf{S}$  such that  $c_1 \xRightarrow{*} d$  and  $c_2 \xRightarrow{*} d$ . Consider such a  $d$ . Applying (12) to  $c_1$  and  $d$  instead of  $a$  and  $b$ , we obtain  $\ell(c_1) \geq \ell(d)$ , so that  $\ell(d) \leq \ell(c_1) < N$ . Hence, we can apply (13) to  $d$  instead of  $a$  (according to the induction hypothesis). As a result, we conclude that there exists a unique final element  $b \in \mathbf{S}$  such that  $d \xRightarrow{*} b$ . Let us denote this  $b$  by  $e$ . Thus,  $e$  is a final element of  $\mathbf{S}$  such that  $d \xRightarrow{*} e$ .

We have  $c_1 \xRightarrow{*} d$  and  $d \xRightarrow{*} e$ . Hence,  $c_1 \xRightarrow{*} e$  (since the relation  $\xRightarrow{*}$  is transitive). Thus,  $e$  is a final element of  $\mathbf{S}$  such that  $c_1 \xRightarrow{*} e$ . In other words,  $e$  is a final element  $b \in \mathbf{S}$  such that  $c_1 \xRightarrow{*} b$ . Since we already know that  $b_1$  is the unique such element  $b$  (in fact, this is how we defined  $b_1$ ), this shows that  $e = b_1$ .

We have  $c_2 \xRightarrow{*} d$  and  $d \xRightarrow{*} e$ . Hence,  $c_2 \xRightarrow{*} e$  (since the relation  $\xRightarrow{*}$  is transitive). In other words,  $c_2 \xRightarrow{*} b_1$  (since  $e = b_1$ ). Hence,  $b_1$  is a final element of  $\mathbf{S}$  such that  $c_2 \xRightarrow{*} b_1$ . In other words,  $b_1$  is a final element  $b \in \mathbf{S}$  such that  $c_2 \xRightarrow{*} b$ . Also,  $b_2$  is a final element  $b \in \mathbf{S}$  such that  $c_2 \xRightarrow{*} b$  (since  $b_2$  is final and since  $c_2 \xRightarrow{*} b_2$ ).

But applying the length-decrease hypothesis to  $b = c_2$ , we obtain  $\ell(a) > \ell(c_2)$  (since  $a \Rightarrow c_2$ ), so that  $\ell(c_2) < \ell(a) = N$ . Thus, we can apply (13) to  $c_2$  instead of  $a$  (according to the induction hypothesis). As a result, we conclude that there exists a unique final element  $b \in \mathbf{S}$  such that  $c_2 \xRightarrow{*} b$ . The “uniqueness” part of this result gives us  $b_2 = b_1$  (since both  $b_2$  and  $b_1$  are final elements  $b \in \mathbf{S}$  such that  $c_2 \xRightarrow{*} b$ ).

Now let us forget that we fixed  $b_2$ . We thus have shown that if  $b_2$  is any final element  $b \in \mathbf{S}$  such that  $a \xRightarrow{*} b$ , then  $b_2 = b_1$ . Hence, there exists at most one final element  $b \in \mathbf{S}$  such that  $a \xRightarrow{*} b$ . As a consequence, there exists a unique final element  $b \in \mathbf{S}$  such that  $a \xRightarrow{*} b$  (because we already know that there exists such a  $b$ ). In other words, (13) holds. This completes the induction step. The induction proof of (13) is thus complete. In other words, Lemma 4.1 is proven.  $\square$

## 4.2. Example: Sorting $n$ -tuples by local transpositions

Let us give a simple example of an application of Lemma 4.1. This example (which will take up the whole Subsection 4.2) will not be used in the rest of the paper, but it serves as a kind of prototype that our proof of Lemma 3.5 imitates, and so might help clarifying the latter proof.

All of the definitions and conventions that will be made in this Subsection 4.2 are supposed to stand only for this Subsection. (In particular, the meanings of

the letter **S** and the symbol  $\Rightarrow$  will later be used for completely different things.)

For the rest of Subsection 4.2, we fix  $n \in \mathbb{N}$ , and we fix a poset  $P$ .

For any  $n$ -tuple  $z \in P^n$  and every  $i \in \{1, 2, \dots, n\}$ , we use the notation  $z_i$  to denote the  $i$ -th entry of  $z$ . (Thus,  $z = (z_1, z_2, \dots, z_n)$  for every  $z \in P^n$ .)

Before we go into further details, let us informally explain what we will prove in the following. Imagine that we start with some  $n$ -tuple  $z = (z_1, z_2, \dots, z_n)$  of elements of  $P$ , and we want to “sort it in nondecreasing order”. We do this by repeatedly picking an index  $k \in \{1, 2, \dots, n-1\}$  satisfying  $z_k > z_{k+1}$ , and switching the entries  $z_k$  and  $z_{k+1}$  in the tuple, and continuing in the same way until we can no longer find such a  $k$ .<sup>15</sup> It is easy to see that this process will eventually terminate, leaving behind an  $n$ -tuple  $z$  such that no  $k \in \{1, 2, \dots, n-1\}$  satisfies  $z_k > z_{k+1}$  (although, in general, it will not satisfy  $z_1 \leq z_2 \leq \dots \leq z_n$ , as  $P$  is only partially ordered). But a priori, it is not clear whether this resulting  $n$ -tuple could depend on the choices we made in the “sorting” process<sup>16</sup>. It turns out that it does not, but this is not completely trivial. We shall now formalize this fact. We prefer not to talk about processes, nor to regard  $z$  as mutable; instead, we will introduce a binary relation on the set of all permutations of a given  $n$ -tuple, which will model the idea of a “step” of our “sorting” process.

For every  $k \in \{1, 2, \dots, n-1\}$ , let  $s_k$  be the transposition  $(k, k+1) \in \mathfrak{S}_n$ . The group  $\mathfrak{S}_n$  acts on  $P^n$  by permuting the coordinates:

$$\sigma \cdot z = (z_{\sigma^{-1}(1)}, z_{\sigma^{-1}(2)}, \dots, z_{\sigma^{-1}(n)}) \quad \text{for all } \sigma \in \mathfrak{S}_n \text{ and } z \in P^n.$$

In particular, for each  $k \in \{1, 2, \dots, n-1\}$  and  $z \in P^n$ , the  $n$ -tuple  $s_k \cdot z$  is obtained from  $z$  by switching the  $k$ -th and the  $(k+1)$ -th entries.

<sup>15</sup>Here is an example: If  $P$  is the four-element poset  $\{a, b, c, d\}$  with relations  $a < b < d$  and  $a < c < d$ , if  $n = 6$ , and if  $z = (d, b, d, c, a, b)$ , then our sorting process can look as follows:

$$\begin{aligned} (d, b, d, c, a, b) &\rightarrow (b, d, \underline{d, c}, a, b) \rightarrow (b, d, c, d, a, b) \rightarrow (b, c, d, \underline{d, a}, b) \rightarrow (b, c, d, a, d, b) \\ &\rightarrow (b, c, \underline{a, d}, d, b) \rightarrow (\underline{b, a}, c, d, d, b) \rightarrow (a, b, c, d, \underline{d, b}) \rightarrow (a, b, c, d, b, d) \\ &\rightarrow (a, b, c, b, d, d) \end{aligned}$$

(where an underline under two adjacent entries of a tuple means that these entries are going to be switched in the next step). The final result  $(a, b, c, b, d, d)$  is “sorted” in the sense that we can no longer find a  $k \in \{1, 2, \dots, n-1\}$  such that  $z_k > z_{k+1}$ .

We notice that we had some freedom in performing our sorting process: e.g., we could have started out by switching the  $d$  with the  $c$  in the  $(d, b, d, c, a, b)$  rather than by switching the  $d$  with the  $b$ .

This is similar to the bubble sort algorithm, but there are two differences: Firstly,  $P$  is now a poset, not a totally ordered set (so we cannot hope to get our  $n$ -tuple  $z$  to satisfy  $z_1 \leq z_2 \leq \dots \leq z_n$  in the end). Secondly, we are allowed to pick an index  $k \in \{1, 2, \dots, n-1\}$  satisfying  $z_k > z_{k+1}$  arbitrarily (so our process is nondeterministic), rather than having to scan the  $n$ -tuple from left to right (in multiple passes) as in the classical bubble sort algorithm.

<sup>16</sup>Namely, at every step of our process, we had to choose an index  $k \in \{1, 2, \dots, n-1\}$  satisfying  $z_k > z_{k+1}$ . Whenever this index  $k$  was not unique, we had freedom in choosing one of them to start with. These choices have an effect on the “sorting” process, and so it would not be surprising if the final result would depend on them too.

**Definition 4.2.** Fix  $w \in P^n$ . Let  $\mathbf{S}$  be the set of all permutations of  $w$ . Clearly,  $\mathbf{S}$  is a finite set (having at most  $n!$  elements). Moreover,  $\mathbf{S}$  is an  $\mathfrak{S}_n$ -subset of the  $\mathfrak{S}_n$ -set  $P^n$ .

Let us define a binary relation  $\Rightarrow$  on this set  $\mathbf{S}$  as follows: Let  $a \in \mathbf{S}$  and  $b \in \mathbf{S}$ . If  $k \in \{1, 2, \dots, n-1\}$ , then we write  $a \xRightarrow[k]{\Rightarrow} b$  if and only if  $a_k > a_{k+1}$  and  $b = s_k \cdot a$ . We write  $a \Rightarrow b$  if and only if there exists an  $k \in \{1, 2, \dots, n-1\}$  such that  $a \xRightarrow[k]{\Rightarrow} b$ . (In other words, we write  $a \Rightarrow b$  if and only if the  $n$ -tuple  $b$  can be obtained from  $a$  by switching two adjacent entries which are out of order in  $a$ . Here, we say that two entries of  $a$  are *out of order* if the left one is greater than the right one.) Thus, the relation  $\Rightarrow$  is defined.

For example, if  $n = 5$ ,  $P = \mathbb{Z}$  and  $w = (3, 1, 6, 3, 5)$ , then  $(1, 6, 3, 5, 3) \xRightarrow[2]{\Rightarrow} (1, 3, 6, 5, 3)$  (and thus  $(1, 6, 3, 5, 3) \Rightarrow (1, 3, 6, 5, 3)$ ) but not  $(1, 6, 3, 5, 3) \xRightarrow[3]{\Rightarrow} (1, 6, 5, 3, 3)$  (since we required  $a_k > a_{k+1}$  when defining  $a \xRightarrow[k]{\Rightarrow} b$ ).

We define a binary relation  $\xRightarrow{*}$  on  $\mathbf{S}$  as in Lemma 4.1. This relation  $\xRightarrow{*}$  is the reflexive-and-transitive closure of the relation  $\Rightarrow$ . Thus, the relation  $\xRightarrow{*}$  is reflexive and transitive and extends the relation  $\Rightarrow$ .

We also define the notion of a “final” element of  $\mathbf{S}$  as in Lemma 4.1. Now, it is easy to see that an element  $u \in \mathbf{S}$  is final if and only if no  $k \in \{1, 2, \dots, n-1\}$  satisfies  $u_k > u_{k+1}$ .

Now, we claim:

**Proposition 4.3.** For every  $a \in \mathbf{S}$ , there exists a unique final element  $b \in \mathbf{S}$  such that  $a \xRightarrow{*} b$ .

In words, Proposition 4.3 says that if we start with some  $n$ -tuple  $a \in \mathbf{S}$  and repeatedly switch adjacent entries of  $a$  which are out of order, then the procedure eventually terminates (i.e., eventually we will arrive at an  $n$ -tuple which has no two adjacent entries that are out of order) and the resulting  $n$ -tuple does not depend on the choices we made in the process (i.e., even if there were several choices of adjacent entries to switch, they all lead to the same final result).<sup>17</sup> The only reason why we are working in  $\mathbf{S}$  instead of the whole set  $P^n$  is that  $\mathbf{S}$  is always finite, which will make it easier for us to apply Lemma 4.1.

**Remark 4.4.** It is important that we are switching adjacent entries of  $a$ . If we start with some  $n$ -tuple  $a \in \mathbf{S}$  and repeatedly switch entries of  $a$  which are out of order but **not necessarily** adjacent, then the result of this procedure (once it has terminated) might well depend on our choices. (For instance, if  $P$  is the poset  $\{1, 2, 2'\}$  with relations  $1 < 2$  and  $1 < 2'$ , and if  $n = 3$  and

<sup>17</sup>Strictly speaking, Proposition 4.3 does not really say that the procedure eventually terminates; but this will follow from the length-decrease hypothesis in its proof below.

$a = (2, 2', 1)$ , then switching the first and the third entries leads to  $(1, 2', 2)$ , whereas switching the second and the third entries and then switching the first and the second entries yields  $(1, 2, 2')$ ; and these two results are both final and nevertheless distinct.)

Proposition 4.3 is rather obvious in the case when  $P$  is totally ordered (indeed, in this case, the unique final element  $b \in \mathbf{S}$  such that  $a \xRightarrow{*} b$  will simply be the  $n$ -tuple obtained by rearranging  $a$  in nondecreasing order). But let us prove Proposition 4.3 in the general case using Lemma 4.1.

*Proof of Proposition 4.3.* If  $z \in P^n$ , then an *inversion* of  $z$  means a pair  $(i, j) \in \{1, 2, \dots, n\}^2$  with  $i < j$  and  $z_i > z_j$ . For instance, if  $n = 5$  and  $P = \mathbb{Z}$  (as posets, where  $\mathbb{Z}$  is equipped with the usual order), then the inversions of  $(3, 1, 6, 3, 5)$  are  $(1, 2)$ ,  $(3, 4)$  and  $(3, 5)$ .

Define a map  $\ell : P^n \rightarrow \mathbb{N}$  as follows: For every  $z \in P^n$ , let  $\ell(z)$  be the number of inversions of  $z$ . Clearly,  $\ell(z) \in \mathbb{N}$  and  $\ell(z) \leq \binom{n}{2}$ .

We need to show that for every  $a \in \mathbf{S}$ , there exists a unique final element  $b \in \mathbf{S}$  such that  $a \xRightarrow{*} b$ . According to Lemma 4.1, it is enough to check that the local confluence hypothesis and the length-decrease hypothesis are satisfied<sup>18</sup>.

*Proof that the length-decrease hypothesis is satisfied:* Let  $a \in \mathbf{S}$  and  $b \in \mathbf{S}$  be such that  $a \xRightarrow{*} b$ . Then, there exists a  $k \in \{1, 2, \dots, n-1\}$  such that  $a \xRightarrow{k} b$  (since  $a \xRightarrow{*} b$ ). Consider this  $k$ . We have  $a \xRightarrow{k} b$ ; in other words,  $a_k > a_{k+1}$  and  $b = s_k \cdot a$ . In other words, the  $n$ -tuple  $b$  is obtained from  $a$  by switching the  $k$ -th and the  $(k+1)$ -th entry, which were out of order in  $a$ . Thus, the pair  $(k, k+1)$  is an inversion of  $a$ , but not an inversion of  $b$ . Furthermore,  $b_{s_k(u)} = a_u$  for every  $u \in \{1, 2, \dots, n\}$  (since  $b = s_k \cdot a$ ). Furthermore, for any  $(i, j) \in \{1, 2, \dots, n\}^2$  satisfying  $i < j$ , we have  $s_k(i) < s_k(j)$  if  $(i, j) \neq (k, k+1)$  (this is easy to prove by checking all possible cases). From the last two observations, we can easily conclude that the inversions of  $b$  are precisely the pairs of the form  $(s_k(i), s_k(j))$  with  $(i, j)$  being an inversion of  $a$  satisfying  $(i, j) \neq (k, k+1)$ . Thus, the number of inversions of  $b$  is one less than the number of inversions of  $a$  (because  $(k, k+1)$  is an inversion of  $a$ , and thus its exclusion lowers the count by 1). In other words,  $\ell(b) = \ell(a) - 1$  (because  $\ell(z)$  means the number of inversions of  $z$  whenever  $z \in P^n$ ). Thus,  $\ell(a) > \ell(b)$ . Hence, the length-decrease hypothesis is proven.

*Proof that the local confluence hypothesis is satisfied:* Let  $a, b$  and  $c$  be three elements of  $\mathbf{S}$  satisfying  $a \xRightarrow{*} b$  and  $a \xRightarrow{*} c$ . We need to show that there exists a  $d \in \mathbf{S}$  such that  $b \xRightarrow{*} d$  and  $c \xRightarrow{*} d$ .

We have  $a \xRightarrow{*} b$ . In other words, the  $n$ -tuple  $b$  can be obtained from  $a$  by switching two adjacent entries which are out of order in  $a$ . In other words, we

<sup>18</sup>Both of these hypotheses were stated in Lemma 4.1.

can write  $a$  and  $b$  in the forms

$$a = (\dots, p, q, \dots) \quad \text{and} \quad b = (\dots, q, p, \dots) \quad (14)$$

for some  $p \in P$  and  $q \in P$  satisfying  $p > q$ , where the “...” stand for strings<sup>19</sup> of entries of  $a$  that appear unchanged in  $b$ . Similarly, we can write  $a$  and  $c$  in the forms

$$a = (\dots, r, t, \dots) \quad \text{and} \quad c = (\dots, t, r, \dots) \quad (15)$$

for some  $r \in P$  and  $t \in P$  satisfying  $r > t$ , where the “...” stand for strings of entries of  $a$  that appear unchanged in  $c$ . Consider the  $p$  and  $q$  from (14), and the  $r$  and  $t$  from (15). Also, let  $u$  and  $u + 1$  be the positions of  $p$  and  $q$  in  $a$  in (14). Furthermore, let  $v$  and  $v + 1$  be the positions of  $r$  and  $t$  in  $a$  in (15).

We WLOG assume that  $u \leq v$ , because otherwise we can simply switch  $b$  with  $c$  (thus forcing  $u$  to switch with  $v$ ). Moreover, we can WLOG assume that  $u \neq v$  (because if  $u = v$ , then finding a  $d \in \mathbf{S}$  such that  $b \xrightarrow{*} d$  and  $c \xrightarrow{*} d$  is trivial<sup>20</sup>). Thus,  $u < v$  (since  $u \leq v$ ).

Let us now try to combine the representations (14) for  $a$  and  $b$  with the representations (15) for  $a$  and  $c$  into a set of representations for  $a$ ,  $b$  and  $c$  in which both the changes from  $a$  to  $b$  and the changes from  $a$  to  $c$  are visible at the same time. We must be in one of the following two cases:

Case 1: We have  $u < v - 1$ .

Case 2: We have  $u = v - 1$ .

Let us first consider Case 1. In this case, we can merge the representations (14) and (15) as follows:

$$a = (\dots, p, q, \dots, r, t, \dots), \quad b = (\dots, q, p, \dots, r, t, \dots), \quad c = (\dots, p, q, \dots, t, r, \dots),$$

where the “...” stand for strings of entries of  $a$  that appear unchanged in both  $b$  and  $c$ . Thus, we can find a  $d \in \mathbf{S}$  such that  $b \xrightarrow{*} d$  and  $c \xrightarrow{*} d$ : namely, set

$$d = (\dots, q, p, \dots, t, r, \dots)$$

(where the “...” have the same meaning as before). Thus, the local confluence hypothesis is proven in Case 1.

Let us now consider Case 2. In this case,  $u = v - 1$ . Hence,  $u + 1 = v$ . Now,  $q$  is the  $(u + 1)$ -th entry of  $a$ , that is, the  $v$ -th entry of  $a$  (since  $u + 1 = v$ ); but  $r$  is also the  $v$ -th entry of  $a$ . Hence,  $q = r$ , so that  $p > q = r > t$ . Now, we can merge the representations (14) and (15) as follows:

$$a = (\dots, p, q, t, \dots), \quad b = (\dots, q, p, t, \dots), \quad c = (\dots, p, t, q, \dots),$$

<sup>19</sup>These strings are allowed to be empty.

<sup>20</sup>*Proof.* Assume that  $u = v$ . Thus, the  $p$  and  $q$  in (14) appear in the same positions as the  $r$  and  $t$  in (15). Hence, both  $b$  and  $c$  are obtained from  $a$  in one and the same way (namely, by switching the entries in these positions). Hence,  $b = c$ . Thus, we can find a  $d \in \mathbf{S}$  such that  $b \xrightarrow{*} d$  and  $c \xrightarrow{*} d$  just by setting  $d = b = c$ , qed.

where the “...” stand for strings of entries of  $a$  that appear unchanged in both  $b$  and  $c$ . Let us now set

$$e = (\dots, q, t, p, \dots), \quad f = (\dots, t, p, q, \dots), \quad d = (\dots, t, q, p, \dots)$$

(where the “...” have the same meaning as before). Then,  $b \Rightarrow e$  and  $e \Rightarrow d$ ; thus,  $b \stackrel{*}{\Rightarrow} d$  (since  $\stackrel{*}{\Rightarrow}$  is the reflexive-and-transitive closure of  $\Rightarrow$ ). Also,  $c \Rightarrow f$  and  $f \Rightarrow d$ ; thus,  $c \stackrel{*}{\Rightarrow} d$  (since  $\stackrel{*}{\Rightarrow}$  is the reflexive-and-transitive closure of  $\Rightarrow$ ). Hence, we have found a  $d \in \mathbf{S}$  such that  $b \stackrel{*}{\Rightarrow} d$  and  $c \stackrel{*}{\Rightarrow} d$ . Thus, the local confluence hypothesis is proven in Case 2 as well.

The local confluence hypothesis thus holds (because it is proven in both Cases 1 and 2).

We now know that both the local confluence hypothesis and the length-decrease hypothesis are satisfied. This completes the proof of Proposition 4.3.  $\square$

## 5. Proof of Lemma 3.5

We now come to the actual proof of Lemma 3.5. For the whole Section 5, we shall be working in the situation of Lemma 3.5.

### 5.1. 12-tables and the four types of their columns

Let  $Z$  be a finite convex subset of  $\mathbb{N}_+^2$ . We shall keep  $Z$  fixed for the rest of Section 5. Let  $\mathbf{R}$  denote the set of all 12-rpps of shape  $Z$ .

A *12-table* will mean a map  $T : Z \rightarrow \{1, 2\}$  such that the entries of  $T$  are weakly increasing down columns. (We do not require them to be weakly increasing along rows.) Every column of a 12-table is a sequence of the form

$$\left( \underbrace{1, 1, \dots, 1}_{u \text{ times } 1}, \underbrace{2, 2, \dots, 2}_{v \text{ times } 2} \right) \text{ with } u \in \mathbb{N} \text{ and } v \in \mathbb{N}. \text{ We say that such a sequence is}$$

- *1-pure* if it is nonempty and consists purely of 1's (that is,  $u > 0$  and  $v = 0$ );
- *2-pure* if it is nonempty and consists purely of 2's (that is,  $u = 0$  and  $v > 0$ );
- *mixed* if it contains both 1's and 2's (that is,  $u > 0$  and  $v > 0$ ).

Consequently, every column of a 12-table is either empty or 1-pure or 2-pure or mixed (and these four cases do not overlap).

Also, if  $s$  is a sequence of the form  $\left( \underbrace{1, 1, \dots, 1}_{u \text{ times } 1}, \underbrace{2, 2, \dots, 2}_{v \text{ times } 2} \right)$  with  $u \in \mathbb{N}$  and  $v \in \mathbb{N}$ , then we define the *signature* of  $s$  to be the nonnegative integer



$\begin{cases} 0, & \text{if } s \text{ is 2-pure or empty;} \\ 1, & \text{if } s \text{ is mixed;} \\ 2, & \text{if } s \text{ is 1-pure} \end{cases}$ . We denote this signature by  $\text{sig}(s)$ . For any 12-table  $T$ , we define a nonnegative integer  $\ell(T)$  by

$$\ell(T) = \sum_{h \in \mathbb{N}_+} h \cdot \text{sig}(\text{the } h\text{-th column of } T).$$

<sup>21</sup> For instance, if  $T =$ 

|   |   |   |   |   |   |   |
|---|---|---|---|---|---|---|
|   |   |   | 1 | 2 | 1 | 2 |
|   |   | 1 | 1 | 2 |   |   |
| 2 | 1 | 1 | 2 |   |   |   |
| 2 | 2 |   |   |   |   |   |

 , then  $\ell(T) = 1 \cdot 0 + 2 \cdot 1 + 3 \cdot 2 + 4 \cdot 0 + 5 \cdot 2 + 6 \cdot 0 + 7 \cdot 0 + 8 \cdot 0 + \dots = 18$ .

## 5.2. Conflicts of 12-tables

If  $T$  is a 12-table, then we define a *conflict* of  $T$  to be a pair  $(i, j)$  of positive integers satisfying  $i < j$  such that there exists an  $r \in \mathbb{N}_+$  satisfying  $(r, i) \in Z$ ,  $(r, j) \in Z$ ,  $T(r, i) = 2$  and  $T(r, j) = 1$ . (Speaking visually, a conflict of  $T$  is a pair  $(i, j)$  of positive integers such that the filling  $T$  has an entry 2 in column  $i$  lying due west of an entry 1 in column  $j$ .) For instance, the conflicts of the 12-table

|   |   |   |   |   |   |   |
|---|---|---|---|---|---|---|
|   |   |   | 1 | 2 | 1 | 2 |
|   |   | 1 | 1 | 2 |   |   |
| 2 | 1 | 1 | 2 |   |   |   |
| 2 | 2 |   |   |   |   |   |

 are  $(1, 2)$ ,  $(1, 3)$  and  $(4, 5)$ .

(The notion of a conflict of  $T$  is in some sense analogous to that of an inversion of  $z$  in Subsection 4.2.)

Clearly, a 12-rpp of shape  $Z$  is the same as a 12-table which has no conflicts.<sup>22</sup>

**Proposition 5.1.** Let  $T$  be a 12-table. Let  $a, b$  and  $c$  be positive integers such that  $(a, b)$  and  $(b, c)$  are conflicts of  $T$ . Then,  $(a, c)$  also is a conflict of  $T$ .

**Example 5.2.** If  $T =$ 

|   |   |   |
|---|---|---|
|   |   | 1 |
| 2 | 1 | 1 |
| 2 | 2 | 1 |

 , then  $(1, 2)$  and  $(2, 3)$  are conflicts of  $T$ , and so is  $(1, 3)$ . One can notice that every row which “witnesses” the conflict  $(1, 2)$  will also “witness” the conflict  $(1, 3)$  (where we say that the  $r$ -th row *witnesses* a conflict  $(i, j)$  if and only if  $(r, i) \in Z$ ,  $(r, j) \in Z$ ,  $T(r, i) = 2$  and  $T(r, j) = 1$ ).

<sup>21</sup>This is well-defined, because all but finitely many  $h \in \mathbb{N}_+$  satisfy  $\text{sig}(\text{the } h\text{-th column of } T) = 0$  (since for all but finitely many  $h \in \mathbb{N}_+$ , the  $h$ -th column of  $T$  is empty).

<sup>22</sup>Indeed, the conflicts of a 12-table stem from the failures of its entries to be weakly increasing along rows.

Since we shall not use Proposition 5.1, we leave its proof (which is an instructive exercise on the definition of conflicts and on the use of the convexity of  $Z$ ) to the reader.  $\square$

**Remark 5.3.** Proposition 5.1 has an analogue for “non-conflicts”: Let  $T$  be a 12-table. Let  $a, b$  and  $c$  be positive integers such that  $(a, c)$  is a conflict of  $T$  and such that  $a < b < c$ . Then, at least one of the pairs  $(a, b)$  and  $(b, c)$  is a conflict of  $T$ . We shall not use this fact, however.

### 5.3. Benign 12-tables and separators

We say that a 12-table  $T$  is *benign* if there exists no conflict  $(i, j)$  of  $T$  such that the  $i$ -th column of  $T$  and the  $j$ -th column of  $T$  both are mixed. (Remember that

columns are sequences.) For instance, the 12-table

|   |   |   |   |   |   |
|---|---|---|---|---|---|
|   |   | 1 | 1 | 2 | 1 |
| 1 | 1 | 1 |   |   |   |
| 1 | 2 | 1 |   |   |   |
| 1 | 2 |   |   |   |   |
| 2 |   |   |   |   |   |

is benign

(despite having  $(2, 3)$  and  $(4, 5)$  as conflicts), while the 12-table

|   |   |   |   |   |   |
|---|---|---|---|---|---|
|   |   | 1 | 1 | 2 | 1 |
| 1 | 1 | 1 |   |   |   |
| 1 | 2 | 1 |   |   |   |
| 1 | 2 | 2 |   |   |   |
| 2 |   |   |   |   |   |

is not (its conflict  $(2, 3)$  has the property that the 2-nd column and the 3-rd column both are mixed). Notice that 12-rpps of shape  $Z$  are benign 12-tables, but the converse is not true.

Let us give an alternative description of benign 12-tables. Namely, if  $T$  is a 12-table, and if  $k \in \mathbb{N}_+$  is such that the  $k$ -th column of  $T$  is mixed, then we define  $\text{sep}_k T$  to be the smallest  $r \in \mathbb{N}_+$  such that  $(r, k) \in Z$  and  $T(r, k) = 2$ .<sup>23</sup> (Speaking visually, the integer  $\text{sep}_k T$  tells us at what row the 1's end<sup>24</sup> and the 2's begin in the  $k$ -th column of  $T$ . Or, more sloppily said, it separates the 1's from the 2's in the  $k$ -th column of  $T$ ; this is why we call it  $\text{sep}_k T$ .) Thus, every 12-table  $T$ , every  $r \in \mathbb{N}_+$  and every  $k \in \mathbb{N}_+$  such that the  $k$ -th column of  $T$  is mixed and such that  $(r, k) \in Z$  satisfy

$$T(r, k) = \begin{cases} 1, & \text{if } r < \text{sep}_k T; \\ 2, & \text{if } r \geq \text{sep}_k T \end{cases} \quad (16)$$

(because the  $k$ -th column of  $T$  is weakly increasing).

<sup>23</sup>Such an  $r$  exists since the  $k$ -th column of  $T$  contains at least one 2 (in fact, it is mixed).

<sup>24</sup>Our use of the words “end” and “begin” always assumes that we are reading the columns of our 12-tables from top to bottom.

If  $T$  is a 12-table, then we let  $\text{seplist } T$  denote the list of all values  $\text{sep}_k T$  (in the order of increasing  $k$ ), where  $k$  ranges over all positive integers for which the  $k$ -th

column of  $T$  is mixed. For instance, if  $T =$ 

|   |   |   |   |   |
|---|---|---|---|---|
|   |   | 1 | 1 | 1 |
|   | 2 | 1 | 1 | 2 |
| 1 | 2 | 1 |   |   |
| 2 | 2 | 2 |   |   |

 $, then  $\text{sep}_1 T = 4$$

(since  $T(1,4) = 2$  and  $T(1,3) = 1$ ), and  $\text{sep}_3 T = 4$ , and  $\text{sep}_5 T = 2$  (and there are no other  $k \in \mathbb{N}_+$  for which  $\text{sep}_k T$  is defined), so that  $\text{seplist } T = (4, 4, 2)$ .

What do the numbers  $\text{sep}_k T$  have to do with being benign?

It is easy to see that if  $T$  is a 12-table, and  $i$  and  $j$  are two positive integers such that the  $i$ -th column of  $T$  and the  $j$ -th column of  $T$  both are mixed, then  $(i, j)$  is a conflict of  $T$  if and only if we have  $i < j$  and  $\text{sep}_i T < \text{sep}_j T$ .

Hence, the definition of a “benign” 12-table rewrites as follows: A 12-table  $T$  is benign if and only if there exists no pair  $(i, j)$  of positive integers such that the  $i$ -th column of  $T$  and the  $j$ -th column of  $T$  both are mixed and such that  $i < j$  and  $\text{sep}_i T < \text{sep}_j T$ . In other words, a 12-table  $T$  is benign if and only if the list  $\text{seplist } T$  is weakly decreasing. We will refer to this fact as the “separational definition of benignity”.

Let  $\mathbf{S}$  denote the set of all benign 12-tables.<sup>25</sup> Then,  $\mathbf{S}$  is a finite set, and we have  $\mathbf{R} \subseteq \mathbf{S}$  (since every 12-rpp of shape  $Z$  is a benign 12-table).

## 5.4. The flip map on benign 12-tables

We define a map  $\text{flip} : \mathbf{S} \rightarrow \mathbf{S}$  as follows: Let  $T \in \mathbf{S}$ ; that is, let  $T$  be a benign 12-table. For every  $k \in \mathbb{N}_+$  for which the  $k$ -th column of  $T$  is nonempty, we transform the  $k$ -th column of  $T$  as follows:

- **If** this column is 1-pure, we replace all its entries by 2’s (so that it becomes 2-pure).
- Otherwise**, if this column is 2-pure, we replace all its entries by 1’s (so that it becomes 1-pure).
- Otherwise** (i.e., if this column is mixed), we do not change it.

Once these transformations are made for all  $k$ , the resulting filling of  $Z$  is a 12-table which is still benign (because its mixed columns are precisely the mixed columns of the original  $T$ ). We define  $\text{flip}(T)$  to be this resulting benign 12-table. Thus, the map  $\text{flip} : \mathbf{S} \rightarrow \mathbf{S}$  is defined.

<sup>25</sup>We recall that  $Z$  is fixed, and all 12-tables have to have  $Z$  as their domain.

For example, if  $T =$ 

|   |   |   |   |   |
|---|---|---|---|---|
|   | 1 | 1 | 2 | 1 |
| 1 | 1 | 1 |   |   |
| 1 | 2 | 1 |   |   |
| 1 | 2 |   |   |   |
| 2 |   |   |   |   |

, then  $\text{flip}(T) =$ 

|   |   |   |   |   |
|---|---|---|---|---|
|   | 1 | 2 | 1 | 2 |
| 1 | 1 | 2 |   |   |
| 1 | 2 | 2 |   |   |
| 1 | 2 |   |   |   |
| 2 |   |   |   |   |

.

The following proposition gathers some easy properties of  $\text{flip}$ :

**Proposition 5.4. (a)** We have  $\text{flip} \circ \text{flip} = \text{id}$  (that is, the map  $\text{flip}$  is an involution).

**(b)** Let  $T$  be a benign 12-table. When  $T$  is transformed into  $\text{flip}(T)$ , the 1-pure columns of  $T$  become 2-pure columns of  $\text{flip}(T)$ , and the 2-pure columns of  $T$  become 1-pure columns of  $\text{flip}(T)$ , while the mixed columns and the empty columns do not change.

**(c)** For every benign 12-table  $T$ , we have

$$\text{ceq}(\text{flip}(T)) = \text{ceq}(T) \quad (17)$$

and

$$\text{ircont}(\text{flip}(T)) = s_1 \cdot \text{ircont}(T). \quad (18)$$

*Proof of Proposition 5.4.* All of Proposition 5.4 is straightforward to prove. (The equality (18) follows from observing that the  $k \in \mathbb{N}_+$  for which the  $k$ -th column of  $\text{flip}(T)$  contains 1 are precisely the  $k \in \mathbb{N}_+$  for which the  $k$ -th column of  $T$  contains 2, and vice versa.)  $\square$

We notice that, when the map  $\text{flip}$  acts on a benign 12-table  $T$ , it transforms every column of  $T$  independently. Thus, we have the following:

**Remark 5.5.** If  $P$  and  $Q$  are two benign 12-tables, and if  $i \in \mathbb{N}_+$  is such that

$$(\text{the } i\text{-th column of } P) = (\text{the } i\text{-th column of } Q),$$

then

$$(\text{the } i\text{-th column of } \text{flip}(P)) = (\text{the } i\text{-th column of } \text{flip}(Q)).$$

## 5.5. Plan of the proof

Let us now briefly sketch the ideas behind the rest of the proof before we go into them in detail. The map  $\text{flip} : \mathbf{S} \rightarrow \mathbf{S}$  does not generally send 12-rpps to 12-rpps (i.e., it does not restrict to a map  $\mathbf{R} \rightarrow \mathbf{R}$ ). However, we shall amend this by defining a way to transform any benign 12-table into a 12-rpp by what we call “resolving conflicts”. The process of “resolving conflicts” will be a stepwise

process, and will be formalized in terms of a binary relation  $\Rightarrow$  on the set  $\mathbf{S}$  which we will soon introduce. The intuition behind saying “ $P \Rightarrow Q$ ” is that the benign 12-table  $P$  has a “resolvable” conflict, resolving which yields the benign 12-table  $Q$ . By “resolvable conflict”, we mean a conflict  $(i, j)$  with  $j = i + 1$ . (The relation  $\Rightarrow$  is similar to the relation  $\Rightarrow$  from Subsection 4.2. “Resolving” a resolvable conflict in a benign 12-table  $P$  is an analogue of switching two adjacent entries of an  $n$ -tuple  $z$  which are out of order.) Starting with a benign 12-table  $P$ , we can repeatedly resolve “resolvable” conflicts until this is no longer possible<sup>26</sup>. We have some freedom in performing this process, because at any step there can be a choice of several resolvable conflicts to resolve; but we will see (using Lemma 4.1) that the final result does not depend on the process. Hence, the final result can be regarded as a function of  $P$ . We will denote it by  $\text{norm } P$ , and we will see that it is a 12-rpp. We will then define a map  $\mathbf{B} : \mathbf{R} \rightarrow \mathbf{R}$  by  $\mathbf{B}(T) = \text{norm}(\text{flip } T)$ , and show that it is an involution satisfying the properties that we want it to satisfy.

## 5.6. Resolving conflicts

Now we come to the details.

Let  $k \in \mathbb{N}_+$ . Let  $P \in \mathbf{S}$ . Thus,  $P$  is a benign 12-table. Assume (for the whole Subsection 5.6) that  $(k, k + 1)$  is a conflict of  $P$ . In this case, we say that  $(k, k + 1)$  is a *resolvable conflict* of  $P$  (and, in a moment, we will explain what it means to “resolve” it). Since  $(k, k + 1)$  is a conflict of  $P$ , it is clear that the  $k$ -th column of  $P$  must contain at least one 2. Hence, the  $k$ -th column of  $P$  is either mixed or 2-pure. Similarly, the  $(k + 1)$ -th column of  $P$  is either mixed or 1-pure. But the  $k$ -th and the  $(k + 1)$ -th columns of  $P$  cannot both be mixed at the same time<sup>27</sup>. Hence, if the  $k$ -th column of  $P$  is mixed, then the  $(k + 1)$ -th column of  $P$  cannot be mixed, and thus this  $(k + 1)$ -th column must be 1-pure<sup>28</sup>. Thus we introduce the following notations:

- We say that the 12-table  $P$  has *k-type M1* if the  $k$ -th column of  $P$  is mixed and the  $(k + 1)$ -th column of  $P$  is 1-pure.
- We say that the 12-table  $P$  has *k-type 2M* if the  $k$ -th column of  $P$  is 2-pure and the  $(k + 1)$ -th column of  $P$  is mixed.

<sup>26</sup>This will eventually happen; i.e., we will eventually reach a state where resolving conflicts will no longer be possible because there will be no resolvable conflicts left. In fact, we will show that if “resolving” a conflict in  $P$  yields a new 12-table  $Q$ , then  $\ell(P) > \ell(Q)$  using the notations of Subsection 5.1; thus, we cannot go on resolving conflicts indefinitely (because the value of  $\ell(T)$  cannot go on decreasing indefinitely). The function  $\ell$  thus plays the same role as the function  $\ell$  in Subsection 4.2.

<sup>27</sup>This is because there exists no conflict  $(i, j)$  of  $P$  such that the  $i$ -th column of  $P$  and the  $j$ -th column of  $P$  both are mixed (since  $P$  is benign), but  $(k, k + 1)$  would be such a conflict if the  $k$ -th and the  $(k + 1)$ -th columns of  $P$  both were mixed.

<sup>28</sup>since the  $(k + 1)$ -th column of  $P$  is either mixed or 1-pure

- We say that the 12-table  $P$  has  $k$ -type 21 if the  $k$ -th column of  $P$  is 2-pure and the  $(k+1)$ -th column of  $P$  is 1-pure.

Then, the 12-table  $P$  always either has  $k$ -type M1, or has  $k$ -type 2M, or has  $k$ -type 21<sup>29</sup>.

(Of course, the names “M1”, “2M”, “21” have been chosen to match the types of the columns: e.g., “2M” stands for “2-pure and Mixed”.)

Now, we define a new 12-table  $\text{res}_k P$  as follows:

- If  $P$  has  $k$ -type M1, then we let  $\text{res}_k P$  be the 12-table defined as follows<sup>30</sup>: The  $k$ -th column of  $\text{res}_k P$  is 1-pure (i.e., it is filled with 1’s); the  $(k+1)$ -th column of  $\text{res}_k P$  is mixed and satisfies  $\text{sep}_{k+1}(\text{res}_k P) = \text{sep}_k P$ ; all other columns of  $\text{res}_k P$  are copied over from  $P$  unchanged.<sup>31</sup>

<sup>29</sup>*Proof.* As we know, the  $k$ -th column of  $P$  is either mixed or 2-pure. If it is 2-pure, then  $P$  must either have  $k$ -type 2M or have  $k$ -type 21 (since the  $(k+1)$ -th column of  $P$  is either mixed or 1-pure). If it is mixed, then the  $(k+1)$ -th column of  $P$  must be 1-pure (as we have seen above), and thus  $P$  must have type M1. In either case, the 12-table  $P$  either has  $k$ -type M1, or has  $k$ -type 2M, or has  $k$ -type 21. Qed.

<sup>30</sup>Here is an example for this definition: If  $P =$

|   |   |   |   |
|---|---|---|---|
|   |   | 1 | 1 |
|   |   | 1 | 2 |
|   | 1 | 1 | 2 |
|   | 1 | 1 |   |
|   | 2 | 1 |   |
| 1 | 2 | 1 |   |
| 2 | 2 |   |   |

conflict of  $P$ , and we have  $\text{sep}_k P = 5$  (since  $P(4, k) = P(4, 2) = 1$  and  $P(5, k) = P(5, 2) = 2$ )

and  $\text{res}_k P =$

|   |   |   |   |
|---|---|---|---|
|   |   | 1 | 1 |
|   |   | 1 | 2 |
|   | 1 | 1 | 2 |
|   | 1 | 1 |   |
|   | 1 | 2 |   |
| 1 | 1 | 2 |   |
| 2 | 1 |   |   |

. The 2’s in the  $(k+1)$ -th column of  $\text{res}_k P$  start in row 5 because

the 2’s in the  $k$ -th column of  $P$  start in row 5; this illustrates the equality  $\text{sep}_{k+1}(\text{res}_k P) = \text{sep}_k P$ .

See Example 5.6 below for another example.

<sup>31</sup>The reader should check that this definition is well-defined: It is clear that the requirements that we are imposing on  $\text{res}_k P$  determine the 12-table  $\text{res}_k P$  uniquely, but it is not immediately obvious why there exists a 12-table  $\text{res}_k P$  which meets these requirements. What could (in theory) go wrong is the requirement that the  $(k+1)$ -th column of  $\text{res}_k P$  be mixed and satisfy  $\text{sep}_{k+1}(\text{res}_k P) = \text{sep}_k P$ . We can try to achieve this by setting

$$(\text{res}_k P)(r, k+1) = \begin{cases} 1, & \text{if } r < \text{sep}_k P; \\ 2, & \text{if } r \geq \text{sep}_k P \end{cases}$$

for all  $r \in \mathbb{N}_+$  for which  $(r, k+1) \in Z$ .

- If  $P$  has  $k$ -type 2M, then we let  $\text{res}_k P$  be the 12-table defined as follows: The  $k$ -th column of  $\text{res}_k P$  is mixed and satisfies  $\text{sep}_k(\text{res}_k P) = \text{sep}_{k+1} P$ ; the  $(k+1)$ -th column of  $\text{res}_k P$  is 2-pure (i.e., it is filled with 2's); all other columns of  $\text{res}_k P$  are copied over from  $P$  unchanged.<sup>32</sup>
- If  $P$  has  $k$ -type 21, then we let  $\text{res}_k P$  be the 12-table defined as follows: The  $k$ -th column of  $\text{res}_k P$  is 1-pure; the  $(k+1)$ -th column of  $\text{res}_k P$  is 2-pure; all other columns of  $\text{res}_k P$  are copied over from  $P$  unchanged.

In either case,  $\text{res}_k P$  is a well-defined 12-table. It is furthermore clear that  $\text{seplist}(\text{res}_k P) = \text{seplist} P$ . Thus, using the “separational definition of benignity”, we see that  $\text{res}_k P$  is benign (since  $P$  is benign); that is,  $\text{res}_k P \in \mathbf{S}$ . We say that  $\text{res}_k P$  is the 12-table obtained by *resolving* the conflict  $(k, k+1)$  in  $P$ . Let us give some examples:

**Example 5.6.** Let  $P =$ 

|   |   |   |   |   |
|---|---|---|---|---|
|   |   | 1 | 2 | 1 |
|   | 1 | 1 | 2 |   |
| 2 | 1 | 1 |   |   |
| 2 | 2 | 1 |   |   |
| 2 |   |   |   |   |

. Then,  $P$  is a benign 12-table (with

only one mixed column), and its conflicts are  $(1, 2)$ ,  $(1, 3)$ ,  $(2, 3)$  and  $(4, 5)$ . Out of these conflicts,  $(1, 2)$ ,  $(2, 3)$  and  $(4, 5)$  are resolvable (as they have the form  $(k, k+1)$  for various  $k$ ). We have  $\text{sep}_2 P = 4$ .

If we set  $k = 1$ , then  $P$  has  $k$ -type 2M, and resolving the conflict  $(k, k+1) =$

$(1, 2)$  gives us the 12-table  $\text{res}_1 P =$ 

|   |   |   |   |   |
|---|---|---|---|---|
|   |   | 1 | 2 | 1 |
|   | 2 | 1 | 2 |   |
| 1 | 2 | 1 |   |   |
| 2 | 2 | 1 |   |   |
| 2 |   |   |   |   |

.

If we instead set  $k = 2$ , then  $P$  has  $k$ -type M1, and resolving the conflict

$(k, k+1) = (2, 3)$  gives us the 12-table  $\text{res}_2 P =$ 

|   |   |   |   |   |
|---|---|---|---|---|
|   |   | 1 | 2 | 1 |
|   | 1 | 1 | 2 |   |
| 2 | 1 | 1 |   |   |
| 2 | 1 | 2 |   |   |
| 2 |   |   |   |   |

.

This (together with the requirements on the other columns) defines a 12-table  $\text{res}_k P$ , but we still need to check that the  $(k+1)$ -th column of the 12-table  $\text{res}_k P$  constructed in this way is actually mixed. To check this, the reader should verify that both cells  $(\text{sep}_k P, k+1)$  and  $(\text{sep}_k P + 1, k+1)$  belong to  $Z$  (here it is necessary to invoke the convexity of  $Z$  and the existence of the conflict  $(k, k+1)$  in  $P$ ), and that these cells have entries 1 and 2 in  $\text{res}_k P$ , respectively.

<sup>32</sup>Again, it is easy to see that this is well-defined.

If we instead set  $k = 4$ , then  $P$  has  $k$ -type 21, and resolving the conflict

$$(k, k+1) = (4, 5) \text{ gives us the 12-table } \text{res}_4 P = \begin{array}{|c|c|c|} \hline & 1 & 1 & 2 \\ \hline & 1 & 1 & 1 \\ \hline 2 & 1 & 1 & \\ \hline 2 & 2 & 1 & \\ \hline 2 & & & \\ \hline \end{array}.$$

We notice that each of the three 12-tables  $\text{res}_1 P$ ,  $\text{res}_2 P$  and  $\text{res}_4 P$  still has conflicts<sup>33</sup>, and again some of these conflicts are resolvable. In order to get a 12-rpp from  $P$ , we will have to keep resolving these conflicts until none remain.

We now observe some further properties of  $\text{res}_k P$ :

**Proposition 5.7.** Let  $P \in \mathbf{S}$  and  $k \in \mathbb{N}_+$  be such that  $(k, k+1)$  is a conflict of  $P$ .

(a) The 12-table  $\text{res}_k P$  differs from  $P$  only in columns  $k$  and  $k+1$ . In other words,

$$(\text{the } h\text{-th column of } \text{res}_k P) = (\text{the } h\text{-th column of } P) \quad (19)$$

for every  $h \in \mathbb{N}_+ \setminus \{k, k+1\}$ .

(b) The  $k$ -th and the  $(k+1)$ -th columns of  $\text{res}_k P$  depend only on the  $k$ -th and the  $(k+1)$ -th columns of  $P$ . In other words, if  $Q$  is a further benign 12-table satisfying

$$\begin{aligned} (\text{the } h\text{-th column of } Q) &= (\text{the } h\text{-th column of } P) \\ &\text{for each } h \in \{k, k+1\}, \end{aligned}$$

then  $(k, k+1)$  is a conflict of  $Q$  and we have

$$\begin{aligned} (\text{the } h\text{-th column of } \text{res}_k Q) &= (\text{the } h\text{-th column of } \text{res}_k P) \\ &\text{for each } h \in \{k, k+1\}. \end{aligned} \quad (20)$$

(c) We have

$$\text{ceq}(\text{res}_k P) = \text{ceq}(P). \quad (21)$$

(d) We have

$$\begin{aligned} &(\text{the number of } h \in \mathbb{N}_+ \text{ such that the } h\text{-th column of } \text{res}_k P \text{ is mixed}) \\ &= (\text{the number of } h \in \mathbb{N}_+ \text{ such that the } h\text{-th column of } P \text{ is mixed}), \end{aligned} \quad (22)$$

<sup>33</sup>Actually, each of these three 12-tables has fewer conflicts than  $P$  (in particular, the conflict that

was resolved is now gone). But this does not generalize. For instance, if  $P = \begin{array}{|c|c|} \hline 1 & 1 \\ \hline 2 & 1 \\ \hline \end{array}$  and

$k = 1$ , then resolving the conflict  $(k, k+1) = (1, 2)$  (which is the only conflict of  $P$ ) leads to

the 12-table  $\text{res}_1 P = \begin{array}{|c|c|} \hline 2 & 1 \\ \hline 1 & 2 \\ \hline \end{array}$ , which has as many conflicts as  $P$  did.



$$\begin{aligned} & (\text{the number of } h \in \mathbb{N}_+ \text{ such that the } h\text{-th column of } \text{res}_k P \text{ is 1-pure}) \\ &= (\text{the number of } h \in \mathbb{N}_+ \text{ such that the } h\text{-th column of } P \text{ is 1-pure}), \end{aligned} \quad (23)$$

$$\begin{aligned} & (\text{the number of } h \in \mathbb{N}_+ \text{ such that the } h\text{-th column of } \text{res}_k P \text{ is 2-pure}) \\ &= (\text{the number of } h \in \mathbb{N}_+ \text{ such that the } h\text{-th column of } P \text{ is 2-pure}), \end{aligned} \quad (24)$$

and

$$\text{ircont}(\text{res}_k P) = \text{ircont}(P). \quad (25)$$

(e) For every  $r \in \mathbb{N}_+$  and  $i \in \mathbb{N}_+$  satisfying  $(r, i) \in Z$  and  $(r, s_k(i)) \in Z$ , we have

$$P(r, i) = (\text{res}_k P)(r, s_k(i)). \quad (26)$$

(f) If  $(i, j)$  is a conflict of  $P$  such that  $(i, j) \neq (k, k+1)$ , then

$$(s_k(i), s_k(j)) \text{ is a conflict of } \text{res}_k P. \quad (27)$$

(g) The benign 12-tables  $\text{flip}(P)$  and  $\text{flip}(\text{res}_k P)$  have the property that

$$\left( \begin{array}{l} (k, k+1) \text{ is a conflict of } \text{flip}(\text{res}_k P), \\ \text{and we have } \text{flip}(P) = \text{res}_k(\text{flip}(\text{res}_k P)) \end{array} \right). \quad (28)$$

(h) Recall that we defined a nonnegative integer  $\ell(T)$  for every 12-table  $T$  in Subsection 5.1. We have

$$\ell(P) > \ell(\text{res}_k P). \quad (29)$$

Notice that the converse of Proposition 5.7 (f) does not generally hold.

*Proof of Proposition 5.7.* Most of Proposition 5.7 succumbs to straightforward arguments using the definitions of  $\text{res}_k$  and  $\text{flip}$  coupled with a thorough case analysis, with an occasional use of the convexity of  $Z$  and of the formula (16). Merely the parts (c) and (f) require a bit more thinking. We shall only give the proof for part (c), since part (f) will not be used in the following.

(c) A cell  $(i, j)$  in  $Z$  will be called *good* if the cell  $(i+1, j)$  also belongs to  $Z$ . Notice that every redundant cell of  $P$  or of  $\text{res}_k P$  must be good.

In order to prove (21), we need to show that, for every  $r \in \mathbb{N}_+$ , the number of redundant cells of  $P$  in row  $r$  equals the number of redundant cells of  $\text{res}_k P$  in row  $r$ . Instead of comparing the numbers of redundant cells, we can just as well compare the numbers of good cells that are not redundant (because all redundant cells are good, and because the total number of good cells clearly depends only on  $Z$  and not on the 12-table). So we need to show that, for every  $r \in \mathbb{N}_+$ , the number of good cells in row  $r$  that are not redundant cells of  $P$  equals the number of good cells in row  $r$  that are not redundant cells of  $\text{res}_k P$ .

Fix  $r \in \mathbb{N}_+$ . The number of good cells in row  $r$  that are not redundant cells of  $P$  is precisely the number of appearances of  $r + 1$  in the list  $\text{seplist } P$  (because the good cells that are not redundant cells of  $P$  are precisely the cells of the form  $(\text{sep}_k P, k)$ , where  $k$  is a positive integer such that the  $k$ -th column of  $P$  is mixed). Similarly, the number of good cells in row  $r$  that are not redundant cells of  $\text{res}_k P$  is precisely the number of appearances of  $r + 1$  in the list  $\text{seplist } (\text{res}_k P)$ . These two numbers are equal, because  $\text{seplist } (\text{res}_k P) = \text{seplist } P$ . As explained above, this completes the proof of (21).  $\square$

## 5.7. The conflict-resolution relation $\Rightarrow$

**Definition 5.8.** Let us now define a binary relation  $\Rightarrow$  on the set  $\mathbf{S}$  as follows: Let  $P \in \mathbf{S}$  and  $Q \in \mathbf{S}$ . If  $k \in \mathbb{N}_+$ , then we write  $P \Rightarrow_k Q$  if and only if  $(k, k + 1)$  is a conflict of  $P$  and we have  $Q = \text{res}_k P$ . (In other words, if  $k \in \mathbb{N}_+$ , then we write  $P \Rightarrow_k Q$  if and only if  $(k, k + 1)$  is a conflict of  $P$  and the 12-table  $Q$  is obtained from  $P$  by resolving this conflict.) We write  $P \Rightarrow Q$  if and only if there exists a  $k \in \mathbb{N}_+$  such that  $P \Rightarrow_k Q$ . (In other words, we write  $P \Rightarrow Q$  if and only if the 12-table  $Q$  is obtained from  $P$  by resolving a conflict of the form  $(k, k + 1)$  with  $k \in \mathbb{N}_+$ .) Thus, the relation  $\Rightarrow$  is defined.

Some of what was shown above translates into properties of this relation  $\Rightarrow$ :

**Lemma 5.9.** Let  $P \in \mathbf{S}$  and  $Q \in \mathbf{S}$  be such that  $P \Rightarrow Q$ . Then:

- (a) We have  $\text{ceq}(Q) = \text{ceq}(P)$ .
- (b) We have  $\text{ircont}(Q) = \text{ircont}(P)$ .
- (c) The benign 12-tables  $\text{flip}(P)$  and  $\text{flip}(Q)$  have the property that  $\text{flip}(Q) \Rightarrow \text{flip}(P)$ .
- (d) We have  $\ell(P) > \ell(Q)$ .

*Proof of Lemma 5.9.* We have  $P \Rightarrow Q$ . In other words, there exists a  $k \in \mathbb{N}_+$  such that  $P \Rightarrow_k Q$ . Consider this  $k$ . We have  $P \Rightarrow_k Q$ . In other words,  $(k, k + 1)$  is a conflict of  $P$  and we have  $Q = \text{res}_k P$ .

- (a) We have  $\text{ceq}\left(\underbrace{Q}_{=\text{res}_k P}\right) = \text{ceq}(\text{res}_k P) = \text{ceq}(P)$  (by (21)). This proves

Lemma 5.9 (a).

- (b) This follows similarly from (25).

(c) From (28), we know that  $(k, k + 1)$  is a conflict of  $\text{flip}(\text{res}_k P)$ , and we have  $\text{flip}(P) = \text{res}_k(\text{flip}(\text{res}_k P))$ . In other words,  $\text{flip}(\text{res}_k P) \Rightarrow_k \text{flip}(P)$ . Thus,  $\text{flip}(\text{res}_k P) \Rightarrow \text{flip}(P)$ . In other words,  $\text{flip}(Q) \Rightarrow \text{flip}(P)$  (since  $Q = \text{res}_k P$ ). This proves Lemma 5.9 (c).

(d) From (29), we have  $\ell(P) > \ell\left(\underbrace{\text{res}_k P}_{=Q}\right) = \ell(Q)$ . This proves Lemma 5.9

(d). □

We furthermore define a relation  $\Rightarrow^*$  as in Lemma 4.1. In other words,  $\Rightarrow^*$  is the reflexive-and-transitive closure of the relation  $\Rightarrow$ . In particular, the relation  $\Rightarrow^*$  is reflexive and transitive, and extends the relation  $\Rightarrow$ .

If  $P \in \mathbf{S}$  and  $Q \in \mathbf{S}$ , then the relation “ $P \Rightarrow^* Q$ ” can be interpreted as “ $Q$  can be obtained from  $P$  by repeatedly resolving conflicts” (because  $P \Rightarrow Q$  holds if and only if  $Q$  is obtained from  $P$  by resolving a resolvable conflict).

It is easy to derive from Lemma 5.9 the following fact:

**Lemma 5.10.** Let  $P \in \mathbf{S}$  and  $Q \in \mathbf{S}$  be such that  $P \Rightarrow^* Q$ . Then:

(a) We have  $\text{ceq}(Q) = \text{ceq}(P)$ .

(b) We have  $\text{ircont}(Q) = \text{ircont}(P)$ .

(c) The benign 12-tables  $\text{flip}(P)$  and  $\text{flip}(Q)$  have the property that  $\text{flip}(Q) \Rightarrow^* \text{flip}(P)$ .

*Proof of Lemma 5.10.* Recalling that  $\Rightarrow^*$  is the reflexive-and-transitive closure of the relation  $\Rightarrow$ , we see that Lemma 5.10 follows by induction using Lemma 5.9. □

In Subsection 5.1, we defined a nonnegative integer  $\ell(T)$  for every 12-table  $T$ . In particular,  $\ell(T)$  is defined for every  $T \in \mathbf{S}$ . We thus have a map  $\ell : \mathbf{S} \rightarrow \mathbb{N}$  which sends every  $T \in \mathbf{S}$  to  $\ell(T)$ .

Our goal is now to apply Lemma 4.1 to our set  $\mathbf{S}$ , our map  $\ell$  and our relation  $\Rightarrow$ . In order to do so, we need to check the following fact:

**Proposition 5.11.** The local confluence hypothesis and the length-decrease hypothesis are satisfied for our set  $\mathbf{S}$ , our map  $\ell$  and our relation  $\Rightarrow$ . (See Lemma 4.1 for the statements of these two hypotheses.)

*Proof of Proposition 5.11.* The length-decrease hypothesis is clearly satisfied (indeed, it is just Lemma 5.9 (d), with  $P$  and  $Q$  renamed as  $a$  and  $b$ ). It thus remains only to prove that the local confluence hypothesis is satisfied. In other words, it remains to prove that if  $a, b$  and  $c$  are three elements of  $\mathbf{S}$  satisfying  $a \Rightarrow b$  and  $a \Rightarrow c$ , then there exists a  $d \in \mathbf{S}$  such that  $b \Rightarrow^* d$  and  $c \Rightarrow^* d$ . Let us rename the bound variables  $a, b, c$  and  $d$  as  $A, B, C$  and  $D$  in this sentence. Thus, it remains to prove that if  $A, B$  and  $C$  are three elements of  $\mathbf{S}$  satisfying  $A \Rightarrow B$  and  $A \Rightarrow C$ , then there exists a  $D \in \mathbf{S}$  such that  $B \Rightarrow^* D$  and  $C \Rightarrow^* D$ .

So let  $A, B$  and  $C$  be three elements of  $\mathbf{S}$  satisfying  $A \Rightarrow B$  and  $A \Rightarrow C$ . We need to prove that there exists a  $D \in \mathbf{S}$  such that  $B \Rightarrow^* D$  and  $C \Rightarrow^* D$ . If  $B = C$ ,

then we can simply choose  $D = B = C$  and be done with it; thus, we WLOG assume that  $B \neq C$ .

We have  $A \Rightarrow B$ . In other words, there exists a  $k \in \mathbb{N}_+$  such that  $A \xRightarrow[k]{\quad} B$ . Let us denote this  $k$  by  $u$ . Thus,  $A \xRightarrow[u]{\quad} B$ . In other words,  $(u, u+1)$  is a conflict of  $A$  and we have  $B = \text{res}_u A$  (due to the definition of " $A \xRightarrow[u]{\quad} B$ "). Similarly, we can find a  $v \in \mathbb{N}_+$  such that  $(v, v+1)$  is a conflict of  $A$  and we have  $C = \text{res}_v A$ . Consider this  $v$  as well.

We have  $\text{res}_u A = B \neq C = \text{res}_v A$  and thus  $u \neq v$ . Hence, either  $u < v$  or  $u > v$ . We WLOG assume that  $u < v$  (since otherwise, we can simply switch  $u$  with  $v$ ). Hence, we are in one of the following two Cases:

*Case 1:* We have  $u = v - 1$ .

*Case 2:* We have  $u < v - 1$ .

Let us deal with Case 2 first (since it is the simpler of the two). In this case,  $u < v - 1$ , so that  $\{u, u+1\} \cap \{v, v+1\} = \emptyset$ .

Now, the operation of resolving the conflict  $(u, u+1)$  in  $A$  (that is, the passage from  $A$  to  $\text{res}_u A$ ) only affects the columns  $u$  and  $u+1$ , and thus it preserves the conflict  $(v, v+1)$  (since  $\{u, u+1\} \cap \{v, v+1\} = \emptyset$ ). Hence,  $\text{res}_v(\text{res}_u A)$  is well-defined. Similarly,  $\text{res}_u(\text{res}_v A)$  is well-defined.

Recall again that  $\{u, u+1\} \cap \{v, v+1\} = \emptyset$ . Thus, the operation of resolving the conflict  $(u, u+1)$  and the operation of resolving the conflict  $(v, v+1)$  "do not interact" (in the sense that the former only changes the columns  $u$  and  $u+1$ , and changes them in a way that does not depend on any of the other columns; and similarly for the latter). Therefore, the two operations can be applied one after the other in any order; the results will be the same. In other words,  $\text{res}_u(\text{res}_v A) = \text{res}_v(\text{res}_u A)$ . Now, set  $D = \text{res}_u(\text{res}_v A) = \text{res}_v(\text{res}_u A)$ . Then,  $D = \text{res}_u(\underbrace{\text{res}_v A}_{=C}) = \text{res}_u C$  and thus  $C \xRightarrow[u]{\quad} D$ , so that  $C \Rightarrow D$ , therefore

$C \xRightarrow{*} D$ . Similarly,  $B \xRightarrow{*} D$ . Hence, we have found a  $D \in \mathbf{S}$  such that  $B \xRightarrow{*} D$  and  $C \xRightarrow{*} D$ . This completes the proof of the local confluence hypothesis in Case 2.

Now, let us consider Case 1. In this case,  $u = v - 1$ . Hence,  $(v - 1, v)$  is a conflict of  $A$  (since  $(u, u+1)$  is a conflict of  $A$ ), and we have  $B = \text{res}_u A = \text{res}_{v-1} A$  (since  $u = v - 1$ ).

The  $v$ -th column of  $A$  must contain a 1 (since  $(v - 1, v)$  is a conflict of  $A$ ) and a 2 (since  $(v, v+1)$  is a conflict of  $A$ ). Hence, the  $v$ -th column of  $A$  is mixed. The  $(v - 1)$ -th column of  $A$  is 2-pure<sup>34</sup>, and the  $(v + 1)$ -th column of  $A$  is 1-pure<sup>35</sup>.

<sup>34</sup>*Proof.* Assume the contrary. Then, the  $(v - 1)$ -th column of  $A$  contains a 2 (because  $(v - 1, v)$  is a conflict of  $A$ ) but is not 2-pure. Hence, this column is mixed. But  $A$  is benign. In other words, there exists no conflict  $(i, j)$  of  $A$  such that the  $i$ -th column of  $A$  and the  $j$ -th column of  $A$  both are mixed. This flies in the face of the fact that  $(v - 1, v)$  is exactly such a conflict (since both the  $(v - 1)$ -th and the  $v$ -th columns of  $A$  are mixed). This contradiction proves that our assumption was wrong, qed.

<sup>35</sup>This follows similarly.

We can thus semiotically represent the 12-table  $A$  as follows:

$$A = \begin{array}{|c|c|c|} \hline & 1 & 1 \\ \hline 2 & & \\ \hline & 2 & \\ \hline \end{array}. \quad (30)$$

In this representation, we only draw the  $(v-1)$ -th, the  $v$ -th and the  $(v+1)$ -th columns (since the remaining columns are neither used nor changed by  $\text{res}_{v-1}$  and  $\text{res}_v$ , and thus are irrelevant to our argument); we use a rectangle with a “1” inside to signify a string of 1’s in a column<sup>36</sup>, and we use a rectangle with a “2” inside to signify a string of 2’s in a column.

Let  $s = \text{sep}_v A$ . Then,  $(s, v)$  and  $(s+1, v)$  belong to  $Z$  and satisfy  $A(s, v) = 1$  and  $A(s+1, v) = 2$  (by the definition of  $\text{sep}_v A$ ). Also,  $(s, v-1)$  must belong to  $Z$ <sup>37</sup>. Hence,  $(s+1, v-1)$  must belong to  $Z$  as well<sup>38</sup>. Similarly,  $(s+1, v+1)$  and  $(s, v+1)$  belong to  $Z$ . Altogether, we thus know that all six squares  $(s, v)$ ,  $(s+1, v)$ ,  $(s, v-1)$ ,  $(s+1, v-1)$ ,  $(s+1, v+1)$  and  $(s, v+1)$  belong to  $Z$ . We shall denote these six squares as the “core squares”. The restriction of  $A$  to the

core squares is 

|   |   |   |
|---|---|---|
| 2 | 1 | 1 |
| 2 | 2 | 1 |

<sup>39</sup>.

Now,  $A$  has  $(v-1)$ -type 2M, and resolving the conflict  $(v-1, v)$  of  $A$  yields  $\text{res}_{v-1} A = B$ . Hence,  $B$  is represented semiotically as follows:

$$B = \begin{array}{|c|c|c|} \hline & & 1 \\ \hline 1 & 2 & \\ \hline & & \\ \hline 2 & & \\ \hline \end{array},$$

<sup>36</sup>The length of the rectangle is immaterial; it does not say anything about the number of 1’s.

<sup>37</sup>*Proof.* We know that  $(v-1, v)$  is a conflict of  $A$ . Hence, there exists an  $r \in \mathbb{N}_+$  such that  $(r, v-1) \in Z$ ,  $(r, v) \in Z$ ,  $A(r, v-1) = 2$  and  $A(r, v) = 1$ . Consider this  $r$ . If we had  $s+1 \leq r$ , then we would have  $A(s+1, v) \leq A(r, v)$  (since the entries of  $A$  are weakly decreasing down columns), which would contradict  $A(r, v) = 1 < 2 = A(s+1, v)$ . Therefore, we cannot have  $s+1 \leq r$ . Hence,  $r < s+1$ , so that  $r \leq s$ . Hence, (1) (applied to  $r, s, s, v-1, v-1$  and  $v$  instead of  $i, i', i'', j, j'$  and  $j''$ ) yields  $(s, v-1) \in Z$ , qed.

<sup>38</sup>by (1) (applied to  $s, s+1, s+1, v-1, v-1$  and  $v$  instead of  $i, i', i'', j, j'$  and  $j''$ )

<sup>39</sup>Indeed, the two core squares in the  $v$ -th column have entries  $A(s, v) = 1$  and  $A(s+1, v) = 2$ ; the two core squares in the  $(v-1)$ -th column have entries 2 (since the  $(v-1)$ -th column of  $A$  is 2-pure); and the two core squares in the  $(v+1)$ -th column have entries 1 (since the  $(v+1)$ -th column of  $A$  is 1-pure).

and the restriction of  $B$  to the core squares is  $\begin{array}{|c|c|c|} \hline 1 & 2 & 1 \\ \hline 2 & 2 & 1 \\ \hline \end{array}$ . This shows that  $(v, v+1)$  is a conflict of  $B$ , and that  $B$  has  $v$ -type 21. Hence, resolving this conflict in  $B$  yields a 12-table  $\text{res}_v B$  which is represented semiotically as follows:

$$\text{res}_v B = \begin{array}{|c|c|c|} \hline & & \\ \hline 1 & 1 & 2 \\ \hline 2 & & \\ \hline \end{array},$$

and the restriction of  $\text{res}_v B$  to the core squares is  $\begin{array}{|c|c|c|} \hline 1 & 1 & 2 \\ \hline 2 & 1 & 2 \\ \hline \end{array}$ . This, in turn, shows that  $(v-1, v)$  is a conflict of  $\text{res}_v B$ , and that  $\text{res}_v B$  has  $(v-1)$ -type M1. Thus, resolving this conflict in  $\text{res}_v B$  yields a 12-table  $\text{res}_{v-1}(\text{res}_v B)$  which is represented semiotically as follows:

$$\text{res}_{v-1}(\text{res}_v B) = \begin{array}{|c|c|c|} \hline & & \\ \hline 1 & 1 & 2 \\ \hline & 2 & \\ \hline \end{array}, \quad (31)$$

and the restriction of  $\text{res}_{v-1}(\text{res}_v B)$  to the core squares is  $\begin{array}{|c|c|c|} \hline 1 & 1 & 2 \\ \hline 1 & 2 & 2 \\ \hline \end{array}$ .

On the other hand,  $A$  has  $v$ -type M1. Resolving the conflict  $(v, v+1)$  of  $A$  yields  $\text{res}_v A = C$ . Thus, we can represent  $C$  semiotically and find its restriction to the core squares. This shows us that  $C$  has  $(v-1, v)$  as a conflict and has  $(v-1)$ -type 21. Resolving this conflict yields a 12-table  $\text{res}_{v-1} C$  which we can again represent semiotically and find its restriction to the core squares. Doing this, we observe that  $\text{res}_{v-1} C$  has  $(v, v+1)$  as a conflict and has  $v$ -type 2M. Resolving this conflict yields a 12-table  $\text{res}_v(\text{res}_{v-1} C)$  whose semiotic representation and restriction to the core squares can again be found. We leave the details of this argument to the reader, but we state its result: The 12-table  $\text{res}_v(\text{res}_{v-1} C)$  is well-defined and has the same semiotic representation and the same restriction to the core squares as the 12-table  $\text{res}_{v-1}(\text{res}_v B)$ . Consequently,

the 12-tables  $\text{res}_v(\text{res}_{v-1} C)$  and  $\text{res}_{v-1}(\text{res}_v B)$  are equal<sup>40</sup>.

Hence, we can set  $D = \text{res}_v(\text{res}_{v-1} C) = \text{res}_{v-1}(\text{res}_v B)$ . Consider this  $D$ . We have  $C \Rightarrow \text{res}_{v-1} C$  (since  $C \Rightarrow_{v-1} \text{res}_{v-1} C$ ) and  $\text{res}_{v-1} C \Rightarrow \text{res}_v(\text{res}_{v-1} C)$  (since  $\text{res}_{v-1} C \Rightarrow_v \text{res}_v(\text{res}_{v-1} C)$ ). Combining these two relations, we obtain  $C \xRightarrow{*} \text{res}_v(\text{res}_{v-1} C)$  (since  $\xRightarrow{*}$  is the reflexive-and-transitive closure of the relation  $\Rightarrow$ ). In other words,  $C \xRightarrow{*} D$  (since  $D = \text{res}_v(\text{res}_{v-1} C)$ ). Similarly,  $B \xRightarrow{*} D$ . Thus, we have found a  $D \in \mathbf{S}$  such that  $B \xRightarrow{*} D$  and  $C \xRightarrow{*} D$ . This completes the proof of the local confluence hypothesis in Case 1.

Now, the local confluence hypothesis is proven (since we have shown it in both Cases 1 and 2), and with it, Proposition 5.11.  $\square$

Now, let us define the notion of a “final” element of  $\mathbf{S}$  as in Lemma 4.1. Then, the following is almost obvious:

**Proposition 5.12.** Let  $P \in \mathbf{S}$ . Then, the element  $P$  of  $\mathbf{S}$  is final if and only if  $P$  is a 12-rpp.

*Proof of Proposition 5.12.* Let us first assume that  $P$  is final. We shall show that  $P$  is a 12-rpp.

Indeed, assume the contrary. Then,  $P$  is not a 12-rpp. But  $P$  is an element of  $\mathbf{S}$ , thus a benign 12-table. The entries of  $P$  are weakly increasing down columns (since  $P$  is a 12-table). Thus, the entries of  $P$  are not weakly increasing along rows (because otherwise,  $P$  would be a 12-rpp). In other words, there exists an  $r \in \mathbb{N}_+$  such that the  $r$ -th row of  $P$  is not weakly increasing. Consider this  $r$ . The  $r$ -th row of  $P$  is not weakly increasing; hence, there exist two adjacent entries of

<sup>40</sup>*Proof.* To see this, we need to show that for every  $h \in \mathbb{N}_+$ , the  $h$ -th column of  $\text{res}_v(\text{res}_{v-1} C)$  equals the  $h$ -th column of  $\text{res}_{v-1}(\text{res}_v B)$ .

For  $h \notin \{v-1, v, v+1\}$ , this is obvious (because for  $h \notin \{v-1, v, v+1\}$ , the  $h$ -th column of a 12-table never changes under  $\text{res}_v$  or  $\text{res}_{v-1}$ ).

For  $h = v-1$ , this is again obvious (because the semiotic representation of  $\text{res}_{v-1}(\text{res}_v B)$  given in (31) shows that the  $(v-1)$ -th column of  $\text{res}_{v-1}(\text{res}_v B)$  is 1-pure, and the same can be said of the  $(v-1)$ -th column of  $\text{res}_v(\text{res}_{v-1} C)$ ).

For  $h = v+1$ , this is also obvious (because the semiotic representation of  $\text{res}_{v-1}(\text{res}_v B)$  given in (31) shows that the  $(v+1)$ -th column of  $\text{res}_{v-1}(\text{res}_v B)$  is 2-pure, and the same can be said of the  $(v+1)$ -th column of  $\text{res}_v(\text{res}_{v-1} C)$ ).

It thus only remains to deal with the case of  $h = v$ . In other words, we need to prove that the  $v$ -th column of  $\text{res}_v(\text{res}_{v-1} C)$  equals the  $v$ -th column of  $\text{res}_{v-1}(\text{res}_v B)$ .

We know from (31) that the  $v$ -th column of  $\text{res}_{v-1}(\text{res}_v B)$  is mixed. Moreover, the restric-

tion of  $\text{res}_{v-1}(\text{res}_v B)$  to the core squares is  $\begin{bmatrix} 1 & 1 & 2 \\ 1 & 2 & 2 \end{bmatrix}$ ; therefore, the last 1 and the first 2

in the  $v$ -th column of  $\text{res}_{v-1}(\text{res}_v B)$  are in the cells  $(s, v)$  and  $(s+1, v)$ , respectively. But the same can be said about the  $v$ -th column of  $\text{res}_v(\text{res}_{v-1} C)$ . Hence, the  $v$ -th column of  $\text{res}_v(\text{res}_{v-1} C)$  and the  $v$ -th column of  $\text{res}_{v-1}(\text{res}_v B)$  both are mixed, and the cell containing the last 1 is the same for both of these columns. This yields that these columns must be equal. As we know, this finishes our proof.

this row such that the left one is larger than the right one. In other words, there exists a  $k \in \mathbb{N}_+$  such that  $(r, k) \in Z$ ,  $(r, k+1) \in Z$  and  $P(r, k) > P(r, k+1)$ . Consider this  $k$ . Both  $P(r, k)$  and  $P(r, k+1)$  belong to  $\{1, 2\}$ . Hence, from  $P(r, k) > P(r, k+1)$ , we obtain  $P(r, k) = 2$  and  $P(r, k+1) = 1$ . Therefore,  $(k, k+1)$  is a conflict of  $P$  (due to the definition of a “conflict”). Consequently,  $\text{res}_k P$  is well-defined, and we have  $P \Rightarrow_k \text{res}_k P$  (due to the definition of “ $P \Rightarrow_k \text{res}_k P$ ”), so that  $P \Rightarrow \text{res}_k P$  (due to the definition of the relation  $\Rightarrow$ ).

But recall that  $P$  is final. In other words, there exists no  $b \in \mathbf{S}$  satisfying  $P \Rightarrow b$  (according to the definition of “final”). This contradicts the fact that  $\text{res}_k P$  is such a  $b$  (since  $P \Rightarrow \text{res}_k P$  and  $\text{res}_k P \in \mathbf{S}$ ). This contradiction proves that our assumption was wrong. So we have shown that  $P$  is a 12-rpp.

Now, let us forget that we assumed that  $P$  is final. Thus, we have proven that if  $P$  is final, then  $P$  is a 12-rpp. It remains to prove the converse. In other words, it remains to prove that if  $P$  is a 12-rpp, then  $P$  is final.

So let us assume that  $P$  is a 12-rpp. Let  $b \in \mathbf{S}$  be such that  $P \Rightarrow b$ . Then, there exists a  $k \in \mathbb{N}_+$  such that  $P \Rightarrow_k b$  (by the definition of the relation  $\Rightarrow$ ). Consider this  $k$ . We have  $P \Rightarrow_k b$ . In other words,  $(k, k+1)$  is a conflict of  $P$  and we have  $b = \text{res}_k P$ . But  $P$  is a 12-rpp of shape  $Z$ , and thus has no conflicts (since a 12-rpp of shape  $Z$  is the same as a 12-table which has no conflicts). So  $(k, k+1)$  is a conflict of  $P$ , but  $P$  has no conflicts. This is a contradiction.

Now, let us forget that we fixed  $b$ . We thus have found a contradiction for every  $b \in \mathbf{S}$  satisfying  $P \Rightarrow b$ . Hence, there exists no  $b \in \mathbf{S}$  satisfying  $P \Rightarrow b$ . In other words,  $P$  is final (according to the definition of “final”). This completes our proof of Proposition 5.12.  $\square$

## 5.8. The normalization map

**Definition 5.13.** We now define a map  $\text{norm} : \mathbf{S} \rightarrow \mathbf{R}$  as follows:

Let  $T \in \mathbf{S}$ . Proposition 5.11 shows that the local confluence hypothesis and the length-decrease hypothesis are satisfied for our set  $\mathbf{S}$ , our map  $\ell$  and our relation  $\Rightarrow$ . Thus, Lemma 4.1 shows that for every  $a \in \mathbf{S}$ , there exists a unique final element  $b \in \mathbf{S}$  such that  $a \Rightarrow^* b$ . Applying this to  $a = T$ , we conclude that there exists a unique final element  $b \in \mathbf{S}$  such that  $T \Rightarrow^* b$ . Denote this  $b$  by  $P$ . Then,  $P$  is a final element of  $\mathbf{S}$  and satisfies  $T \Rightarrow^* P$ . But Proposition 5.12 shows that  $P$  is final if and only if  $P$  is a 12-rpp. Hence,  $P$  is a 12-rpp (since  $P$  is final). In other words,  $P \in \mathbf{R}$  (since  $\mathbf{R}$  is the set of all 12-rpps). We define  $\text{norm}(T)$  to be  $P$ .

Thus, for every  $T \in \mathbf{S}$ , we have defined  $\text{norm}(T)$  to be the unique final element  $b \in \mathbf{S}$  such that  $T \Rightarrow^* b$ . As a consequence, for every  $T \in \mathbf{S}$ , we have

$$T \Rightarrow^* \text{norm}(T). \quad (32)$$



Thus, the map  $\text{norm} : \mathbf{S} \rightarrow \mathbf{R}$  is defined.

**Example 5.14.** Let us give an example of a computation of  $\text{norm}(T)$ . For this example, let us take

$$T = \begin{array}{ccccc} & & & 1 & 2 & 1 \\ & & & 1 & 1 & 2 \\ & 2 & 1 & 1 & & \\ & 2 & 2 & 1 & & \\ & 2 & & & & \end{array} .$$

Then,  $\text{norm}(T)$  is the unique final element  $b \in \mathbf{S}$  such that  $T \xRightarrow{*} b$ . Thus, we can obtain  $\text{norm}(T)$  from  $T$  by repeatedly resolving conflicts until no more conflicts are left (because “ $T \xRightarrow{*} b$ ” means “ $b$  can be obtained from  $T$  by repeatedly resolving conflicts”). The word “unique” here implies that, in whatever order we resolve conflicts, the result will always be the same. And the procedure will eventually come to an end because the nonnegative integer  $\ell(T)$  decreases every time we resolve a conflict in  $T$  (by Lemma 5.9 (d)).

Let us first resolve the conflict (2,3) in  $T$ . This gives us the 12-table

$$\text{res}_2 T = \begin{array}{ccccc} & & & 1 & 2 & 1 \\ & & & 1 & 1 & 2 \\ & 2 & 1 & 1 & & \\ & 2 & 1 & 2 & & \\ & 2 & & & & \end{array} .$$

(In fact, we have seen this in Example 5.6 already, but we denoted the 12-table by  $P$  there.) Next, resolving the conflict (4,5) in  $\text{res}_2 T$ , we obtain the 12-table

$$\text{res}_4(\text{res}_2 T) = \begin{array}{ccccc} & & & 1 & 1 & 2 \\ & & & 1 & 1 & 1 \\ & 2 & 1 & 1 & & \\ & 2 & 1 & 2 & & \\ & 2 & & & & \end{array} .$$

We go on by resolving the conflict (1,2) in  $\text{res}_4(\text{res}_2 T)$ , and thus obtain

$$\text{res}_1(\text{res}_4(\text{res}_2 T)) = \begin{array}{ccccc} & & & 1 & 1 & 2 \\ & & & 2 & 1 & 1 \\ & 1 & 2 & 1 & & \\ & 1 & 2 & 2 & & \\ & 1 & & & & \end{array} .$$

Next, we resolve the conflict  $(2, 3)$  in  $\text{res}_1(\text{res}_4(\text{res}_2 T))$ , and obtain

$$\text{res}_2(\text{res}_1(\text{res}_4(\text{res}_2 T))) = \begin{array}{|c|c|c|} \hline & 2 & 1 & 2 \\ \hline & 1 & 2 & 1 \\ \hline 1 & 1 & 2 & \\ \hline 1 & 2 & 2 & \\ \hline 1 & & & \\ \hline \end{array}.$$

Next, we resolve the conflict  $(3, 4)$  in  $\text{res}_2(\text{res}_1(\text{res}_4(\text{res}_2 T)))$ , and this leads us to

$$\text{res}_3(\text{res}_2(\text{res}_1(\text{res}_4(\text{res}_2 T)))) = \begin{array}{|c|c|c|} \hline & 1 & 2 & 2 \\ \hline & 1 & 1 & 2 \\ \hline 1 & 1 & 1 & \\ \hline 1 & 2 & 1 & \\ \hline 1 & & & \\ \hline \end{array}.$$

Finally, we resolve the conflict  $(2, 3)$  in  $\text{res}_3(\text{res}_2(\text{res}_1(\text{res}_4(\text{res}_2 T))))$ , and thus obtain

$$\text{res}_2(\text{res}_3(\text{res}_2(\text{res}_1(\text{res}_4(\text{res}_2 T)))) = \begin{array}{|c|c|c|} \hline & 1 & 2 & 2 \\ \hline & 1 & 1 & 2 \\ \hline 1 & 1 & 1 & \\ \hline 1 & 1 & 2 & \\ \hline 1 & & & \\ \hline \end{array}.$$

This 12-table  $\text{res}_2(\text{res}_3(\text{res}_2(\text{res}_1(\text{res}_4(\text{res}_2 T))))$  has no more conflicts, and thus is final. So  $\text{norm}(T) = \text{res}_2(\text{res}_3(\text{res}_2(\text{res}_1(\text{res}_4(\text{res}_2 T))))$ .

Notice that we have needed six steps to compute  $\text{norm}(T)$ , although  $T$  only had 4 conflicts. So the number of conflicts does not always decrease when we resolve a conflict. (It is easy to construct an example where it can actually increase.) This is why we could not have used a function  $\ell : \mathbf{S} \rightarrow \mathbb{N}$  that counts the number of conflicts to satisfy the length-decrease condition.

## 5.9. Definition of $\mathbf{B}$

We can now finally prove Lemma 3.5.

**Definition 5.15.** Let us define a map  $\mathbf{B} : \mathbf{R} \rightarrow \mathbf{R}$  as follows:

Let  $T \in \mathbf{R}$ . Then,  $T \in \mathbf{R} \subseteq \mathbf{S}$ . Hence,  $\text{flip}(T) \in \mathbf{S}$  is well-defined, and thus  $\text{norm}(\text{flip}(T)) \in \mathbf{R}$  is well-defined. We define  $\mathbf{B}(T)$  to be  $\text{norm}(\text{flip}(T))$ .

Thus, the map  $\mathbf{B}$  is defined. In order to complete the proof of Lemma 3.5, we

need to show that this map  $\mathbf{B}$  is an involution and that, for every  $S \in \mathbf{R}$ , the equalities (7) and (8) hold. At this point, all of this is easy:

*Proof that  $\mathbf{B}$  is an involution:* Let  $T \in \mathbf{R}$ . The definition of  $\mathbf{B}$  yields  $\mathbf{B}(T) = \text{norm}(\text{flip}(T))$ . From (32) (applied to  $\text{flip}(T)$  instead of  $T$ ), we have  $\text{flip}(T) \stackrel{*}{\Rightarrow} \text{norm}(\text{flip}(T))$ . This rewrites as  $\text{flip}(T) \stackrel{*}{\Rightarrow} \mathbf{B}(T)$  (since  $\mathbf{B}(T) = \text{norm}(\text{flip}(T))$ ). Lemma 5.10 (c) (applied to  $P = \text{flip}(T)$  and  $Q = \mathbf{B}(T)$ ) thus yields  $\text{flip}(\mathbf{B}(T)) \stackrel{*}{\Rightarrow} \text{flip}(\text{flip}(T))$ . Since  $\text{flip}(\text{flip}(T)) = \underbrace{(\text{flip} \circ \text{flip})}_{=\text{id}}(T) = \text{id}(T) = T$ , this (by Proposition 5.4 (a))

rewrites as  $\text{flip}(\mathbf{B}(T)) \stackrel{*}{\Rightarrow} T$ .

But  $T \in \mathbf{R}$ . In other words,  $T$  is a 12-rpp (since  $\mathbf{R}$  is the set of all 12-rpps of shape  $Z$ ). Thus,  $T$  is final (because Proposition 5.12 (applied to  $P = T$ ) yields that  $T$  is final if and only if  $T$  is a 12-rpp).

Now, recall that  $\text{norm}(T)$  is the unique final element  $b \in \mathbf{S}$  such that  $T \stackrel{*}{\Rightarrow} b$  (by the definition of  $\text{norm}(T)$ ). Applying this to  $\text{flip}(\mathbf{B}(T))$  instead of  $T$ , we see that  $\text{norm}(\text{flip}(\mathbf{B}(T)))$  is the unique final element  $b \in \mathbf{S}$  such that  $\text{flip}(\mathbf{B}(T)) \stackrel{*}{\Rightarrow} b$ . Hence, every final element  $b \in \mathbf{S}$  such that  $\text{flip}(\mathbf{B}(T)) \stackrel{*}{\Rightarrow} b$  must satisfy  $b = \text{norm}(\text{flip}(\mathbf{B}(T)))$ . Applying this to  $b = T$ , we obtain  $T = \text{norm}(\text{flip}(\mathbf{B}(T)))$  (since  $T$  is a final element of  $\mathbf{S}$  satisfying  $\text{flip}(\mathbf{B}(T)) \stackrel{*}{\Rightarrow} T$ ).

But  $(\mathbf{B} \circ \mathbf{B})(T) = \mathbf{B}(\mathbf{B}(T)) = \text{norm}(\text{flip}(\mathbf{B}(T)))$  (by the definition of  $\mathbf{B}(\mathbf{B}(T))$ ). Comparing this with  $T = \text{norm}(\text{flip}(\mathbf{B}(T)))$ , we obtain  $(\mathbf{B} \circ \mathbf{B})(T) = T$ .

Let us now forget that we fixed  $T$ . We thus have shown that  $(\mathbf{B} \circ \mathbf{B})(T) = T$  for every  $T \in \mathbf{R}$ . In other words,  $\mathbf{B} \circ \mathbf{B} = \text{id}$ . In other words,  $\mathbf{B}$  is an involution.

*Proof of the equality (7) for every  $S \in \mathbf{R}$ :* Let  $S \in \mathbf{R}$ . The definition of  $\mathbf{B}$  yields  $\mathbf{B}(S) = \text{norm}(\text{flip}(S))$ . But (32) (applied to  $T = \text{flip}(S)$ ) yields  $\text{flip}(S) \stackrel{*}{\Rightarrow} \text{norm}(\text{flip}(S))$ . This rewrites as  $\text{flip}(S) \stackrel{*}{\Rightarrow} \mathbf{B}(S)$  (since  $\mathbf{B}(S) = \text{norm}(\text{flip}(S))$ ). Lemma 5.10 (a) (applied to  $P = \text{flip}(S)$  and  $Q = \mathbf{B}(S)$ ) thus yields

$$\text{ceq}(\mathbf{B}(S)) = \text{ceq}(\text{flip}(S)) = \text{ceq}(S)$$

(by (17), applied to  $T = S$ ). This proves (7).

*Proof of the equality (8) for every  $S \in \mathbf{R}$ :* Let  $S \in \mathbf{R}$ . The definition of  $\mathbf{B}$  yields  $\mathbf{B}(S) = \text{norm}(\text{flip}(S))$ . But (32) (applied to  $T = \text{flip}(S)$ ) yields  $\text{flip}(S) \stackrel{*}{\Rightarrow} \text{norm}(\text{flip}(S))$ . This rewrites as  $\text{flip}(S) \stackrel{*}{\Rightarrow} \mathbf{B}(S)$  (since  $\mathbf{B}(S) = \text{norm}(\text{flip}(S))$ ). Lemma 5.10 (b) (applied to  $P = \text{flip}(S)$  and  $Q = \mathbf{B}(S)$ ) thus yields

$$\text{ircont}(\mathbf{B}(S)) = \text{ircont}(\text{flip}(S)) = s_1 \cdot \text{ircont}(S)$$

(by (18), applied to  $T = S$ ). This proves (8).

We have thus shown that  $\mathbf{B}$  is an involution, and that, for every  $S \in \mathbf{R}$ , the equalities (7) and (8) hold. This completes the proof of Lemma 3.5. Thus, Lemma

3.6 is proven (since we have proven it using Lemma 3.5), and consequently Theorem 3.4 is proven (since we have derived it from Lemma 3.6). This, in turn, finishes the proof of Theorem 3.3 (since we have proven Theorem 3.3 using Theorem 3.4).

## 6. The classical Bender-Knuth involutions

### 6.1. Recalling the definition of $\mathbf{B}_i$

We fix a skew partition  $\lambda/\mu$  and a positive integer  $i$  for the whole Section 6.

Theorem 3.4 merely claims the existence of an involution  $\mathbf{B}_i : \text{RPP}(\lambda/\mu) \rightarrow \text{RPP}(\lambda/\mu)$  satisfying certain properties. Such an involution, per se, need not be unique. However, if we trace back the proof of Theorem 3.4 (and the proofs of the lemmas that were used in this proof), we notice that this proof constructs a specific involution  $\mathbf{B}_i$ . This construction is spread across various proofs; we can summarize it as follows:

- The main step of the construction was the construction of the involution  $\mathbf{B} : \mathbf{R} \rightarrow \mathbf{R}$  in the proof of Lemma 3.5 (for a given finite convex subset  $Z$  of  $\mathbb{N}_+^2$ ). This is an involution which sends 12-rpps of shape  $Z$  to 12-rpps of the same shape  $Z$ , and it was constructed as follows: Given a 12-rpp  $T$  of shape  $Z$ , we set  $\mathbf{B}(T) = \text{norm}(\text{flip}(T))$ . (Recall that  $\text{flip}(T)$  fills all the 1-pure columns of  $T$  with 2's while simultaneously filling all the 2-pure columns of  $T$  with 1's. Recall furthermore that  $\text{norm}(\text{flip}(T))$  is obtained from  $\text{flip}(T)$  by repeatedly resolving conflicts until no conflicts remain.)
- Having constructed this map  $\mathbf{B} : \mathbf{R} \rightarrow \mathbf{R}$ , we can construct the involution  $\mathbf{B}_Z : \mathbf{R}_Z \rightarrow \mathbf{R}_Z$  in Lemma 3.6 (for a given finite convex subset  $Z$  of  $\mathbb{N}_+^2$ ) as follows: Given an rpp  $S$  of shape  $Z$  whose entries are  $i$ 's and  $(i+1)$ 's, we first replace these entries by 1's and 2's (respectively), so that we obtain a 12-rpp; then, we apply the involution  $\mathbf{B} : \mathbf{R} \rightarrow \mathbf{R}$  to this 12-rpp; and then, in the resulting 12-rpp, we change the 1's and 2's back into  $i$ 's and  $(i+1)$ 's. The resulting rpp is  $\mathbf{B}_Z(S)$ .
- Finally, we can construct the involution  $\mathbf{B}_i : \text{RPP}(\lambda/\mu) \rightarrow \text{RPP}(\lambda/\mu)$ . To wit, if we are given an rpp  $S \in \text{RPP}(\lambda/\mu)$ , then we can restrict our attention to the cells of  $S$  which contain the entries  $i$  and  $i+1$ . These cells form an rpp of some shape  $Z$ . We then apply the involution  $\mathbf{B}_Z$  to this new rpp, while leaving all the remaining entries of  $S$  unchanged. The result is an rpp of shape  $Y(\lambda/\mu)$  again; this rpp is  $\mathbf{B}_i(S)$ .

In the following, whenever we will be talking about the involution  $\mathbf{B}_i$ , we will always mean this particular involution  $\mathbf{B}_i$ , rather than an arbitrary involution  $\mathbf{B}_i$  that satisfies the claims of Theorem 3.4.

## 6.2. The Bender-Knuth involutions

We claimed that our involution  $\mathbf{B}_i : \text{RPP}(\lambda/\mu) \rightarrow \text{RPP}(\lambda/\mu)$  is a generalization of the  $i$ -th Bender-Knuth involution defined for semistandard tableaux. Let us now elaborate on this claim. First, we shall define the  $i$ -th Bender-Knuth involution (following [GriRei15, proof of Proposition 2.11] and [Stan99, proof of Theorem 7.10.2]).

Let  $\text{SST}(\lambda/\mu)$  denote the set of all semistandard tableaux of shape  $Y(\lambda/\mu)$ . We define a map  $B_i : \text{SST}(\lambda/\mu) \rightarrow \text{SST}(\lambda/\mu)$  as follows:<sup>41</sup>

Let  $T \in \text{SST}(\lambda/\mu)$ . Then,  $T$  is a semistandard tableau, so that every column of  $T$  contains at most one  $i$  and at most one  $i+1$ . We shall ignore all columns of  $T$  which contain both an  $i$  and an  $i+1$ ; that is, we mark all the entries of all such columns as “ignored”. Now, let  $k \in \mathbb{N}_+$ . The  $k$ -th row of  $T$  is a weakly increasing sequence of positive integers; thus, it contains a (possibly empty) string of  $i$ ’s followed by a (possibly empty) string of  $(i+1)$ ’s. These two strings together form a substring of the  $k$ -th row which looks as follows:

$$(i, i, \dots, i, i+1, i+1, \dots, i+1)$$

<sup>42</sup>. Some of the entries of this substring are “ignored”; it is easy to see that the “ignored”  $i$ ’s are gathered at the left end of the substring whereas the “ignored”  $(i+1)$ ’s are gathered at the right end of the substring. So the substring looks as follows:

$$\left( \underbrace{i, i, \dots, i}_{\substack{a \text{ many } i\text{'s which} \\ \text{are "ignored"}}} , \underbrace{i, i, \dots, i}_{\substack{r \text{ many } i\text{'s which} \\ \text{are not "ignored"}}} , \underbrace{i+1, i+1, \dots, i+1}_{\substack{s \text{ many } (i+1)\text{'s which} \\ \text{are not "ignored"}}} , \underbrace{i+1, i+1, \dots, i+1}_{\substack{b \text{ many } (i+1)\text{'s which} \\ \text{are "ignored"}}} \right)$$

for some  $a, r, s, b \in \mathbb{N}$ . Now, we change this substring into

$$\left( \underbrace{i, i, \dots, i}_{\substack{a \text{ many } i\text{'s which} \\ \text{are "ignored"}}} , \underbrace{i, i, \dots, i}_{\substack{s \text{ many } i\text{'s which} \\ \text{are not "ignored"}}} , \underbrace{i+1, i+1, \dots, i+1}_{\substack{r \text{ many } (i+1)\text{'s which} \\ \text{are not "ignored"}}} , \underbrace{i+1, i+1, \dots, i+1}_{\substack{b \text{ many } (i+1)\text{'s which} \\ \text{are "ignored"}}} \right).$$

And we do this for every  $k \in \mathbb{N}_+$  (simultaneously or consecutively – it does not matter). At the end, we have obtained a new semistandard tableau of shape  $Y(\lambda/\mu)$ . We define  $B_i(T)$  to be this new tableau.

<sup>41</sup>We refer to Example 6.1 below for illustration.

<sup>42</sup>Of course, this substring might contain no  $i$ ’s or no  $(i+1)$ ’s.

**Example 6.1.** Let us give an example of this construction of  $B_i$ . Namely, let  $i = 2$ , let  $\lambda = (7, 6, 4, 1)$ , and let  $\mu = (3)$ . Let  $T$  be the semistandard tableau

|   |   |   |   |   |   |   |   |
|---|---|---|---|---|---|---|---|
|   |   |   |   | 1 | 1 | 2 | 2 |
| 1 | 2 | 2 | 2 | 3 | 3 |   |   |
| 3 | 3 | 5 | 6 |   |   |   |   |
| 4 |   |   |   |   |   |   |   |

of shape  $Y(\lambda/\mu)$ . We want to find  $B_i(T)$ .

The columns that contain both an  $i$  and an  $i + 1$  (that is, both a 2 and a 3) are the second and the sixth columns. So we mark all entries of these two columns as “ignored”. Now, the substring of the 2-nd row of  $T$  formed by the  $i$ ’s and the  $(i + 1)$ ’s looks as follows:

$$\left( \underbrace{2}_{\substack{1 \text{ many } 2\text{'s which} \\ \text{are "ignored"}}}, \underbrace{2, 2}_{\substack{2 \text{ many } 2\text{'s which} \\ \text{are not "ignored"}}}, \underbrace{3}_{\substack{1 \text{ many } 3\text{'s which} \\ \text{are not "ignored"}}}, \underbrace{3}_{\substack{2 \text{ many } 3\text{'s which} \\ \text{are "ignored"}}} \right).$$

So we change it into

$$\left( \underbrace{2}_{\substack{1 \text{ many } 2\text{'s which} \\ \text{are "ignored"}}}, \underbrace{2}_{\substack{1 \text{ many } 2\text{'s which} \\ \text{are not "ignored"}}}, \underbrace{3, 3}_{\substack{2 \text{ many } 3\text{'s which} \\ \text{are not "ignored"}}}, \underbrace{3}_{\substack{2 \text{ many } 3\text{'s which} \\ \text{are "ignored"}}} \right).$$

Similarly, we change the substring  $(2, 2)$  of the 1-st row of  $T$  into  $(2, 3)$  (because its first 2 is “ignored” but its second 2 is not), and we change the substring  $(3, 3)$  of the 3-rd row of  $T$  into  $(2, 3)$  (because its first 3 is not “ignored” but its second 3 is). The substring of the 4-th row, of the 5-th row, of the 6-th row, etc., formed by the  $i$ ’s and  $(i + 1)$ ’s are empty (because these rows contain neither  $i$ ’s nor  $(i + 1)$ ’s), and thus we do not make any changes on them. Now,  $B_i(T)$  is defined to be the tableau that results from all of these changes; thus,

$$B_i(T) = \begin{array}{cccccc} & & & & 1 & 1 & 2 & 3 \\ 1 & 2 & 2 & 3 & 3 & 3 & & \\ 2 & 3 & 5 & 6 & & & & \\ 4 & & & & & & & \end{array}.$$

**Proposition 6.2.** The map  $B_i : \text{SST}(\lambda/\mu) \rightarrow \text{SST}(\lambda/\mu)$  thus defined is an involution. It is known as the  $i$ -th Bender-Knuth involution.

Proposition 6.2 is easy to prove (and is usually proven in less or more detail everywhere the map  $B_i$  is defined).

Now, every semistandard tableau of shape  $Y(\lambda/\mu)$  is also an rpp of shape  $Y(\lambda/\mu)$ . In other words,  $\text{SST}(\lambda/\mu) \subseteq \text{RPP}(\lambda/\mu)$ . Hence,  $\mathbf{B}_i(T)$  is defined for every  $T \in \text{SST}(\lambda/\mu)$ . Now, the claim that we want to make (that our involution  $\mathbf{B}_i$  is a generalization of the  $i$ -th Bender-Knuth involution  $B_i$ ) can be stated as follows:

**Proposition 6.3.** For every  $T \in \text{SST}(\lambda/\mu)$ , we have  $B_i(T) = \mathbf{B}_i(T)$ .

*Proof of Proposition 6.3 (sketched).* We shall abbreviate “semistandard tableau” as “sst”. We define a 12-sst to be an sst whose entries all belong to the set  $\{1, 2\}$ .

Let  $Z$  be a finite convex subset of  $\mathbb{N}_+^2$ . Let  $R$  denote the set of all 12-ssts of shape  $Z$ . We define a map  $B : R \rightarrow R$  in the same way as we defined the map  $B_i : \text{SST}(\lambda/\mu) \rightarrow \text{SST}(\lambda/\mu)$ , with the only differences that we replace every appearance of “SST( $\lambda/\mu$ )”, of “ $i$ ” and of “ $i + 1$ ” by “ $R$ ”, “1” and “2”, respectively. Then, this map  $B : R \rightarrow R$  is an involution.

Now let us forget that we fixed  $Z$ . We thus have constructed a map  $B : R \rightarrow R$  for every finite convex subset  $Z$  of  $\mathbb{N}_+^2$ . Now, recall how the map  $\mathbf{B}_i : \text{RPP}(\lambda/\mu) \rightarrow \text{RPP}(\lambda/\mu)$  was constructed from the maps  $\mathbf{B} : \mathbf{R} \rightarrow \mathbf{R}$  for every finite convex subset  $Z$  of  $\mathbb{N}_+^2$  (essentially by forgetting all entries of an rpp except for the entries  $i$  and  $i + 1$  and relabelling these entries  $i$  and  $i + 1$  as 1 and 2). Similarly, the map  $B_i : \text{SST}(\lambda/\mu) \rightarrow \text{SST}(\lambda/\mu)$  can be constructed from the maps  $B : R \rightarrow R$  for every finite convex subset  $Z$  of  $\mathbb{N}_+^2$  (essentially by forgetting all entries of an sst except for the entries  $i$  and  $i + 1$  and relabelling these entries  $i$  and  $i + 1$  as 1 and 2). Thus, in order to prove that  $B_i(T) = \mathbf{B}_i(T)$  for every  $T \in \text{SST}(\lambda/\mu)$ , it suffices to show that  $B(T) = \mathbf{B}(T)$  for every finite convex subset  $Z$  of  $\mathbb{N}_+^2$  and any 12-sst  $T$  of shape  $Z$ .

So let  $Z$  be any finite convex subset of  $\mathbb{N}_+^2$ , and let  $T$  be a 12-sst of shape  $Z$ . We need to prove that  $B(T) = \mathbf{B}(T)$ .

**Example 6.4.** Here is an example of a 12-sst:

$$T = \begin{array}{c} \begin{array}{|c|c|} \hline 1 & 2 \\ \hline 2 & \\ \hline \end{array} \quad \begin{array}{|c|c|c|c|} \hline 1 & 2 & 2 & 2 \\ \hline & 1 & 1 & 2 \\ \hline & & & 1 \\ \hline \end{array} \end{array} . \quad (33)$$

It satisfies

$$B(T) = \begin{array}{cccc} & & & 2 \\ & & 1 & 1 & 1 \\ & 1 & 2 & 2 & 2 \\ 1 & 1 & & & \\ 2 & & & & \end{array} \quad (34)$$

and

$$\text{flip}(T) = \begin{array}{cccc} & & & 2 \\ & & 1 & 1 & 1 \\ 2 & 1 & 2 & 2 & \\ 1 & 1 & & & \\ 2 & & & & \end{array} \quad (35)$$

(where  $\text{flip}(T)$  is defined as in the construction of  $\mathbf{B}(T)$ ).

We make a few basic observations: The columns which are ignored in the construction of  $B(T)$  are the columns which contain both a 1 and a 2.<sup>43</sup> These columns contain exactly two entries each (because a column of a 12-sst can only contain at most one 1, at most one 2 and no other entries), while every other column is either empty or contains only one entry. As a consequence, every entry of  $T$  which is not “ignored” in the construction of  $B(T)$  is alone in its column.

Let us compare the basic ideas of the constructions of  $B(T)$  and  $\mathbf{B}(T)$ :

- To construct  $B(T)$ , we ignore all columns of  $T$  which contain both a 1 and a 2; that is, we mark all entries in these columns as “ignored”. Then, in every row, we let  $r$  be the number of 1’s which are not “ignored”, and let  $s$  be the number of 2’s which are not “ignored”. We replace these  $r$  many 1’s and  $s$  many 2’s by  $s$  many 1’s and  $r$  many 2’s. This we do for every row; the resulting 12-sst is  $B(T)$ .
- To construct  $\mathbf{B}(T)$ , we consider  $T$  as a 12-rpp, and we identify which of its columns are 1-pure, which are 2-pure and which are mixed. Then, we replace all entries of all 1-pure columns by 2’s, while simultaneously replacing all entries of all 2-pure columns by 1’s. The resulting 12-table is denoted  $\text{flip}(T)$ . Then, we repeatedly resolve conflicts in  $\text{flip}(T)$  until no more conflicts remain. The resulting 12-table  $\text{norm}(\text{flip}(T))$  is a 12-rpp, and is denoted  $\mathbf{B}(T)$ .

If we compare the two constructions just described, we first notice that the columns ignored in the construction of  $B(T)$  are precisely the mixed columns of

<sup>43</sup>For instance, in the 12-sst (33), the ignored columns are the 1-st, the 6-th and the 7-th columns.



$T$ . Thus, the 12-table flip ( $T$ ) can be obtained from  $T$  by replacing all 1's which are not "ignored" by 2's while simultaneously replacing all 2's which are not "ignored" by 1's. Thus, for any given  $k \in \mathbb{N}_+$ , if the  $k$ -th row of  $T$  contains  $r$  many 1's which are not "ignored" and  $s$  many 2's which are not "ignored", then the  $k$ -th row of flip ( $T$ ) contains  $r$  many 2's which are not "ignored" and  $s$  many 1's which are not "ignored" (while the "ignored" entries in  $T$  appear in flip ( $T$ ) unchanged). So we can restate the construction of flip ( $T$ ) as follows:

- To construct flip ( $T$ ) from  $T$ , do the following: In every row of  $T$ , let  $r$  be the number of 1's which are not "ignored", and let  $s$  be the number of 2's which are not "ignored". We replace these  $r$  many 1's and  $s$  many 2's by  $r$  many 2's and  $s$  many 1's (in this order). This we do for every row; the resulting 12-table is flip ( $T$ ).

Compare this to our construction of  $B(T)$ :

- To construct  $B(T)$  from  $T$ , do the following: In every row of  $T$ , let  $r$  be the number of 1's which are not "ignored", and let  $s$  be the number of 2's which are not "ignored". We replace these  $r$  many 1's and  $s$  many 2's by  $s$  many 1's and  $r$  many 2's (in this order). This we do for every row; the resulting 12-sst is  $B(T)$ .

Comparing these two constructions makes it clear that each row of  $B(T)$  differs from the corresponding row of flip ( $T$ ) merely in the order in which the non-"ignored" entries appear: In  $B(T)$ , the non-"ignored" 1's appear before the non-"ignored" 2's (as they must,  $B(T)$  being an sst), whereas in flip ( $T$ ) they appear in the opposite order. Hence,  $B(T)$  can be obtained from flip ( $T$ ) by sorting all non-"ignored" entries into increasing order in each row.

Now, let us notice that every pair of a non-"ignored" 2 and a non-"ignored" 1 lying in the same row of flip ( $T$ ) cause a conflict<sup>44</sup>. Conversely, all conflicts of flip ( $T$ ) are caused by a non-"ignored" 2 and a non-"ignored" 1 lying in the same row (because all "ignored" entries are carried over from  $T$  without change and thus cannot take part in conflicts). We can resolve these conflicts one after the other (starting with the 2 and the 1 that are adjacent to each other), until none are left. The result is a 12-rpp. What is this 12-rpp?

- On the one hand, this 12-rpp is norm (flip ( $T$ )), because norm (flip ( $T$ )) is defined as what results when all conflicts of flip ( $T$ ) are resolved.
- On the other hand, this 12-rpp is  $B(T)$ . In fact, resolving a conflict caused by a non-"ignored" 2 and a non-"ignored" 1 lying in the same row results in this 2 getting switched with the 1 (while no other entries get moved<sup>45</sup>).

<sup>44</sup>More precisely: If  $r \in \mathbb{N}_+$ ,  $i \in \mathbb{N}_+$  and  $j \in \mathbb{N}_+$  are such that (flip  $T$ ) ( $r, i$ ) is a non-"ignored" 2 and that (flip  $T$ ) ( $r, j$ ) is a non-"ignored" 1, then  $(i, j)$  is a conflict of flip  $T$ .

<sup>45</sup>This is because every non-"ignored" entry is alone in its column.

Hence, when we resolve the conflicts, we just sort all non-“ignored” entries into increasing order in each row. But as we know, the 12-table obtained from  $\text{flip}(T)$  by sorting all non-“ignored” entries into increasing order in each row is  $B(T)$ .

So we have found a 12-rpp which equals both  $\text{norm}(\text{flip}(T))$  and  $B(T)$ . Thus,  $B(T) = \text{norm}(\text{flip}(T)) = \mathbf{B}(T)$ . This completes our proof of Proposition 6.3.  $\square$

## 7. The structure of 12-rpps

In this section, we let  $\mathbf{k}$  be the polynomial ring  $\mathbb{Z}[t_1, t_2, t_3, \dots]$  in countably many indeterminates, and we let  $t_1, t_2, t_3, \dots$  be these indeterminates. Furthermore, we restrict ourselves to the two-variable dual stable Grothendieck polynomial  $\tilde{g}_{\lambda/\mu}(x_1, x_2, 0, 0, \dots; \mathbf{t})$  defined as the result of substituting  $0, 0, 0, \dots$  for  $x_3, x_4, x_5, \dots$  in  $\tilde{g}_{\lambda/\mu}$ . We can represent it as a polynomial in  $\mathbf{t}$  with coefficients in  $\mathbb{Z}[x_1, x_2]$ :

$$\tilde{g}_{\lambda/\mu}(x_1, x_2, 0, 0, \dots; \mathbf{t}) = \sum_{\alpha \in \mathbb{N}^{\mathbb{N}_+}} \mathbf{t}^\alpha Q_\alpha(x_1, x_2),$$

where the sum ranges over all weak compositions  $\alpha$ , and all but finitely many  $Q_\alpha(x_1, x_2)$  are 0. (The  $Q_\alpha(x_1, x_2)$  here belong to  $\mathbb{Z}[x_1, x_2]$ .)

We shall show that each  $Q_\alpha(x_1, x_2)$  is either zero or has the form

$$Q_\alpha(x_1, x_2) = (x_1 x_2)^M P_{n_0}(x_1, x_2) P_{n_1}(x_1, x_2) \cdots P_{n_r}(x_1, x_2), \quad (36)$$

where  $M, r$  and  $n_0, n_1, \dots, n_r$  are nonnegative integers naturally associated to  $\alpha$  and  $\lambda/\mu$  and where

$$P_n(x_1, x_2) = \frac{x_1^{n+1} - x_2^{n+1}}{x_1 - x_2} = x_1^n + x_1^{n-1}x_2 + \cdots + x_1x_2^{n-1} + x_2^n.$$

We fix the skew partition  $\lambda/\mu$  throughout the whole section. Abusing notation, we shall abbreviate  $Y(\lambda/\mu)$  as  $\lambda/\mu$ . We will have a running example with  $\lambda = (7, 7, 7, 4, 4)$  and  $\mu = (5, 3, 2)$ .

### 7.1. Irreducible components

We recall that a 12-rpp means an rpp whose entries all belong to the set  $\{1, 2\}$ .

Given a 12-rpp  $T$ , consider the set  $\text{NR}(T)$  of all cells  $(i, j) \in \lambda/\mu$  such that  $T(i, j) = 1$  but  $(i+1, j) \in \lambda/\mu$  and  $T(i+1, j) = 2$ . (In other words,  $\text{NR}(T)$  is the set of all non-redundant cells in  $T$  which are filled with a 1 and which are not the lowest cells in their columns.) Clearly,  $\text{NR}(T)$  contains at most one cell from each column; thus, let us write  $\text{NR}(T) = \{(i_1, j_1), (i_2, j_2), \dots, (i_s, j_s)\}$  with

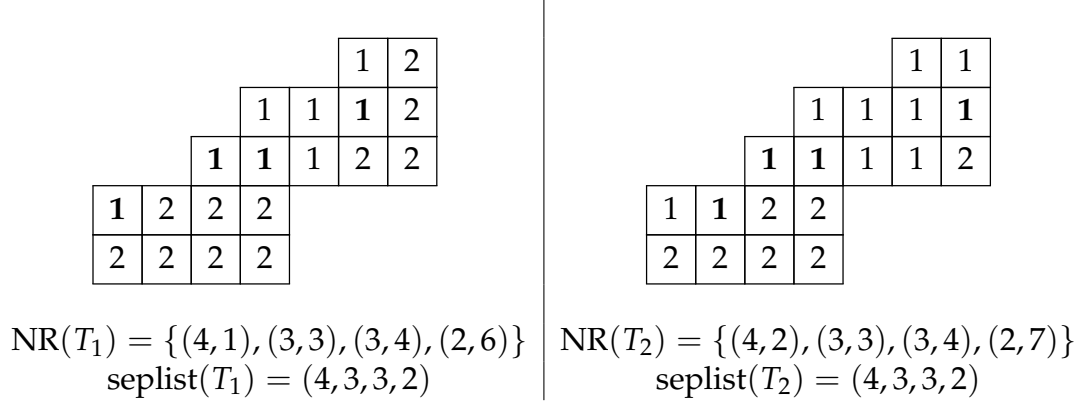

Figure 1: Two 12-rpps of the same shape and with the same seplist-partition.

$j_1 < j_2 < \dots < j_s$ . Because  $T$  is a 12-rpp, it follows that the numbers  $i_1, i_2, \dots, i_s$  decrease weakly, therefore they form a partition which we denoted

$$\text{seplist}(T) := (i_1, i_2, \dots, i_s)$$

in Section 5.3. This partition will be called the *seplist-partition* of  $T$ . An example of calculation of  $\text{seplist}(T)$  and  $\text{NR}(T)$  is illustrated on Figure 1.

We would like to answer the following question: for which partitions  $\nu = (i_1 \geq \dots \geq i_s > 0)$  does there exist a 12-rpp  $T$  of shape  $\lambda/\mu$  such that  $\text{seplist}(T) = \nu$ ?

A trivial necessary condition for this to happen is that there should exist some numbers  $j_1 < j_2 < \dots < j_s$  such that

$$(i_1, j_1), (i_1 + 1, j_1), (i_2, j_2), (i_2 + 1, j_2), \dots, (i_s, j_s), (i_s + 1, j_s) \in \lambda/\mu. \quad (37)$$

Until the end of Section 7, we make an assumption: namely, that the skew partition  $\lambda/\mu$  is connected as a subgraph of  $\mathbb{Z}^2$  (where two nodes are connected if and only if their cells have an edge in common), and that it has no empty columns. This is a harmless assumption, since every skew partition  $\lambda/\mu$  can be written as a disjoint union of such connected skew partitions, and the corresponding seplist-partition splits into several independent parts, the polynomials  $\tilde{g}_{\lambda/\mu}$  get multiplied and the right hand side of (36) changes accordingly.

For each integer  $i$ , the set of all integers  $j$  such that  $(i, j), (i + 1, j) \in \lambda/\mu$  is just an interval  $[\mu_i + 1, \lambda_{i+1}]$ , which we call *the support of  $i$*  and denote  $\text{supp}(i) := [\mu_i + 1, \lambda_{i+1}]$ .

We say that a partition  $\nu$  is *admissible* if every  $k$  satisfies  $\text{supp}(i_k) \neq \emptyset$ . (This is clearly satisfied when there exist  $j_1 < j_2 < \dots < j_s$  satisfying (37), but also in other cases.) Assume that  $\nu = (i_1 \geq \dots \geq i_s > 0)$  is an admissible partition. For two integers  $a < b$ , we let  $\nu|_{\subseteq [a,b]}$  denote the subpartition  $(i_r, i_{r+1}, \dots, i_{r+q})$  of  $\nu$ , where  $[r, r+q]$  is the (possibly empty) set of all  $k$  for which  $\text{supp}(i_k) \subseteq [a, b]$ . In this case, we put<sup>46</sup>  $\#\nu|_{\subseteq [a,b]} := q + 1$ , which is just the number of entries in

<sup>46</sup>Here and in the following,  $\#\kappa$  denotes the length of a partition  $\kappa$ .

$\nu|_{\subseteq[a,b]}$ . Similarly, we set  $\nu|_{\cap[a,b]}$  to be the subpartition  $(i_r, i_{r+1}, \dots, i_{r+q})$  of  $\nu$ , where  $[r, r+q]$  is the set of all  $k$  for which  $\text{supp}(i_k) \cap [a, b] \neq \emptyset$ . For example, for  $\nu = (4, 3, 3, 2)$  and  $\lambda/\mu$  as on Figure 1, we have

$$\text{supp}(3) = [3, 4], \text{supp}(2) = [4, 7], \text{supp}(4) = [1, 4],$$

$$\nu|_{\subseteq[2,7]} = (3, 3), \nu|_{\subseteq[2,8]} = (3, 3, 2), \nu|_{\subseteq[4,8]} = (2), \nu|_{\cap[4,5]} = (4, 3, 3, 2), \# \nu|_{\subseteq[2,7]} = 2.$$

**Remark 7.1.** If  $\nu$  is not admissible, that is, if  $\text{supp}(i_k) = \emptyset$  for some  $k$ , then  $i_k$  belongs to  $\nu|_{\subseteq[a,b]}$  for any  $a, b$ , so  $\nu|_{\subseteq[a,b]}$  might no longer be a contiguous subpartition of  $\nu$ . On the other hand, if  $\nu$  is an admissible partition, then the partitions  $\nu|_{\subseteq[a,b]}$  and  $\nu|_{\cap[a,b]}$  are clearly admissible as well. For the rest of this section, we will only work with admissible partitions.

We introduce several definitions: An admissible partition  $\nu = (i_1 \geq \dots \geq i_s > 0)$  is called

- *non-representable* if for some  $a < b$  we have  $\# \nu|_{\subseteq[a,b]} > b - a$ ;
- *representable* if for all  $a < b$  we have  $\# \nu|_{\subseteq[a,b]} \leq b - a$ ;

a representable partition  $\nu$  is called

- *irreducible* if for all  $a < b$  we have  $\# \nu|_{\subseteq[a,b]} < b - a$ ;
- *reducible* if for some  $a < b$  we have  $\# \nu|_{\subseteq[a,b]} = b - a$ .

For example,  $\nu = (4, 3, 3, 2)$  is representable but reducible because we have  $\nu|_{\subseteq[3,5]} = (3, 3)$  so  $\# \nu|_{\subseteq[3,5]} = 2 = 5 - 3$ .

Note that these notions depend on the skew partition; thus, when we want to use a skew partition  $\widetilde{\lambda/\mu}$  rather than  $\lambda/\mu$ , we will write that  $\nu$  is non-representable/irreducible/etc. *with respect to*  $\widetilde{\lambda/\mu}$ , and we denote the corresponding partitions by  $\nu|_{\subseteq[a,b]}^{\widetilde{\lambda/\mu}}$ .

These definitions can be motivated as follows. Suppose that a partition  $\nu$  is non-representable, so there exist integers  $a < b$  such that  $\# \nu|_{\subseteq[a,b]} > b - a$ . Recall that  $\nu|_{\subseteq[a,b]} =: (i_r, i_{r+1}, \dots, i_{r+q})$  contains all entries of  $\nu$  whose support is a subset of  $[a, b]$ . Thus in order for condition (37) to be true there must exist some integers  $j_r < j_{r+1} < \dots < j_{r+q}$  such that

$$(i_r, j_r), (i_r + 1, j_r), \dots, (i_{r+q}, j_{r+q}), (i_{r+q} + 1, j_{r+q}) \in \lambda/\mu.$$

On the other hand, by the definition of the support, we must have  $j_k \in \text{supp}(i_k) \subseteq [a, b]$  for all  $r \leq k \leq r+q$ . Therefore we get  $q+1$  distinct elements of  $[a, b]$  which is impossible if  $q+1 = \# \nu|_{\subseteq[a,b]} > b - a$ . It means that a non-representable partition  $\nu$  is never a seplist-partition of a 12-rpp  $T$ .

Suppose now that a partition  $\nu$  is reducible, so for some  $a < b$  we get an equality  $\# \nu|_{\subseteq[a,b]} = b - a$ . Then these integers  $j_r < \dots < j_{r+q}$  should still all belong to  $[a, b]$  and there are exactly  $b - a$  of them, hence

$$j_r = a, j_{r+1} = a + 1, \dots, j_{r+q} = a + q = b - 1. \quad (38)$$

Because  $\text{supp}(i_r) \subseteq [a, b)$  but  $\text{supp}(i_r) \neq \emptyset$  (since  $\nu$  is admissible), we have  $(i_r, a-1) \notin \lambda/\mu$ . Thus, placing a 1 into  $(i_r, a)$  and 2's into  $(i_r+1, a), (i_r+2, a), \dots$  does not put any restrictions on entries in columns  $1, \dots, a-1$ . And the same is true for columns  $b, b+1, \dots$  when we place a 2 into  $(i_{r+q}+1, b-1)$  and 1's into all cells above. Thus, if a partition  $\nu$  is reducible, then the filling of columns  $a, a+1, \dots, b-1$  is uniquely determined (by (38)), and the filling of the rest can be arbitrary – the problem of existence of a 12-rpp  $T$  such that  $\text{seplist}(T) = \nu$  reduces to two smaller independent problems of the same kind (one for the columns  $1, 2, \dots, a-1$ , the other for the columns<sup>47</sup>  $b, b+1, \dots, \lambda_1$ ). One can continue this reduction process and end up with several independent irreducible components separated from each other by mixed columns. An illustration of this phenomenon can be seen on Figure 1: the columns 3 and 4 must be mixed for any 12-rpps  $T$  with  $\text{seplist}(T) = (4, 3, 3, 2)$ .

More explicitly, we have thus shown that every nonempty interval  $[a, b) \subseteq [1, \lambda_1 + 1)$  satisfying  $\# \nu|_{\subseteq [a, b)} = b - a$  splits our problem into two independent subproblems. But if two such intervals  $[a, b)$  and  $[c, d)$  satisfy  $a \leq c \leq b \leq d$  then their union  $[a, d)$  is another such interval<sup>48</sup>. Hence, the maximal (with respect to inclusion) among all such intervals are pairwise disjoint and separated from each other by at least a distance of 1. This yields part (a) of the following lemma:

**Lemma 7.2.** Let  $\nu$  be a representable partition.

(a) There exist unique integers  $(1 = b_0 \leq a_1 < b_1 < a_2 < b_2 < \dots < a_r < b_r \leq a_{r+1} = \lambda_1 + 1)$  satisfying the following two conditions:

1. For all  $1 \leq k \leq r$ , we have  $\# \nu|_{\subseteq [a_k, b_k)} = b_k - a_k$ .
2. The set  $\bigcup_{k=0}^r [b_k, a_{k+1})$  is minimal (with respect to inclusion) among all sequences  $(1 = b_0 \leq a_1 < b_1 < a_2 < b_2 < \dots < a_r < b_r \leq a_{r+1} = \lambda_1 + 1)$  satisfying property 1.

<sup>47</sup>Recall that a 12-rpp of shape  $\lambda/\mu$  cannot have any nonempty column beyond the  $\lambda_1$ 'th one.

<sup>48</sup>*Proof.* Assume that two intervals  $[a, b)$  and  $[c, d)$  satisfying  $\# \nu|_{\subseteq [a, b)} = b - a$  and  $\# \nu|_{\subseteq [c, d)} = d - c$  intersect. We need to show that their union is another such interval.

We WLOG assume that  $a \leq c$ . Then,  $c \leq b$  (since the intervals intersect). If  $b > d$ , then the union of the two intervals is simply  $[a, b)$ , which makes our claim obvious. Hence, we WLOG assume that  $b \leq d$ . Thus,  $a \leq c \leq b \leq d$ . The union of the two intervals is therefore  $[a, d)$ , and we must show that  $\# \nu|_{\subseteq [a, d)} = d - a$ . A set of positive integers is a subset of both  $[a, b)$  and  $[c, d)$  if and only if it is a subset of  $[c, b)$ . On the other hand, a set of positive integers that is a subset of either  $[a, b)$  or  $[c, d)$  must be a subset of  $[a, d)$  (but not conversely). Combining these two observations, we obtain  $\# \nu|_{\subseteq [a, d)} \geq \# \nu|_{\subseteq [a, b)} + \# \nu|_{\subseteq [c, d)} - \# \nu|_{\subseteq [c, b)}$ . Since  $\nu$  is representable (or, when  $b = c$ , for obvious reasons), we have  $\# \nu|_{\subseteq [c, b)} \leq b - c$ . Thus,

$$\# \nu|_{\subseteq [a, d)} \geq \underbrace{\# \nu|_{\subseteq [a, b)}}_{=b-a} + \underbrace{\# \nu|_{\subseteq [c, d)}}_{=d-c} - \underbrace{\# \nu|_{\subseteq [c, b)}}_{\leq b-c} \geq (b-a) + (d-c) - (b-c) = d-a.$$

Combined with  $\# \nu|_{\subseteq [a, d)} \leq d - a$  (since  $\nu$  is representable), this yields  $\# \nu|_{\subseteq [a, d)} = d - a$ , qed.

Furthermore, for these integers, we have:

(b) The partition  $\nu$  is the concatenation

$$\left(\nu|_{\cap[b_0, a_1)}\right) \left(\nu|_{\subseteq[a_1, b_1)}\right) \left(\nu|_{\cap[b_1, a_2)}\right) \left(\nu|_{\subseteq[a_2, b_2)}\right) \cdots \left(\nu|_{\cap[b_r, a_{r+1})}\right)$$

(where we regard a partition as a sequence of positive integers, with no trailing zeroes).

(c) The partitions  $\nu|_{\cap[b_k, a_{k+1})}$  are irreducible with respect to  $\lambda/\mu|_{[b_k, a_{k+1})}$ , which is the skew partition  $\lambda/\mu$  with columns  $1, 2, \dots, b_k - 1, a_{k+1}, a_{k+1} + 1, \dots$  removed.

*Proof.* Part (a) has already been proven.

(b) Let  $\nu = (i_1 \geq \dots \geq i_s > 0)$ . If  $\text{supp}(i_r) \subseteq [a_k, b_k)$  for some  $k$ , then  $i_r$  appears in exactly one of the concatenated partitions, namely,  $\nu|_{\subseteq[a_k, b_k)}$ . Otherwise there is an integer  $k$  such that  $\text{supp}(i_r) \cap [b_k, a_{k+1}) \neq \emptyset$ . It remains to show that such  $k$  is unique, that is, that  $\text{supp}(i_r) \cap [b_{k+1}, a_{k+2}) = \emptyset$ . Assume the contrary. The interval  $[a_{k+1}, b_{k+1})$  is nonempty, therefore there is an entry  $i$  of  $\nu$  with  $\text{supp}(i) \subseteq [a_{k+1}, b_{k+1})$ . It remains to note that we get a contradiction: we get two numbers  $i, i_r$  with  $\text{supp}(i_r)$  being both to the left and to the right of  $\text{supp}(i)$ .

(c) Fix  $k$ . Let  $J$  denote the restricted skew partition  $\lambda/\mu|_{[b_k, a_{k+1})}$ , and let  $\nu' = \nu|_{\cap[b_k, a_{k+1})}$ . We need to show that if  $[c, d)$  is a nonempty interval contained in  $[b_k, a_{k+1})$ , then  $\#\nu'|_{\subseteq[c, d)}^J < d - c$ . We are in one of the following four cases:

- *Case 1:* We have  $c > b_k$  (or  $k = 0$ ) and  $d < a_{k+1}$  (or  $k = r$ ). In this case, every  $i_p$  with  $\text{supp}^J(i_p) \subseteq [c, d)$  must satisfy  $\text{supp}(i_p) \subseteq [c, d)$ . Hence,  $\nu'|_{\subseteq[c, d)}^J = \nu|_{\subseteq[c, d)}$ , so that  $\#\nu'|_{\subseteq[c, d)}^J = \#\nu|_{\subseteq[c, d)} < d - c$ , and we are done.
- *Case 2:* We have  $c = b_k$  and  $k > 0$  (but not  $d = a_{k+1}$  and  $k < r$ ). Assume (for the sake of contradiction) that  $\#\nu'|_{\subseteq[c, d)}^J \geq d - c$ . Then, the  $i_p$  satisfying  $\text{supp}^J(i_p) \subseteq [c, d)$  must satisfy  $\text{supp}(i_p) \subseteq [a_k, d)$  (since otherwise,  $\text{supp}(i_p)$  would intersect both  $[b_{k-1}, a_k)$  and  $[b_k, a_{k+1})$ , something we have ruled out in the proof of (b)). Thus,  $\#\nu|_{\subseteq[a_k, d)} \geq (d - c) + (b_k - a_k) = d - a_k$ , which contradicts the minimality of  $\bigcup_{k=0}^r [b_k, a_{k+1})$  (we could increase  $b_k$  to  $d$ ).
- *Case 3:* We have  $d = a_{k+1}$  and  $k < r$  (but not  $c = b_k$  and  $k > 0$ ). The argument here is analogous to Case 2.
- *Case 4:* Neither of the above. Exercise.

□

**Definition 7.3.** In the context of Lemma 7.2, for  $0 \leq k \leq r$  the subpartitions  $\nu|_{\cap[b_k, a_{k+1})}$  are called *the irreducible components of  $\nu$*  and the nonnegative integers  $n_k := a_{k+1} - b_k - \#\nu|_{\cap[b_k, a_{k+1})}$  are called their *degrees*. (For  $T$  with  $\text{seplist}(T) = \nu$ , the  $k$ -th degree  $n_k$  is equal to the number of pure columns of  $T$  inside the corresponding  $k$ -th irreducible component. All  $n_k$  are positive, except for  $n_0$  if  $a_1 = 1$  and  $n_r$  if  $b_r = \lambda_1 + 1$ .)

**Example 7.4.** For  $\nu = (4, 3, 3, 2)$  we have  $r = 1, b_0 = 1, a_1 = 3, b_1 = 5, a_2 = 8$ . The irreducible components of  $\nu$  are  $(4)$  and  $(2)$  and their degrees are  $3 - 1 - 1 = 1$  and  $8 - 5 - 1 = 2$  respectively. We have  $\nu|_{\cap[1,3)} = (4), \nu|_{\subseteq[3,5)} = (3, 3), \nu|_{\cap[5,8)} = (2)$ .

## 7.2. The structural theorem and its applications

It is easy to see that for a 12-rpp  $T$ , the number  $\#\text{seplist}(T)$  is equal to the number of mixed columns in  $T$ .

Let  $\text{RPP}^{12}(\lambda/\mu)$  denote the set of all 12-rpps  $T$  of shape  $\lambda/\mu$ , and let  $\text{RPP}^{12}(\lambda/\mu; \nu)$  denote its subset consisting of all 12-rpps  $T$  with  $\text{seplist}(T) = \nu$ . (Notice that  $\text{RPP}^{12}(\lambda/\mu)$  was formerly called  $\mathbf{R}$  in Lemma 3.5, if  $Z = Y(\lambda/\mu)$ .) Now we are ready to state a theorem that completely describes the structure of irreducible components (which will be proven later):

**Theorem 7.5.** Let  $\nu$  be an irreducible partition. Then for all  $0 \leq m \leq \lambda_1 - \#\nu$  there is exactly one 12-rpp  $T \in \text{RPP}^{12}(\lambda/\mu; \nu)$  with  $\#\nu$  mixed columns,  $m$  1-pure columns and  $(\lambda_1 - \#\nu - m)$  2-pure columns. Moreover, these are the only elements of  $\text{RPP}^{12}(\lambda/\mu; \nu)$ . In other words, for an irreducible partition  $\nu$  we have

$$\sum_{T \in \text{RPP}^{12}(\lambda/\mu; \nu)} \mathbf{x}^{\text{ircont}(T)} = (x_1 x_2)^{\#\nu} P_{\lambda_1 - \#\nu}(x_1, x_2). \quad (39)$$

**Example 7.6.** Each of the two 12-rpps on Figure 1 has two irreducible components. One of them is supported on the first two columns and the other one is supported on the last three columns. Here are all possible 12-rpps for each component:

$$\begin{array}{cc|ccc} \begin{array}{|c|c|} \hline 1 & 1 \\ \hline 1 & 2 \\ \hline \end{array} & \begin{array}{|c|c|} \hline 1 & 2 \\ \hline 2 & 2 \\ \hline \end{array} & \left| & \begin{array}{|c|c|c|} \hline & 1 & 1 \\ \hline 1 & 1 & 1 \\ \hline 1 & 1 & 2 \\ \hline \end{array} & \begin{array}{|c|c|c|} \hline & 1 & 2 \\ \hline 1 & 1 & 2 \\ \hline 1 & 2 & 2 \\ \hline \end{array} & \begin{array}{|c|c|c|} \hline & 2 & 2 \\ \hline 1 & 2 & 2 \\ \hline 2 & 2 & 2 \\ \hline \end{array} \\ \lambda = (2, 2); \mu = (); \nu = (4) & & & \lambda = (3, 3, 3); \mu = (1); \nu = (2). \end{array}$$

After decomposing into irreducible components, we can obtain a formula for general representable partitions:

**Corollary 7.7.** Let  $\nu$  be a representable partition. Then

$$\sum_{T \in \text{RPP}^{12}(\lambda/\mu; \nu)} \mathbf{x}^{\text{ircont}(T)} = (x_1 x_2)^M P_{n_0}(x_1, x_2) P_{n_1}(x_1, x_2) \cdots P_{n_r}(x_1, x_2), \quad (40)$$

where the numbers  $M, r, n_0, \dots, n_r$  are defined above:  $M = \#\nu$ ,  $r + 1$  is the number of irreducible components of  $\nu$  and  $n_0, n_1, \dots, n_r$  are their degrees.

*Proof of Corollary 7.7.* The restriction map

$$\text{RPP}^{12}(\lambda/\mu; \nu) \rightarrow \prod_{k=0}^r \text{RPP}^{12}\left(\lambda/\mu|_{[b_k, a_{k+1})}; \nu|_{\cap [b_k, a_{k+1})}\right)$$

is injective (since, as we know, the entries of a  $T \in \text{RPP}^{12}(\lambda/\mu; \nu)$  in any column outside of the irreducible components are uniquely determined) and surjective (as one can “glue” rpps together). Now use Theorem 7.5.  $\square$

For a 12-rpp  $T$ , the vectors  $\text{seplist}(T)$  and  $\text{ceq}(T)$  uniquely determine each other: if  $(\text{ceq}(T))_i = h$  then  $\text{seplist}(T)$  contains exactly  $\lambda_{i+1} - \mu_i - h$  entries equal to  $i$ , and this correspondence is one-to-one. Therefore, the polynomials on both sides of (40) are equal to  $Q_\alpha(x_1, x_2)$  where the vector  $\alpha$  is the one that corresponds to  $\nu$ .

Note that the polynomials  $P_n(x_1, x_2)$  are symmetric for all  $n$ . Since the question about the symmetry of  $\tilde{g}_{\lambda/\mu}$  can be reduced to the two-variable case, Corollary 7.7 gives an alternative proof of the symmetry of  $\tilde{g}_{\lambda/\mu}$ :

**Corollary 7.8.** The polynomials  $\tilde{g}_{\lambda/\mu} \in \mathbb{Z}[t_1, t_2, t_3, \dots][[x_1, x_2, x_3, \dots]]$  are symmetric.

Of course, our standing assumption that  $\lambda/\mu$  is connected can be lifted here, because in general,  $\tilde{g}_{\lambda/\mu}$  is the product of the analogous power series corresponding to the connected components of  $\lambda/\mu$ . So we have obtained a new proof of Theorem 3.3 in the case when  $\mathbf{k} = \mathbb{Z}[t_1, t_2, t_3, \dots]$  and when  $t_1, t_2, t_3, \dots$  are these indeterminates.

This also holds for any commutative ring  $\mathbf{k}$  and any  $t_1, t_2, t_3, \dots \in \mathbf{k}$ , since the case we have considered (where  $t_1, t_2, t_3, \dots$  are polynomial indeterminates over  $\mathbb{Z}$ ) is universal. Thus, we have reproven Theorem 3.3 in full generality.

Another application of Theorem 7.5 is a complete description of Bender-Knuth involutions on rpps.

**Corollary 7.9.** Let  $\nu$  be an irreducible partition. Then there is a unique map  $b : \text{RPP}^{12}(\lambda/\mu; \nu) \rightarrow \text{RPP}^{12}(\lambda/\mu; \nu)$  such that for all  $T \in \text{RPP}^{12}(\lambda/\mu; \nu)$  we have  $\text{ircont}(b(T)) = s_1 \cdot \text{ircont}(T)$ . This unique map  $b$  is an involution on  $\text{RPP}^{12}(\lambda/\mu; \nu)$ . So, for an irreducible partition  $\nu$  the corresponding Bender-Knuth involution exists and is unique.



Take any 12-rpp  $T \in \text{RPP}^{12}(\lambda/\mu; \nu)$  and recall that a 12-table  $\text{flip}(T)$  is obtained from  $T$  by simultaneously replacing all entries in 1-pure columns by 2 and all entries in 2-pure columns by 1.

**Corollary 7.10.** If  $\nu$  is an irreducible partition, then, no matter in which order one resolves conflicts in  $\text{flip}(T)$ , the resulting 12-rpp  $T'$  will be the same. The map  $T \mapsto T'$  is the unique Bender-Knuth involution on  $\text{RPP}^{12}(\lambda/\mu; \nu)$ .

*Proof of Corollary 7.10.* Conflict-resolution steps applied to  $\text{flip}(T)$  in any order eventually give an element of  $\text{RPP}^{12}(\lambda/\mu; \nu)$  with the desired ircont. There is only one such element. So we get a map  $\text{RPP}^{12}(\lambda/\mu; \nu) \rightarrow \text{RPP}^{12}(\lambda/\mu; \nu)$  that satisfies the assumptions of Corollary 7.9.  $\square$

Finally, notice that, for a general representable partition  $\nu$ , conflicts in a 12-table  $T$  with  $\text{seplist}(T) = \nu$  may only occur inside each irreducible component independently. Thus, we conclude the chain of corollaries by stating that our constructed involutions are canonical in the following sense:

**Corollary 7.11.** For a representable partition  $\nu$ , the map  $\mathbf{B} : \text{RPP}^{12}(\lambda/\mu; \nu) \rightarrow \text{RPP}^{12}(\lambda/\mu; \nu)$  is the unique involution that interchanges the number of 1-pure columns with the number of 2-pure columns inside each irreducible component.

### 7.3. The proof

Let  $\nu = (i_1, \dots, i_s)$  be an irreducible partition. We start with the following simple observation:

**Lemma 7.12.** Let  $T \in \text{RPP}^{12}(\lambda/\mu; \nu)$  for an irreducible partition  $\nu$ . Then any 1-pure column of  $T$  is to the left of any 2-pure column of  $T$ .

*Proof of Lemma 7.12.* Suppose it is false and we have a 1-pure column to the right of a 2-pure column. Among all pairs  $(a, b)$  such that column  $a$  is 2-pure and column  $b$  is 1-pure, and  $b > a$ , consider the one with smallest  $b - a$ . Then, the columns  $a + 1, \dots, b - 1$  must all be mixed. Therefore the set  $\text{NR}(T)$  contains  $\{(i_{p+1}, a + 1), (i_{p+2}, a + 2), \dots, (i_{p+b-1-a}, b - 1)\}$  for some  $p \in \mathbb{N}$ . And because  $a$  is 2-pure and  $b$  is 1-pure, each  $i_{p+k}$  (for  $k = 1, \dots, b - 1 - a$ ) must be  $\leq$  to the y-coordinate of the highest cell in column  $a$  and  $>$  than the y-coordinate of the lowest cell in column  $b$ . Thus, the support of any  $i_{p+k}$  for  $k = 1, \dots, b - 1 - a$  is a subset of  $[a + 1, b)$ , which contradicts the irreducibility of  $\nu$ .  $\square$

*Proof of Theorem 7.5.* We proceed by strong induction on the number of columns in  $\lambda/\mu$ . If the number of columns is 1, then the statement of Theorem 7.5 is obvious. Suppose that we have proven that for all skew partitions  $\widetilde{\lambda}/\mu$  with less

than  $\lambda_1$  columns and for all partitions  $\tilde{v}$  irreducible with respect to  $\widetilde{\lambda/\mu}$  and for all  $0 \leq \tilde{m} \leq \tilde{\lambda}_1 - \#\tilde{v}$ , there is exactly one 12-rpp  $\tilde{T}$  of shape  $\widetilde{\lambda/\mu}$  with exactly  $\tilde{m}$  1-pure columns, exactly  $\#\tilde{v}$  mixed columns and exactly  $(\tilde{\lambda}_1 - \#\tilde{v} - \tilde{m})$  2-pure columns. Now we want to prove the same for  $\lambda/\mu$ .

Take any 12-rpp  $T \in \text{RPP}^{12}(\lambda/\mu; \nu)$  with  $\text{seplist}(T) = \nu$  and with  $m$  1-pure columns for  $0 \leq m \leq \lambda_1 - \#\nu$ . Suppose first that  $m > 0$ . Then there is at least one 1-pure column in  $T$ . Let  $q \geq 0$  be such that the leftmost 1-pure column is column  $q + 1$ . Then by Lemma 7.12 the columns  $1, 2, \dots, q$  are mixed. If  $q > 0$  then the supports of  $i_1, i_2, \dots, i_q$  are all contained inside  $[1, q + 1)$  and we get a contradiction with the irreducibility of  $\nu$ . The only remaining case is that  $q = 0$  and the first column of  $T$  is 1-pure. Let  $\widetilde{\lambda/\mu}$  denote  $\lambda/\mu$  with the first column removed. Then  $\nu$  is obviously admissible but may not be irreducible with respect to  $\widetilde{\lambda/\mu}$ , because it may happen that  $\#\nu|_{\subseteq [2, b+1)} = b - 1$  for some  $b > 1$ . In this case we can remove these  $b - 1$  nonempty columns from  $\widetilde{\lambda/\mu}$  and remove the first  $b - 1$  entries from  $\nu$  to get an irreducible partition again<sup>49</sup>, to which we can apply the induction hypothesis. We are done with the case  $m > 0$ . If  $m < \lambda_1 - \#\nu$  then we can apply a mirrored argument to the last column, and it remains to note that the cases  $m > 0$  and  $m < \lambda_1 - \#\nu$  cover everything (since the irreducibility of  $\nu$  shows that  $\lambda_1 - \#\nu > 0$ ).

This inductive proof shows the uniqueness of the 12-rpp with desired properties. Its existence follows from a parallel argument, using the observation that the first  $b - 1$  columns of  $\widetilde{\lambda/\mu}$  can actually be filled in. This amounts to showing that for a representable  $\nu$ , the set  $\text{RPP}^{12}(\lambda/\mu; \nu)$  is non-empty in the case when  $\lambda_1 = \#\nu$  (so all columns of  $T \in \text{RPP}^{12}(\lambda/\mu; \nu)$  must be mixed). This is clear when there is just one column, and the general case easily follows by induction on the number of columns<sup>50</sup>.  $\square$

<sup>49</sup>This follows from Lemma 7.2 (c) (applied to the skew shape  $\widetilde{\lambda/\mu}$  and  $k = 1$ ). Here we are using the fact that if we apply Lemma 7.2 (a) to  $\widetilde{\lambda/\mu}$  instead of  $\lambda/\mu$ , then we get  $r = 1$  (because if  $r \geq 2$ , then  $\#\nu|_{\subseteq [a_2, b_2)} = \#\nu|_{\subseteq [a_2, b_2)}^{\widetilde{\lambda/\mu}} = b_2 - a_2$  in contradiction to the irreducibility of  $\lambda/\mu$ ).

<sup>50</sup>In more detail:

If we had  $1 \notin \text{supp}(\nu_1)$ , then we would have  $\text{supp}(\nu_1) \subseteq [2, \lambda_1 + 1)$ , and thus  $\text{supp}(\nu_j) \subseteq [2, \lambda_1 + 1)$  for every  $j$  (since  $\nu$  is weakly decreasing and since  $\text{supp}(\nu_1)$  is nonempty), which would lead to  $\nu|_{\subseteq [2, \lambda_1 + 1)} = \nu$  and thus  $\#\nu|_{\subseteq [2, \lambda_1 + 1)} = \#\nu = \lambda_1 > \lambda_1 + 1 - 2$ , contradicting the representability of  $\nu$ . Hence, we have  $1 \in \text{supp}(\nu_1)$ , so that we can fill the first column of  $\lambda/\mu$  with 1's and 2's in such a way that it becomes mixed and the 1's are displaced by 2's at level  $\nu_1$ . Now, let  $\widetilde{\lambda/\mu}$  be the skew partition  $\lambda/\mu$  without its first column, and  $\tilde{\nu}$  be the partition  $(\nu_2, \nu_3, \dots)$ . Then, the partition  $\tilde{\nu}$  is representable with respect to  $\widetilde{\lambda/\mu}$ . (Otherwise we would have  $\#\nu|_{\subseteq [2, b+1)}^{\widetilde{\lambda/\mu}} > b - 1$  for some  $b \geq 1$ , but then we would have  $\text{supp}(\nu_1) \subseteq [1, b + 1)$  as well and therefore  $\#\nu|_{\subseteq [1, b+1)} > (b - 1) + 1 = b$ , contradicting the representability of  $\lambda/\mu$ .) Thus we can fill in the entries in the cells of  $\widetilde{\lambda/\mu}$  by induction.

## References

- [BaaNip98] Franz Baader, Tobias Nipkow, *Term Rewriting and All That*, Cambridge University Press 1998.
- [BezCoq03] Marc Bezem, Thierry Coquand, *Newman's Lemma – a Case Study in Proof Automation and Geometric Logic*, Bulletin of the European Association for Theoretical Computer Science, February 2003.  
<http://www.ii.uib.no/~bezem/NL/>
- [FomGre06] Sergey Fomin, Curtis Greene, *Noncommutative Schur functions and their applications*, Discrete Mathematics 306 (2006) 1080–1096. doi:10.1016/S0012-365X(98)00140-X.
- [Fulton97] William Fulton, *Young Tableaux*, London Mathematical Society Student Texts 35, Cambridge University Press 1997.
- [GriRei15] Darij Grinberg, Victor Reiner, *Hopf algebras in Combinatorics*, August 25, 2015, arXiv:1409.8356v3.  
See also <http://web.mit.edu/~darij/www/algebra/HopfComb.pdf> for a version which is more frequently updated.
- [LamPyl07] Thomas Lam, Pavlo Pylyavskyy, *Combinatorial Hopf algebras and K-homology of Grassmanians*, arXiv:0705.2189v1. An updated version was later published in: International Mathematics Research Notices, Vol. 2007, Article ID rnm125, 48 pages. doi:10.1093/imrn/rnm125.
- [Macdon95] Ian G. Macdonald, *Symmetric Functions and Hall Polynomials*, 2nd edition, Oxford University Press 1995.
- [Stan99] Richard Stanley, *Enumerative Combinatorics, volume 2*, Cambridge University Press, 1999.
